# Supplementary material for: Correctly Communicating Software: Distributed, Asynchronous, and Beyond (extended version)
Source: arXiv:2402.09595 source file (2024-03-01)
Supplement: Supplementary file 2 [file app-meta.tex]

% !TeX root = ../../../../main.tex
\section{Meta-theoretical properties}
\label{app:meta_props}

%<*piBI:proofs>
\ifthesis{}We \else{}In this section we \fi first introduce auxiliary lemmas about (typed) spawn bindings and free/bound names of processes in \Cref{as:piBI:aux}.
We then present omitted proofs of subject congruence and subject reduction in \Cref{as:piBI:tp}.
After that we prove deadlock-freedom (\Cref{t:piBI:df}) in \Cref{as:piBI:df}, introducing a \emph{progress} lemma.
Finally, in \Cref{as:piBI:wn} we detail our proof of weak normalization.
%</piBI:proofs>

%<*piBI:proofs:aux>
\subsection{Spawn Bindings}

We will need the following properties for proving subject reduction, all shown by induction on spawn binding typing.

\begin{lemma}
    \label{l:piBI:typedSCtx}
    If $\spvar \from \Delta_1 \tobunch \Delta_2$, then $\spvar \from \bunchCtx{\Gamma}[\Delta_1] \tobunch \bunchCtx{\Gamma}[\Delta_2]$ for any bunched context $\bunchCtx{\Gamma}$.
\end{lemma}

\begin{lemma}
    \label{l:piBI:typedSCutNil}
    Suppose that $\spvar \from \bunchCtx{\Gamma_1}[x:A] \tobunch \Delta_2$ and $x \notin \dom(\spvar)$.
    Then $\Delta_2 = \bunchCtx{\Gamma_2}[x:A]$ for some~$\bunchCtx{\Gamma_2}$.
    Furthermore, for any~$\Delta$ we have $\spvar \from \bunchCtx{\Gamma_1}[\Delta] \tobunch \bunchCtx{\Gamma_2}[\Delta]$.
\end{lemma}

\begin{proof}
    We proceed by induction on $\spvar \from \bunchCtx{\Gamma_1}[x:A] \tobunch \Delta_2$.
    \begin{itemize}

        \item
            \textbf{(Case Rule~\ruleLabel{spawn-weaken})}
            If $\map{y -> \emptyset | {y \in \fn(\Delta)}} \from \bunchCtx{\Gamma}[\Delta; \Delta'] \tobunch \bunchCtx{\Gamma}[\Delta']$, then, from the assumption that $x \notin \dom(\spvar)$, we know that~$x$ does not occur in~$\Delta$.
            That means that~$x$ is either part of~$\Delta'$ or~$\bunchCtx{\Gamma}$.

            In either case, we can freely replace~$x:A$
            with an arbitrary bunch.

        \item
            \textbf{(Case Rule~\ruleLabel{spawn-contract})}
            Similar to the previous case.

        \item
            \textbf{(Case Rule~\ruleLabel{spawn-merge})}
            Suppose we have $(\spvar_1 \spmerge \spvar_2) \from \bunchCtx{\Gamma_0}[x:A] \tobunch \Delta_2$ with \mbox{$\spvar_1 \from \bunchCtx{\Gamma_0}[x:A] \tobunch \Delta_1$} for some intermediate bunch~$\Delta_1$.

            Since $x \notin \dom(\spvar_1 \spmerge \spvar_2)$, we know that $x \notin \dom(\spvar_1)$.
            Hence, ${\Delta_1 = \bunchCtx{\Gamma_1}[x:A]}$ by the IH, and we have $\spvar_1 \from \bunchCtx{\Gamma_1}[\Delta] \tobunch \bunchCtx{\Gamma_2}[\Delta]$ for any bunch~$\Delta$.

            Furthermore, $x \notin \restrOf(\spvar_1)$ (otherwise we would not be able to replace~$x:A$ with an arbitrary bunch~$\Delta$).
            Hence, $x \notin \dom(\spvar_2)$, and by the IH we have $\Delta_2 = \bunchCtx{\Gamma_2}[x:A]$ for some~$\bunchCtx{\Gamma_2}$, and $\spvar_2 \from \bunchCtx{\Gamma_1}[\Delta] \tobunch \bunchCtx{\Gamma_2}[\Delta]$ for any bunch~$\Delta$.
            The desired result then follows by using Rule~\ruleLabel{spawn-merge} again.
            \qedhere
    \end{itemize}
\end{proof}

\begin{lemma}
    \label{l:piBI:typedSCut}
    Suppose that $\spvar \from \Delta_1 \tobunch \Delta_2$ and $\spvar(x) = \{x_1,\ldots,x_n\}$.
    Then $\Delta_1 = \bunchCtx{\Gamma_1}[x:A]$ and $\Delta_2 = \bunchCtx{\Gamma_2}[x_1:A \mid \ldots \mid x_n:A]$, for some~$\bunchCtx{\Gamma_1}$ and~$\bunchCtx{\Gamma_2}$.
    Furthermore, for any bunch~$\Delta$ we have:
    \[
        (\spvar \setminus \{x\})
        \cup
        \map{y -> \{y_1, \dots, y_n\} | {y \in \fn(\Delta)}}
        \from
        \bunchCtx{\Gamma_1}[\Delta]
        \tobunch
        \bunchCtx[\big]{\Gamma_2}[\idx{\Delta}{1} \mid \ldots \mid \idx{\Delta}{n}]
    \]
\end{lemma}

\begin{proof}
    Similar to the previous lemma.
\end{proof}

\subsection{Names and Substitutions}

\begin{lemma}
    \label{l:piBI:fnIdent}
    If $\Delta \vdash P \typInf x:C$, then $\fn(P) = \fn(\Delta) \cup \{x\}$.
\end{lemma}

\begin{lemma}
    \label{l:piBI:fnTypedCut2}
    If $\pRes{x} ( P \| \pRes{y} ( Q \| R ) )$ is a well-typed process, then $x$ is shared either between~$P$ and~$Q$, or between $P$ and $R$, but not between all the three subprocesses, and $y$ is shared between~$Q$ and~$R$.
    That is, either $x \in \fn(P) \cap \fn(Q)$ and $x \notin \fn(R)$, or $x \in \fn(P) \cap \fn(R)$ and $x \notin \fn(Q)$.
    And in both cases we have $y \notin \fn(P)$
\end{lemma}

This lemma implies that whenever we have a typed process $\pRes{x} ( P \| \pRes{y} ( Q \| R ) )$, then one of the congruences Rule~\ruleLabel{cong-assoc-L} or~\ruleLabel{cong-assoc-R} applies.

\begin{lemma}
    \label{l:piBI:fnTypedCutSpawn}
    If $\pRes{x} ( P \| \pSpw[\spvar] ; Q )$ is a well-typed process, and $x \notin \spvar$, then $\fn(P) \cap \restrOf(\spvar) = \emptyset$.
\end{lemma}

Similarly to the previous lemma, this lemma implies that for a well-typed process of the form $\pRes{x} ( P \| \pSpw[\spvar] ; Q )$ either Rule~\ruleLabel{red-spawn} or Rule~\ruleLabel{red-spawn-R} applies.

\begin{lemma}
    \label{l:piBI:spawnTypedIndep}
    If $\pRes{x} ( \pSpw[\spvar_1] ; P \| \pSpw[\spvar_2] ; Q )$ is a well-typed process, then $\spvar_1$ and $\spvar_2$ are independent.
\end{lemma}

\begin{lemma}
    \label{l:piBI:injSubst}
    If $\Delta \vdash P \typInf x:C$ and $\theta$ is an injective substitution, then $\Delta\theta \vdash P\theta \typInf \theta(x):C$.
\end{lemma}
%</piBI:proofs:aux>

\subsection{Proof of subject reduction}
\label{app:subject_red:proof}

%<*piBI:proofs:tp>
\tPiBITp*

\begin{proof}[Proof (structural congruence)]
    We proceed by induction on $P \congr Q$, examining the possible typing derivations of $P$.

    \textbf{(Case Rule~\ruleLabel{cong-assoc-L})}
    This congruence states that the order of independent cuts does not matter.
    This corresponds to the following proof conversion:
    \begin{align*}
        & \begin{bussproof}
            \bussAssume{
                \Delta_1 \vdash P \typInf x:A
            }
            \bussAssume{
                \Delta_2 \vdash Q \typInf y:B
            }
            \bussAssume{
                \bunchCtx{\Gamma}[x:A \mid y:B] \vdash R \typInf z:C
            }
            \bussBin{
                \bunchCtx{\Gamma}[x:A \mid \Delta_2] \vdash \pRes{y} ( Q \|_y R ) \typInf z:C
            }
            \bussBin{
                \bunchCtx{\Gamma}[\Delta_1 \mid \Delta_2] \vdash \pRes{x} \big( P \|_x \pRes{y} ( Q \|_y R ) \big) \typInf z:C
            }
        \end{bussproof}
        \\
        & \congr
        \\
        & \begin{bussproof}
            \bussAssume{
                \Delta_2 \vdash Q \typInf y:B
            }
            \bussAssume{
                \Delta_1 \vdash P \typInf x:A
            }
            \bussAssume{
                \bunchCtx{\Gamma}[x:A \mid y:B] \vdash R \typInf z:C
            }
            \bussBin{
                \bunchCtx{\Gamma}[\Delta_1 \mid y:B] \vdash \pRes{x} ( P \|_x R) \typInf z:C
            }
            \bussBin{
                \bunchCtx{\Gamma}[\Delta_1 \mid \Delta_2] \vdash \pRes{y} \big( Q \|_y \pRes{x} ( P \|_x R ) \big) \typInf z:C
            }
        \end{bussproof}
    \end{align*}

    \textbf{(Case Rule~\ruleLabel{cong-assoc-R})}
    This congruence states that the order of subsequent cuts does not matter.
    This corresponds to the following proof conversion:
    \begin{align*}
        & \begin{bussproof}
            \bussAssume{
                \Delta \vdash P \typInf x:A
            }
            \bussAssume{
                \bunchCtx{\Gamma_1}[x:A] \vdash Q \typInf y:B
            }
            \bussAssume{
                \bunchCtx{\Gamma_2}[y:B] \vdash R \typInf z:C
            }
            \bussBin{
                \bunchCtx[\big]{\Gamma_2}[\bunchCtx{\Gamma_1}[x:A]] \vdash \pRes{y} ( Q \|_y R ) \typInf z:C
            }
            \bussBin{
                \bunchCtx[\big]{\Gamma_2}[\bunchCtx{\Gamma_1}[\Delta]] \vdash \pRes{x} \big( P \|_x \pRes{y} ( Q \|_y R ) \big) \typInf z:C
            }
        \end{bussproof}
        \\
        & \congr
        \\
        & \begin{bussproof}
            \bussAssume{
                \Delta \vdash P \typInf x:A
            }
            \bussAssume{
                \bunchCtx{\Gamma_1}[x:A] \vdash Q \typInf y:B
            }
            \bussBin{
                \bunchCtx{\Gamma_1}[\Delta] \vdash \pRes{x} ( P \|_x Q ) \typInf y:B
            }
            \bussAssume{
                \bunchCtx{\Gamma_2}[y:B] \vdash R \typInf z:C
            }
            \bussBin{
                \bunchCtx[\big]{\Gamma_2}[\bunchCtx{\Gamma_1}[\Delta]] \vdash \pRes{y} \big( \pRes{x} ( P \|_x Q ) \|_y R \big) \typInf z:C
            }
        \end{bussproof}
    \end{align*}

    \textbf{(Case Rule~\ruleLabel{cong-spawn-swap})}
    If two spawn bindings $\spvar$ and $\spvar'$ are independent, then they correspond to two independent applications of Rule~\ruleLabel{typ-struct} that can be commuted past each other.
    For example:
    \begin{align*}
        & \begin{bussproof}
            \bussAssume{
                \bunchCtx{\Gamma}[\aEmpty \mid \idx{\Delta}{1} ; \idx{\Delta}{2}] \vdash P \typInf z:C
            }
            \bussUn{
                \bunchCtx{\Gamma}[\aEmpty \mid \Delta] \vdash \pSpw[x->\{x_1,x_2\} | x \in \fn(\Delta)] ; P \typInf z:C
            }
            \bussUn{
                \bunchCtx{\Gamma}[\Delta' \mid \Delta] \vdash \pSpw[x->\emptyset | x \in \fn(\Delta')] ; \pSpw[x->\{x_1,x_2\} | x \in \fn(\Delta)] ; P \typInf z:C
            }
        \end{bussproof}
        \\
        & \congr
        \\
        & \begin{bussproof}
            \bussAssume{
                \bunchCtx{\Gamma}[\aEmpty \mid \idx{\Delta}{1} ; \idx{\Delta}{2}] \vdash P \typInf z:C
            }
            \bussUn{
                \bunchCtx{\Gamma}[\Delta' \mid \idx{\Delta}{1} ; \idx{\Delta}{2}] \vdash \pSpw[x->\emptyset | x \in \fn(\Delta')] ; P \typInf z:C
            }
            \bussUn{
                \bunchCtx{\Gamma}[\Delta' \mid \Delta] \vdash \pSpw[x->\{x_1,x_2\}] ; \pSpw[x->\emptyset | x \in \fn(\Delta')] ; P \typInf z:C
            }
        \end{bussproof}
    \end{align*}

    \textbf{(Closure under program contexts)}
     By the IH.
\end{proof}

\begin{proof}[Proof (reduction)]
    By induction on the reduction $P \redd Q$ and the typing derivation.
    The case Rule~\ruleLabel{red-cong} follows from the proof above and the IH.
    The case Rule~\ruleLabel{red-eval-ctx} for evaluation contexts of the forms $\evalCtx{K} = \pRes{x} ( \evalHole \| P )$ and $\evalCtx{K} = \pSpw[\spvar] ; \evalHole$ follows from the IH.

    \textbf{(Case Rule~\ruleLabel{red-close-wait})}
    It corresponds to the following reduction of proofs, or its additive variant:
    \begin{align*}
        & \begin{bussproof}
            \bussAx{
                \mEmpty \vdash \pClose x[] \typInf x:\mOne
            }
            \bussAssume{
                \bunchCtx{\Gamma}[\mEmpty] \vdash Q \typInf z:C
            }
            \bussUn{
                \bunchCtx{\Gamma}[x:\mOne] \vdash \pWait x() ; Q \typInf z:C
            }
            \bussBin{
                \bunchCtx{\Gamma}[\mEmpty] \vdash \pRes{x} ( \pClose x[] \|_x \pWait x() ; Q ) \typInf z:C
            }
        \end{bussproof}
        \\
        & \redd
        \\
        & \begin{bussproof}
            \bussAssume{
                \bunchCtx{\Gamma}[\mEmpty] \vdash Q \typInf z:C
            }
        \end{bussproof}
    \end{align*}

    \textbf{(Case Rule~\ruleLabel{red-wait-close})}
    Processes of the form $\pRes{x} \big( \pWait x() ; Q \|_x \pClose x[] \big)$ are not typable.

    \textbf{(Case Rule~\ruleLabel{red-send-recv})}
    It corresponds to the following reduction of proofs, or its additive version:
    \begin{align*}
        & \begin{bussproof}
            \bussAssume{
                \Delta_1 \vdash P_1 \typInf y:A
            }
            \bussAssume{
                \Delta_2 \vdash P_2 \typInf x:B
            }
            \bussBin{
                \Delta_1 , \Delta_2 \vdash \pOut* x[y] ; ( P_1 \| P_2 ) \typInf x:A \sep B
            }
            \bussAssume{
                \bunchCtx{\Gamma}[y:A , x:B] \vdash Q \typInf z:C
            }
            \bussUn{
                \bunchCtx{\Gamma}[x:A \sep B] \vdash \pIn x(y) ; Q \typInf z:C
            }
            \bussBin{
                \bunchCtx{\Gamma}[\Delta_1 , \Delta_2] \vdash \pRes{x} \big( \pOut* x[y] ; ( P_1 \| P_2 ) \|_x \pIn x(y) ; Q \big) \typInf z:C
            }
        \end{bussproof}
        \\
        & \redd
        \\
        & \begin{bussproof}
            \bussAssume{
                \Delta_2 \vdash P_2 \typInf x:B
            }
            \bussAssume{
                \Delta_1 \vdash P_1 \typInf y:A
            }
            \bussAssume{
                \bunchCtx{\Gamma}[y:A , x:B] \vdash Q \typInf z:C
            }
            \bussBin{
                \bunchCtx{\Gamma}[\Delta_1 , x:B] \vdash \pRes{y} ( P_1 \|_y Q ) \typInf z:C
            }
            \bussBin{
                \bunchCtx{\Gamma}[\Delta_1 , \Delta_2] \vdash \pRes{x} \big( P_2 \|_x \pRes{y} ( P_1 \|_y Q ) \big) \typInf z:C
            }
        \end{bussproof}
    \end{align*}

    \textbf{(Case Rule~\ruleLabel{red-recv-send})}
    It corresponds to the following reduction of proofs, or its additive version:
    \begin{align*}
        & \begin{bussproof}
            \bussAssume{
                \Delta, y:A \vdash Q \typInf x:B
            }
            \bussUn{
                \Delta \vdash \pIn x(y) ; Q \typInf x:A \wand B
            }
            \bussAssume{
                \Theta \vdash P_1 \typInf y:A
            }
            \bussAssume{
                \bunchCtx{\Gamma}[x:B] \vdash P_2 \typInf z:C
            }
            \bussBin{
                \bunchCtx{\Gamma}[\Theta , x:A \wand B] \vdash \pOut* x[y] ; ( P_1 \| P_2 ) \typInf z:C
            }
            \bussBin{
                \bunchCtx{\Gamma}[\Theta , \Delta] \vdash \pRes{x} \big( \pIn x(y) ; Q \|_x \pOut* x[y] ; ( P_1 \| P_2 ) \big) \typInf z:C
            }
        \end{bussproof}
        \\
        & \redd
        \\
        & \begin{bussproof}
            \bussAssume{
                \Theta \vdash P_1 \typInf y:A
            }
            \bussAssume{
                \Delta , y:A \vdash Q \typInf x:B
            }
            \bussBin{
                \Delta , \Theta \vdash \pRes{y} ( P_1 \|_y Q ) \typInf x:B
            }
            \bussAssume{
                \bunchCtx{\Gamma}[x:B] \vdash P_2 \typInf z:C
            }
            \bussBin{
                \bunchCtx{\Gamma}[\Delta , \Theta] \vdash \pRes{y} \big( \pRes{y} ( P_1 \|_y Q ) \|_x P_2 \big) \typInf z:C
            }
            \bussUn{
                \bunchCtx{\Gamma}[\Theta , \Delta] \vdash \pRes{y} \big( \pRes{y} ( P_1 \|_y Q ) \|_x P_2 \big) \typInf z:C
            }
        \end{bussproof}
    \end{align*}

    \textbf{(Case Rule~\ruleLabel{red-sel-bra})}
    It corresponds to the following reduction of proofs (w.l.o.g., for $\ell = \inl$):
    \begin{align*}
        & \begin{bussproof}
            \bussAssume{
                \Delta \vdash P \typInf x:A
            }
            \bussUn{
                \Delta \vdash \pSelL x ; P \typInf x:A \lor B
            }
            \bussAssume{
                \bunchCtx{\Gamma}[x:A] \vdash Q_1 \typInf z:C
            }
            \bussAssume{
                \bunchCtx{\Gamma}[x:B] \vdash Q_2 \typInf z:C
            }
            \bussBin{
                \bunchCtx{\Gamma}[x:A \lor B] \vdash \pBraLR x > {Q_1}{Q_2} \typInf z:C
            }
            \bussBin{
                \bunchCtx{\Gamma}[\Delta] \vdash \pRes{x} \big( \pSelL x ; P \|_x \pBraLR x > {Q_1}{Q_2} \big) \typInf z:C
            }
        \end{bussproof}
        \\
        & \redd
        \\
        & \begin{bussproof}
            \bussAssume{
                \Delta \vdash P \typInf x:A
            }
            \bussAssume{
                \bunchCtx{\Gamma}[x:A] \vdash Q_1 \typInf z:C
            }
            \bussBin{
                \bunchCtx{\Gamma}[\Delta] \vdash \pRes{x} ( P \| Q_1 ) \typInf z:C
            }
        \end{bussproof}
    \end{align*}

    \textbf{(Case Rule~\ruleLabel{red-fwd-L})}
    Follows from \Cref{l:piBI:injSubst}.
    \begin{align*}
        & \begin{bussproof}
            \bussAx{
                y:A \vdash \pFwd [x<>y] \typInf x:A
            }
            \bussAssume{
                \bunchCtx{\Gamma}[x:A] \vdash P \typInf z:C
            }
            \bussBin{
                \bunchCtx{\Gamma}[y:A] \vdash \pRes{x} ( \pFwd [x<>y] \|_x P ) \typInf z:C
            }
        \end{bussproof}
        \\
        & \redd
        \\
        & \begin{bussproof}
            \bussAssume{
                \bunchCtx{\Gamma}[y:A] \vdash P \{ y/x \} \typInf z:C
            }
        \end{bussproof}
    \end{align*}

    \textbf{(Case Rule~\ruleLabel{red-fwd-R})}
    Follows from \Cref{l:piBI:injSubst}.
    \begin{align*}
        & \begin{bussproof}
            \bussAssume{
                \Delta \vdash P \typInf x:A
            }
            \bussAx{
                x:A \vdash \pFwd [y<>x] \typInf y:A
            }
            \bussBin{
                \Delta \vdash \pRes{x} ( P \|_x \pFwd [y<>x] ) \typInf y:A
            }
        \end{bussproof}
        \\
        & \redd
        \\
        & \begin{bussproof}
            \bussAssume{
                \Delta \vdash P \{ y/x \} \typInf y:A
            }
        \end{bussproof}
    \end{align*}

    \textbf{(Case Rule~\ruleLabel{red-spawn})}
    By \Cref{l:piBI:typedSCut}, the derivation that we have is of the following shape:
    \begin{align*}
        & \begin{bussproof}
            
            \bussAssume{
                \Delta \vdash P \typInf x:A
            }
            \bussAssume{
                \bunchCtx{\Gamma_1}[x_1:A \mid \ldots \mid x_n:A] \vdash Q \typInf z:C
            }
            \bussAssume{
                \spvar \from \bunchCtx{\Gamma_2}[x:A] \tobunch \bunchCtx{\Gamma_1}[x_1:A \mid \ldots \mid x_n:A]
            }
            \bussBin{
                \bunchCtx{\Gamma_2}[x:A] \vdash \pSpw[\spvar] ; Q \typInf z:C
            }
            \bussBin{
                \bunchCtx{\Gamma_2}[\Delta] \vdash \pRes{x} ( P \|_x \pSpw[\spvar] ; Q ) \typInf z:C
            }
        \end{bussproof}
        \\
        & \redd
        \\
        & \begin{bussproof}

            \bussAssume{
                \vdots
            }
            \bussAssume{
                \idx{\Delta}{n} \vdash \idx{P}{n} \typInf x_n:A
            }
            \bussAssume{
                \bunchCtx{\Gamma_1}[x_1:A \mid \ldots \mid x_n:A] \vdash Q \typInf z:C
            }
            \bussBin{
                \bunchCtx{\Gamma_1}[x_1:A \mid \ldots \mid \idx{\Delta}{n}] \vdash \pRes{x_n} ( \idx{P}{n} \|_{x_n} Q ) \typInf z:C
            }
            \doubleLine
            \bussBin{
                \bunchCtx{\Gamma_1}[\idx{\Delta}{1} \mid \ldots \mid \idx{\Delta}{n}] \vdash \pRes{x_1} \big( \idx{P}{1} \|_{x_1} \ldots \pRes{x_n} ( \idx{P}{n} \|_{x_n} Q ) \ldots \big) \typInf z:C
            }
            \bussAssume{
                \text{(\Cref{l:piBI:typedSCut})}
            }
            \noLine
            \bussUn{
                \spvar' \from \bunchCtx{\Gamma_2}[\Delta] \tobunch \bunchCtx{\Gamma_1}[\idx{\Delta}{1} \mid \ldots \mid \idx{\Delta}{n}]
            }
            \bussBin{
                \bunchCtx{\Gamma_2}[\Delta] \vdash \pSpw[\spvar'] ; \pRes{x_1} \big( \idx{P}{1} \|_{x_1} \ldots \pRes{x_n} ( \idx{P}{n} \|_{x_n} Q ) \ldots \big) \typInf z:C
            }
        \end{bussproof}
    \end{align*}

    \textbf{(Case Rule~\ruleLabel{red-spawn-L})}
    This reduction corresponds to moving Rule~\ruleLabel{typ-struct} past a Rule~\ruleLabel{typ-cut}.
    Since $\pSpw[\spvar] ; P$ appears on the left side of the composition, we know that the application of Rule~\ruleLabel{typ-struct} was independent from $Q$ and from Rule~\ruleLabel{typ-cut}.
    The corresponding proof transformation is as follows:
    \begin{align*}
        & \begin{bussproof}
            \bussAssume{
                \Delta_1 \vdash P \typInf x:A
            }
            \bussAssume{
                \spvar \from \Delta_2 \tobunch \Delta_1
            }
            \bussBin{
                \Delta_2 \vdash \pSpw[\spvar] ; P \typInf x:A
            }
            \bussAssume{
                \bunchCtx{\Gamma}[x:A] \vdash Q \typInf z:C
            }
            \bussBin{
                \bunchCtx{\Gamma}[\Delta_2] \vdash \pRes{x} ( \pSpw[\spvar] ; P \|_x Q ) \typInf z:C
            }
        \end{bussproof}
        \\
        & \redd
        \\
        & \begin{bussproof}
            \bussAssume{
                \Delta_1 \vdash P \typInf x:A
            }
            \bussAssume{
                \bunchCtx{\Gamma}[x:A] \vdash Q \typInf z:C
            }
            \bussBin{
                \bunchCtx{\Gamma}[\Delta_1] \vdash \pRes{x} ( P \|_x Q ) \typInf z:C
            }
            \bussAssume{
                \text{(\Cref{l:piBI:typedSCtx})}
            }
            \noLine
            \bussUn{
                \spvar \from \bunchCtx{\Gamma}[\Delta_2] \tobunch \bunchCtx{\Gamma}[\Delta_1]
            }
            \bussBin{
                \bunchCtx{\Gamma}[\Delta_2] \vdash \pSpw[\spvar] ; \pRes{x} ( P \|_x Q ) \typInf z:C
            }
        \end{bussproof}
    \end{align*}

    \textbf{(Case Rule~\ruleLabel{red-spawn-R})}
    Similar to the previous case.
    Since $x \notin \spvar$ we know that the application of Rule~\ruleLabel{typ-struct} is independent of the Rule~\ruleLabel{typ-cut}.
    \begin{align*}
        & \begin{bussproof}
            \bussAssume{
                \Delta \vdash P \typInf x:A
            }
            \bussAssume{
                \bunchCtx{\Gamma_1}[x:A] \vdash Q \typInf z:C
            }
            \bussAssume{
                \spvar \from \bunchCtx{\Gamma_2}[x:A] \tobunch \bunchCtx{\Gamma_1}[x:A]
            }
            \bussBin{
                \bunchCtx{\Gamma_2}[x:A] \vdash \pSpw[\spvar] ; Q \typInf z:C
            }
            \bussBin{
                \bunchCtx{\Gamma_2}[\Delta] \vdash \pRes{x} ( P \|_x \pSpw[\spvar] ; Q ) \typInf z:C
            }
        \end{bussproof}
        \\
        & \redd
        \\
        & \begin{bussproof}
            \bussAssume{
                \Delta \vdash P \typInf x:A
            }
            \bussAssume{
                \bunchCtx{\Gamma_1}[x:A] \vdash Q \typInf z:C
            }
            \bussBin{
                \bunchCtx{\Gamma_1}[\Delta] \vdash \pRes{x} ( P \|_x Q ) \typInf z:C
            }
            \bussAssume{
                \text{(\Cref{l:piBI:typedSCutNil})}
            }
            \noLine
            \bussUn{
                \spvar \from \bunchCtx{\Gamma_2}[\Delta] \tobunch \bunchCtx{\Gamma_1}[\Delta]
            }
            \bussBin{
                \bunchCtx{\Gamma_2}[\Delta] \vdash \pSpw[\spvar] ; \pRes{x} ( P \|_x Q ) \typInf z:C
            }
        \end{bussproof}
    \end{align*}

    \textbf{(Case Rule~\ruleLabel{red-spawn-merge})}
    Directly using the rules for spawn prefix typing.
\end{proof}
%</piBI:proofs:tp>

\subsection{Proof of deadlock-freedom}
\label{app:dlfree:proof}

%<*piBI:proofs:df>
To prove deadlock-freedom, we first need to analyze when a process is \emph{not} stuck, i.e.\ when it can reduce.
We define the \emph{readiness} of a process, which is a means to syntactically determine whether a process can reduce.
This notion of readiness\footnote{In some literature this notion is referred to as ``liveness'', but we did not want to confuse it here with a more semantic notion of liveness.} is useful when implementing \piBI as, e.g., a programming language: a reduction can be derived by simply analyzing the syntax of a program.

To define readiness, we need to know which names can be used for a communication.
We define this as a process' set of \emph{active names}: free names used for communication prefixes not guarded by other communication prefixes.

\begin{definition}[Active Names]
    \label{d:piBI:an}
    Given a process $P$, we define the set of \emph{active names} of $P$, denoted $\an(P)$, as follows:
    \begin{align*}
        \an(\pClose x[])
        &\deq \{x\}
        &
        \an(\pRes{x} ( P \|_x Q ))
        &\deq (\an(P) \cup \an(Q)) \setminus \{x\}
        \\
        \an(\pWait x() ; P)
        &\deq \{x\}
        &
        \an(\pSpw[\spvar] ; P)
        &\deq \dom(\spvar) \cup (\an(P) \setminus \restrOf(\spvar))
        \\
        \an(\pOut* x[y] ; ( P \| Q ))
        &\deq \{x\}
        &
        \an(\pIn x(y) ; P)
        &\deq \{x\}
        \\
        \an(\pSelL{x} ; P)
        &\deq \an(\pSelR{x} ; P) \deq \{x\}
        &
        \an(\pFwd [x<>y])
        &\deq \{x,y\}
        \\
        \an(\pBraLR x > {P}{Q})
        &\deq \{x\}
    \end{align*}
\end{definition}

\begin{lemma}
    If $P \congr Q$ then $\an(P) = \an(Q)$.
\end{lemma}

\begin{proof}
    There are no rules of structural congruence that add or remove prefixes.
    Moreover, the only rule of structural congruence that affects names only affects \emph{bound} names, and active names are free by definition.
\end{proof}

\begin{definition}[Ready process]
    \label{def:ready}
    A process $P$ is \emph{ready}, denoted $\ready(P)$, if it is expected to reduce.
    Formally, the $\ready$ predicate is defined by the following rules:
    \begin{mathpar}
        \begin{bussproof}[rdy-spawn]
            \bussAssume{
                \ready(Q)
            }
            \bussUn{
                \ready(\pSpw[\spvar] ; Q)
            }
        \end{bussproof}
        \and
        \begin{bussproof}[rdy-merge]
            \bussAx{
                \ready(\pSpw[\spvar] ; \pSpw[\spvar'] ; Q)
            }
        \end{bussproof}
        \and
        \begin{bussproof}[rdy-cong]
            \bussAssume{
                \ready(Q)
            }
            \bussAssume{
                P \congr Q
            }
            \bussBin{
                \ready(P)
            }
        \end{bussproof}
        \and
        \begin{bussproof}[rdy-an]
            \bussAssume{
                x \in \an(P) \cap \an(Q)
            }
            \bussUn{
                \ready(\pRes{x} ( P \|_x Q ))
            }
        \end{bussproof}
        \and
        \begin{bussproof}[rdy-par]
            \bussAssume{
                \ready(P) \lor \ready(Q)
            }
            \bussUn{
                \ready(\pRes{x} ( P \|_x Q ))
            }
        \end{bussproof}
        \and
        \begin{bussproof}[rdy-spawn-cut]
            \bussAx{
                \ready(\pRes{x} ( \pSpw[\spvar] ; P \|_x Q ))
            }
        \end{bussproof}
        \and
        \begin{bussproof}[rdy-cut-spawn]
            \bussAx{
                \ready(\pRes{x} ( P \|_x \pSpw[\spvar] ; Q ))
            }
        \end{bussproof}
        \and
        \begin{bussproof}[rdy-fwd-L]
            \bussAx{
                \ready(\pRes{x} ( \pFwd [x<>y] \|_x Q ))
            }
        \end{bussproof}
        \and
        \begin{bussproof}[rdy-fwd-R]
            \bussAx{
                \ready(\pRes{x} ( P \|_x \pFwd [x<>y] ))
            }
        \end{bussproof}
    \end{mathpar}
\end{definition}

The following then assures that well-typed, ready processes can reduce:

\begin{lemma}[Progress]
    \label{t:piBI:progress}
    Suppose given a process $P$ such that $\Delta \vdash P \typInf z:C$ and $\ready(P)$.
    Then, there exists a process $S$ such that $P \redd S$.
\end{lemma}

\begin{proof}
    By induction on the derivation of $\ready(P)$.
    \begin{itemize}
        \item
            \textbf{(Case $P = \pSpw[\spvar] ; Q$ and $\ready(Q)$)}
            By the IH, there exists $S'$ such that $Q \redd S'$.
            By Rule~\ruleLabel{red-eval-ctx}, $P \redd \pSpw[\spvar] ; S'$.

        \item
            \textbf{(Case $P = \pSpw[\spvar] ; \pSpw[\spvar'] ; Q$)}
            By Rule~\ruleLabel{red-spawn-merge}, $P \redd \pSpw[\spvar \spmerge \spvar'] ; Q$.

        \item
            \textbf{(Case $P \congr Q$ and $\ready(Q)$)}
            By the IH, there exists $S$ such that $Q \redd S$.
            By Rule~\ruleLabel{red-cong}, $P \redd S$.

        \item
            \textbf{(Case $P = \pRes{x} ( Q \| R )$ and $x \in \an(Q) \cap \an(R)$)}
            We have $\Delta = \bunchCtx{\Gamma}[\Delta']$ where $\Delta' \vdash Q \typInf x:A$ and $\bunchCtx{\Gamma}[x:A] \vdash R \typInf z:C$.
            Since $x \in \an(Q) \cap \an(R)$, there is an unguarded prefix with subject $x$ in both $Q$ and $R$.
            Being unguarded, the prefix in $Q$ appears inside a sequence of $n$ cuts and spawns.
            Similarly, the prefix in $R$ appears inside a sequence of $m$ cuts and spawns.
            By induction on $n$ and $m$, we show that there exists a process $S$ such that $P \redd S$.
            \begin{itemize}
                \item
                    If $n = 0$ and $m = 0$, the analysis depends on whether $Q = \pFwd [x<>y]$ or $R = \pFwd [y<>x]$, or neither.
                    If so, this case is analogous the appropriate of the latter two cases of this proof.

                    Otherwise, neither $Q$ nor $R$ is a forwarder.
                    In that case, $Q$ is typable with a right rule for send, receive, selection, or branching on $x$, depending on the type~$A$.
                    Similarly, $R$ is typable with a dual left rule on $x$.
                    Suppose, as a representative example, that $A = B_1 \sep B_2$.
                    Then, $Q$ is typable with Rule~\ruleLabel{typ-sep-R}, i.e., \mbox{$Q = \pOut* x[y] ; ( Q_1 \| Q_2 )$}.
                    Similarly, $R$ is typable with Rule~\ruleLabel{typ-sep-L}, i.e., $R = \pIn x(y') ; R'$.
                    Then $P = \pRes{x} \big( \pOut* x[y] ; ( Q_1 \| Q_2 ) \| \pIn x(y') ; R \big)$.
                    Let $S \deq \pRes{x} \big( Q_2 \|_x \pRes{y} ( Q_1 \|_y R' \{ y/y' \} ) \big)$.
                    By Rule~\ruleLabel{red-send-recv}, $P \redd S$.

                \item
                    If $n = n' + 1$, then the analysis depends on whether the outermost construct in $Q$ is a cut or a spawn.
                    We thus consider these two cases:
                    \begin{itemize}
                        \item
                            If the outermost construct is a cut, then $P = \pRes{x} \big( \pRes{w} ( Q_1 \|_w Q_2 ) \|_x R )$.
                            The prefix on $x$ appears in $Q_2$, under a sequence of $n'$ sequence of and spawns.
                            Since $x \in \fn(\pRes{w} ( Q_1 \|_w Q_2 ))$, we know $w \neq x$.
                            This means that $x \notin \fn(Q_1)$.
                            Hence, by Rule~\ruleLabel{cong-assoc-R}, $P \congr \pRes{w} \big( Q_1 \|_w \pRes{x} ( Q_2 \|_x R ) \big)$.
                            By the IH, there exists $S'$ such that $\pRes{x} ( Q_2 \|_x R ) \redd S'$.
                            Let $S = \pRes{w} ( Q_1 \|_w S' )$.
                            Then, by Rules~\ruleLabel{red-eval-ctx} and~\ruleLabel{red-cong}, $P \redd S$.

                        \item
                            If the outermost construct is a spawn, then $Q = \pSpw[\spvar] ; Q'$ and the proof follows as in the case where $P = \pRes{x} ( \pSpw[\spvar] ; Q \|_x R )$.
                    \end{itemize}

                \item
                    If $m = m' + 1$, the analysis is analogous to the case above.
            \end{itemize}

        \item
            \textbf{(Case $P = \pRes{x} ( Q \|_x R )$ and $\ready(Q)$ or $\ready(R)$)}
            W.l.o.g., assume $\ready(Q)$.
            By the IH, there exists $S'$ such that $Q \redd S'$.
            By Rule~\ruleLabel{red-eval-ctx}, $P \redd \pRes{x} ( S' \| R )$.

        \item
            \textbf{(Case $P = \pRes{x} ( \pSpw[\spvar] ; Q \| R )$)}
            By well-typedness, $x \notin \spvar$.
            Hence, by Rule~\ruleLabel{red-spawn-L},
            \[
                P \redd \pSpw[\spvar] ; \pRes{x} ( Q \|_x R ).
            \]

        \item
            \textbf{(Case $P = \pRes{x} ( Q \|_x \pSpw[\spvar] ; R )$)}
            The analysis depends on wheter $x \in \spvar$ or not, so we consider two cases:
            \begin{itemize}
                \item
                    If $x \in \spvar$, then $\spvar(x) = \{x_1, \ldots, x_n\}$.
                    Let
                    \[
                        \spvar' = (\spvar \setminus \{x\}) \cup \map{w->\{w_1, \ldots, w_n\} | w \in (\fn(Q) \setminus \{x\})}
                    \]
                    and $S = \pSpw[\spvar'] ; \pRes{x_1} \big( \idx{Q}{1} \|_{x_1} \ldots \pRes{x_n} ( \idx{Q}{n} \|_{x_n} R ) \ldots \big)$.
                    By Rule~\ruleLabel{red-spawn}, $P \redd S$.

                \item
                    If $x \notin \spvar$, by Rule~\ruleLabel{red-spawn-R}, $P \redd \pSpw[\spvar] ; \pRes{x} ( Q \|_x R )$.
            \end{itemize}

        \item
            \textbf{(Case $P = \pRes{x} ( \pFwd[x<>y] \|_x Q )$)}
            By Rule~\ruleLabel{red-fwd-L}, $P \redd Q \{ y/x \}$.

        \item
            \textbf{(Case $P = \pRes{x} ( Q \|_x \pFwd[y<>x] )$)}
            By Rule~\ruleLabel{red-fwd-R}, $P \redd Q \{ y/x \}$.
            \qedhere
    \end{itemize}
\end{proof}

\tPiBIDf*

\begin{proof}
    If the process $P$ is ready, then the result follows from \Cref{t:piBI:progress}.
    Otherwise, towards a contradiction, assume $P \not\congr \pOut z[]$ and $P \not\congr \pSpw[\emptyset] ; \pOut z[]$.
    W.l.o.g., assume $P$ is not prefixed by an empty spawn.
    Since $\Sigma$ contains no names, and $P$ is not an empty send on $z$, the only possibility is that $P$ is a cut: $P \congr \pRes{x} ( Q \|_x R )$.
    There are several possibilities for $Q$ and $R$: they can be communications on $x$, they can be spawn prefixes with only $x$ in the domain, they can be cuts, or they can be forwarders on $x$.
    \begin{itemize}

        \item
            \textbf{(Case $Q$ or $R$ is a spawn prefix with only $x$ in the domain)}
            By definition, $P$ is ready: a contradiction.

        \item
            \textbf{(Case $Q$ or $R$ is a forwarder on $x$)}
            By definition, $P$ is ready: a contradiction.

        \item
            \textbf{(Case $Q$ is a communication on $x$)}
            By typability, $x$ must be free in $R$, so $R$ must contain an action on $x$: a spawn prefix with $x$ in the domain, a forwarder on $x$, or a communication on $x$.
            If $x \in \an(R)$, then $x \in \an(Q) \cap \an(R)$, so $P$ is ready by definition: a contradiction.
            Otherwise, there is a name $y$ such that the action on $x$ in $R$ is guarded by a spawn prefix with $y$ in the domain or by a communication prefix on $y$.
            Either way, there must be a cut on $y$ in $R$, i.e., $R \congr \pRes{y} ( R_1 \|_y R_2 )$.
            We show by induction on the structures of $R_1$ and $R_2$ that $R$ is ready.
            \begin{itemize}

                \item
                    \textbf{(Case $R_2$ is a spawn with $y$ in the domain)}
                    Then $R$ is ready by definition.

                \item
                    \textbf{(Case $R_1$ or $R_2$ is a forwarder on $x$)}
                    Then $R$ is ready by definition.

                \item
                    \textbf{(Case $R_1$ is a communication prefix on $y$)}
                    The analysis depends on whether $y \in \an(R_2)$.
                    If so, $R$ is ready by definition: a contradiction.
                    Otherwise, there is a name $z$ such that the action on $y$ in $R_2$ is guarded by a spawn prefix with $z$ in the domain or by a communication prefix on $z$.
                    Either way, there must be a cut on $z$ in~$R_2$, i.e., $R_2 \congr \pRes{z} ( R'_2 \|_z R''_2 )$.
                    By the IH, $R'_2$ or $R''_2$ is ready, so $R_2$ is ready by definition.
                    Hence, $R$ is ready by definition.

                \item
                    \textbf{(Case $R_2$ is a communication prefix on $y$)}
                    This case is analogous to the previous case.

                \item
                    \textbf{(Case $R_1$ or $R_2$ is a cut)}
                    Then, by the IH, $R_1$ or $R_2$ is ready, so $R$ is ready by definition.
            \end{itemize}
            Since $R$ is ready, also $P$ is ready: a contradiction.

        \item
            \textbf{(Case $R$ is a communication prefix on $x$)}
            This case is analogous to the previous case.

    \end{itemize}
    In each case, the assumption that $P$ is not ready is contradicted, so $P \congr \pClose z[]$ or $P \congr \pSpw[\emptyset] ; \pClose z[]$.
\end{proof}
%</piBI:proofs:df>

\subsection{Weak normalization}
\label{appendix:sec:wn}

%<*piBI:proofs:wn>
Recall our normalization strategy:
If a process can perform a communication reduction or a forwarder reduction, then we do exactly that reduction.
If a process can only perform a reduction that involves a spawn prefix, then we
\begin{enumerate}
    \item
        select an (active) spawn prefix with the least depth;
    \item
        perform the spawn reduction;
    \item
        propagate the newly created spawn prefix to the very top-level, merging it with other spawn prefixes along the way.
\end{enumerate}

We will show that this reduction strategy terminates, by assigning a particular lexicographical measure to the processes and showing that our strategy strictly reduces this measure.
This measure counts the number of communication prefixes in a process at a given depth, where depth is determined by spawn prefixes.
Let us make this precise.

For a process $P$ we consider its \emph{skeleton} $\skelOf(P)$, which is a finite map assigning to each number $n$ the amount of communication prefixes at depth $n$ and above.
Since processes are finite, each communication prefix occurs at a finite depth.
That means that $\skelOf(P)(k) = 0$ for any $k$ greater than the maximal depth of the process.
Formally, we define skeletons as follows.

\begin{definition}[Skeleton]
    A function $\skel \from \mbb{N} \to \mbb{N}$ is a \emph{skeleton of depth~$k$}, if $\forall i>k.~ \skel(i) = 0$.

    We define $\Skel_k$ as the set of all skeletons of depth~$k$.
    Moreover, we define $\Skel \deq \bigcup_{k\in\mbb{N}} \Skel_k$ and equip it with the strict quasi-order $\skelLt$ such that
    \[
        \skel_1 \skelLt \skel_2
        \iff
        \exists j.~ \big(
            \skel_1(j) < \skel_2(j)
            \land
            \forall i>j.~ \skel_1(i) = \skel_2(i)
        \big)
    \]
    We also define $\skel_1 \skelLe \skel_2 \deq (\skel_1 = \skel_2 \lor \skel_1 \skelLt \skel_2)$.
\end{definition}

The following lemmas allow us to do well-founded recursion on skeletons.

\begin{lemma}
    \label{l:piBI:skelLtPresk}
    If $\skel_2 \in \Skel_k$ and $\skel_2 \skelGt \skel_1$ then $\skel_1 \in \Skel_k$.
\end{lemma}

\begin{proof}
    From $\skel_2 \skelGt \skel_1$ we get some~$j$ such that $\skel_1(j) < \skel_2(j)$ and $\forall i>j.~ \skel_1(i) = \skel_2(i)$.
    \begin{itemize}

        \item
            \textbf{(Case $j \leq k$)}
            Then $\forall i>k.~ \skel_1(i) = \skel_2(i) = 0$ which proves $\skel_1 \in \Skel_k$.

        \item
            \textbf{(Case $j > k$)}
            This is impossible as we would have $\skel_1(j) < \skel_2(j) = 0$.
            \qedhere
    \end{itemize}
\end{proof}

\begin{lemma}
    \label{l:piBI:skelkWf}
    $(\Skel_k, \skelLt)$ is well-founded.
\end{lemma}

\begin{proof}
    Towards a contradiction, assume $\skel_0 \skelGt \skel_1 \skelGt \dots$ is an infinite descending chain of $\Skel_k$.
    Let~$j_n$ be the witness for $\skel_n \skelGt \skel_{n+1}$, i.e., $\skel_n(j_n) > \skel_{n+1}(j_n)$ and $\forall i>j_n.~ \skel_n(i) = \skel_{n+1}(i)$.
    From $s_n, s_{n+1} \in \Skel_k$ we get $j_n < k$.
    Since there are finitely many natural numbers below~$k$, by the pigeonhole principle, the sequence $j_0, j_1, \dots$ contains at least one number that repeats infinitely often.
    Among the ones that do, pick the greatest to be~$m$.
    By definition, all the numbers larger than~$m$ appear finitely often in $j_0, j_1, \dots$ and so there is a position~$p$ such that~$\forall n\geq p.~ j_n \leq m$.
    We obtain that $\forall n \geq p.~ \skel_n(m) \geq \skel_{n+1}(m)$.
    Moreover, let $i_0 < i_1 < \dots$ be such that~$j_{i_0}, j_{i_1}, \dots$ consists of the infinite subsequence of the occurrences of~$m$ in $j_p, j_{p+1}, \dots$, i.e., $m = j_{i_0} = j_{i_1} = \dots$.
    We have $\skel_{i_0}(m) > \skel_{i_0+1}(m) \geq \dots \geq \skel_{i_1}(m) > \skel_{i_1+1}(m) \geq \dots$.
    We obtain that $\skel_{i_0}(m) > \skel_{i_1}(m) > \dots$ is an infinite descending chain of~$\mbb{N}$, which is a contradiction.
\end{proof}

\begin{lemma}
    \label{l:piBI:skelWf}
    $(\Skel, \skelLt)$ is well-founded.
\end{lemma}

\begin{proof}
    Towards a contradiction, assume $\skel_0 \skelGt \skel_1 \skelGt \dots$ is an infinite descending chain of $\Skel$.
    Since $\skel_0 \in \Skel_k$ for some~$k$, by \Cref{l:piBI:skelLtPresk}, $\forall i.~ \skel_i \in \Skel_k$.
    Therefore we have an infinite descending chain of $\Skel_k$ which contradicts \Cref{l:piBI:skelkWf}.
\end{proof}

For a process $P$, its \emph{skeleton} $\skelOf(P)$ is a finite map assigning to each number $n$ the amount of communication prefixes at depth $n$.

\begin{definition}[Skeleton of~$P$]
    \label{d:piBI:skelOfP}
    Given $\skel, \skel_1,\skel_2\in\Skel$, we define:
    \begin{align*}
        \skelOne(i)
        &\deq \begin{cases}
            1 & \text{if $i=0$}
            \\
            0 & \text{otherwise}
        \end{cases}
        &
        (\skel_1 \skelPlus \skel_2)(i)
        &\deq \skel_1(i) + \skel_2(i)
        &
        (\skelShift{\skel})(i)
        &\deq \begin{cases}
            \skel(0) & \text{if $i=0$}
            \\
            \skel(i-1) & \text{if $i>0$}
        \end{cases}
    \end{align*}

    The \emph{skeleton of a process~$P$}, written $\skelOf(P)$, is then defined as:
    \begin{align*}
            \skelOf(P)
            &\deq \begin{cases}
                \skelOne & \text{if $P = \pFwd [x<>y]$ or $P = \pClose x[]$}
                \\
                \skelOne \skelPlus \skelOf(Q_1) \skelPlus \skelOf(Q_2) & \text{if $P = \pOut* x[y] ; ( Q_1 \| Q_2 )$ or $P = \pBraLR x > {Q_1}{Q_2}$}
                \\
                \skelOne \skelPlus \skelOf(Q) & \text{if $P = \pWait x() ; Q$ or $P = \pIn x(y) ; Q$ or $P = \pSel* x < \ell ; Q$}
                \\
                \skelOf(Q_1) \skelPlus \skelOf(Q_2) & \text{if $P = \pRes{x} ( Q_1 \|_x Q_2 )$}
                \\
                \skelShift{\skelOf(Q)} & \text{if $P = \pSpw[\spvar] ; Q$}
            \end{cases}
    \end{align*}

    Note that if $ \skel = \skelOf(P) $ then $\forall i.~ \skel(i) \geq \skel(i+1)$.
\end{definition}

For example:
\[
    \skelOf(\pRes{x} \big( \pClose x[] \|_x \pSpw[\spvar] ; \pRes{y} ( \pClose y[] \|_y \pSpw[\spvar'] ; \pWait x() ; \pWait y() ; \pClose k[] ) \big)) = \map{0 -> 5, 1 -> 4; 2 -> 3; \_ -> 0}.
\]

\paragraph{The measure.}

Recall from the main part of the \ifthesis{}chapter\else{}paper\fi, that when computing a measure associated to the process we have to take special care of the top-level spawn prefix.
We define the measure function $\mu$ as follows.
\[
    \mu(P) \deq \begin{cases}
        \skelOf(Q) & \text{if $P = \pSpw[\spvar] ; Q$}
        \\
        \skelOf(P) & \text{otherwise}
    \end{cases}
\]

\begin{lemma}
    \label{l:piBI:measureClosedCongr}
    If $P \congr Q$, then $\mu(P) = \mu(Q)$.
\end{lemma}

\begin{proof}
    None of the congruences can change whether the top-level construct is a spawn prefix.
    Furthermore, none of the congruences change depth of any communication prefixes.
\end{proof}

\begin{lemma}
    \label{l:piBI:measureCommReductions}
    The communication reductions strictly decrease the measure.
    That is, Rules~\ruleLabel{red-close-wait}, \ruleLabel{red-send-recv}, \ruleLabel{red-recv-send}, \ruleLabel{red-sel-bra}, \ruleLabel{red-fwd-L}, and~\ruleLabel{red-fwd-R} decrease the measure $\mu$, even when occurring under arbitrary evaluation contexts.

    Similarly, Rule~\ruleLabel{red-spawn-merge} strictly decreases the measure.
\end{lemma}

\begin{proof}
    Each of those rules reduce the amount of communication prefixes at a given depth, and, as such, decrease the skeleton of the process.
    The only thing that we need to note is the special spawn prefix condition on $\mu$ in Rules~\ruleLabel{red-close-wait}, \ruleLabel{red-fwd-L}, and~\ruleLabel{red-fwd-R}.
    In those cases, the reduction might introduce a spawn prefix in front of the process.
    However, in that case the measure $\mu$ will still strictly decrease.
\end{proof}

As we have seen, Rules~\ruleLabel{red-spawn}, \ruleLabel{red-spawn-L}, and~\ruleLabel{red-spawn-R} might temporarily increase the measure, but if we repeat them long enough then the measure will actually decrease.

\begin{lemma}
    \label{l:piBI:measureRhoReductions}
    Let $\evalCtx{K_0}$ be a non-empty evaluation context which may contain a $\pSpw[\spvar_0] ; \evalHole$ sub-context only at the top level.
    Let $\evalCtx{K_0}[\pSpw[\spvar] ; Q]$ be a process.
    In other words, $\pSpw[\spvar]$ is an active prefix spawn at the least depth in $\evalCtx{K_0}[\pSpw[\spvar] ; Q]$.
    Then there exists a spawn binding $\spvar'$, and an evaluation context $\evalCtx{K_1}$ which is free of $\pSpw[\spvar_1] ; \evalHole$ sub-contexts for any $\spvar_1$, such that
    \begin{align*}
        \evalCtx{K_0}[\pSpw[\spvar] ; Q] \redd* \pSpw[\spvar'] ; \evalCtx{K_1}[Q]
        && \text{and} &&
        \mu(\evalCtx{K_0}[\pSpw[\spvar] ; Q]) > \mu(\pSpw[\spvar'] ; \evalCtx{K_1}[Q]).
    \end{align*}
\end{lemma}

\begin{proof}
    We first show that the last condition follows from the previous ones.
    By definition, ${\mu(\pSpw[\spvar'] ; \evalCtx{K_1}[Q]) = \skelOf(\evalCtx{K_1}[Q])}$.
    We then consider two situations.
    If $\evalCtx{K_0}[\pSpw[\spvar] ; Q]$ does not have a spawn prefix at the top level, then
    \[
        \mu(\evalCtx{K_0}[\pSpw[\spvar] ; Q]) = \skelOf(\evalCtx{K_0}[\pSpw[\spvar] ; Q]) > \skelOf(\evalCtx{K_1}[Q]),
    \]
    as the later process has less spawn prefixes.
    On the other hand, if $\evalCtx{K_0}[\pSpw[\spvar] ; Q]$ begins with a spawn prefix at the top level, that prefix cannot be $\pSpw[\spvar]$ itself, as $\evalCtx{K_0}$ is non-empty.
    Then the process $\evalCtx{K_0}[\pSpw[\spvar] ; Q]$ is of the form $\pSpw[\spvar'] ; \evalCtx{K}[\pSpw[\spvar] ; Q]$, and we have
    \[
        \mu(\pSpw[\spvar'] ; \evalCtx{K}[\pSpw[\spvar] ; Q]) = \skelOf(\evalCtx{K}[\pSpw[\spvar] ; Q]) > \skelOf(\evalCtx{K_1}[Q]).
    \]

    Thus, we only need to find an adequate context $\evalCtx{K_1}$ and establish the reduction.
    We prove this by induction on the size of the evaluation context $\evalCtx{K_0}$.
    We do a case analysis on the ``tail'' of the evaluation context.

    \begin{itemize}

        \item
            \textbf{(Case $\evalCtx{K_0}$ is of the form ${\evalCtx{K'_0}[\pSpw[\spvar'] ; \evalHole]}$)}
            If $\evalCtx{K_0}$ contains the $\pSpw[\spvar'] ; \evalHole$, then by our assumption, it is on the top level.
            That means that $\evalCtx{K'_0}$ is empty.
            We then apply Rule~\ruleLabel{red-spawn-merge}:
            \[
                \pSpw[\spvar'] ; \pSpw[\spvar] ; Q \redd \pSpw[\spvar' \spmerge \spvar] ; Q.
            \]
            Then pick $\evalCtx{K_1}$ to be empty.

        \item
            \textbf{(Case ${\evalCtx{K_0}[\pSpw[\spvar] ; Q]}$ is of the form ${\evalCtx{K'_0}[\pRes{x} ( P \|_x \pSpw[x->x_1,x_2] ; Q )]}$)}
            We then have a reduction
            \[
                \evalCtx{K'_0}[\pRes{x} ( P \|_x \pSpw[x->x_1,x_2] ; Q )]
                \redd
                \evalCtx{K'_0}[
                    \pSpw[z->z_1, z_2] ;
                    \pRes{x_1} (
                        \idx{P}{1}
                        \|_{x_1} \pRes{x_2} ( \idx{P}{2} \|_{x_2} Q )
                    )
                ],
            \]
            if $\fn(P) = \{x, z\}$.

            If $\evalCtx{K'_0}$ is empty, then we are done.
            If it is not, then by the induction hypothesis we then have
            \begin{align*}
                & \evalCtx{K'_0}[
                    \pSpw[z->z_1, z_2] ;
                    \pRes{x_1} ( \idx{P}{1} \|_{x_1} \pRes{x_2} ( \idx{P}{2} \|_{x_2} Q ) )
                ]
                \\
                & \redd*
                \\
                & \pSpw[\spvar'] ;
                \evalCtx{K_1}[
                    \pRes{x_1} ( \idx{P}{1} \|_{x_1} \pRes{x_2} ( \idx{P}{2} \|_{x_2} Q ) )
                ],
            \end{align*}
            which we chain with the original application of Rule~\ruleLabel{red-spawn}.

            Other cases are handled similarly.
            \qedhere
    \end{itemize}
\end{proof}

\tPiBIWn*

\begin{proof}
    We give a normalization procedure as follows.
    Given a process $P$, we consider its possible reductions, and apply them in order that would decrease the measure $\mu$.
    We repeat this until we reach a normal form.
    Since the measure is strictly decreasing, this procedure will terminate by \Cref{l:piBI:skelWf}.

    Thanks to \Cref{l:piBI:measureClosedCongr} we can consider possible reductions of $P$ up to congruence.
    Let us consider which reductions can apply to $P$.
    \begin{itemize}

        \item
            \textbf{(Case Rules~\ruleLabel{red-spawn}, \ruleLabel{red-spawn-L}, \ruleLabel{red-spawn-R}, or~\ruleLabel{red-spawn-merge})}
            In that case we find a spawn prefix, involved with such a reduction, with the least depth.
            Then this spawn prefix will satisfy the conditions of \Cref{l:piBI:measureRhoReductions}, and we pull out this active prefix upfront, decreasing the measure.

        \item
            \textbf{(Case communication or forwarder reductions)}
            In that case we apply that exact reduction, which by \Cref{l:piBI:measureCommReductions} will decrease the measure.
            \qedhere
    \end{itemize}
\end{proof}
%</piBI:proofs:wn>

%%% Local Variables:
%%% mode: latex
%%% TeX-master: "../main"
%%% End:
