# Supplementary material for: Correctly Communicating Software: Distributed, Asynchronous, and Beyond (extended version)
Source: arXiv:2402.09595 source file (2024-03-01)
Supplement: Supplementary file 3 [file translation.tex]

% !TeX root = ../../../../main.tex
\section{Encoding the \alcalc}
\label{sec:appendix:translation}
The \alcalc type system follows the presentations of \alcalc by \citet{ohearn:2003} and \citet[Chapter 2]{pym:2002}, but we adjusted the elimination rule for additive units to match the corresponding rule for multiplicative units.
For reasons of space, we have omitted products and coproducts from \Cref{sec:translation}; these are present here.
\begin{figure}[t]
\adjustfigure
\input{figures/alcalc}
\caption{Typing system for \alcalc.}
\label{fig:alpha_lambda_typing_full}
\end{figure}
The type system is given in \cref{fig:alpha_lambda_typing_full}.
Note that the \ruleref{N-cut} is admissible (cf.\ \cite{ohearn:2003}).
\begin{figure}
\adjustfigure
\input{figures/alcalc_red}
\caption{Reduction rules for \alcalc.}
\label{fig:alcalc_red_rules_full}
\end{figure}
We consider call-by-name reduction strategy, the reduction relation for which is given in \cref{fig:alcalc_red_rules_full}.

The translation function $\bTrans_z(-)$ is defined by recursion on the typing derivation and is given in \cref{fig:translation_big,fig:translation_big_two}.
\begin{figure}
  \adjustfigure[\footnotesize]
  \centering
  \input{figures/alcalc_translation}
  \caption{Translation from \alcalc to \piBI (1/2).}
  \label{fig:translation_big}
\end{figure}
\begin{sidewaysfigure}
  \adjustfigure[\footnotesize]
  \centering
  \input{figures/alcalc_translation_two}
  \caption{Translation from \alcalc to \piBI (2/2).}
  \label{fig:translation_big_two}
\end{sidewaysfigure}

\subsection{Operational correspondence}

%<*alphalambda:oc:completeness>
We split the proof of completeness into two parts.
First, we show that if a term can reduce, then this reduction is matched by the translated process, and the resulting term and process diverge up to substitution lifting.

\begin{restatable}[Basic Completeness]{lemma}{lAlphalambdaBasicCompleteness}
    \label{l:alphalambda:basicCompleteness}
    Given $\Delta \vdash M : A$, if $M \aredd N$, then there exists $Q$ such that $\alTrans(M)z \redd* Q \subLift N$.
\end{restatable}

\begin{proof}
    By induction on the derivation of $M \aredd N$.
    There are six base cases:
    \begin{itemize}

        \item
            Rule~\ruleLabel{red-app-M}.
            We have $(\lam x . M)\ N \aredd M \{ N/x \}$.
            We then have
            \begin{align*}
                \alTrans({(\lam x. M)\ N})z
                &= \pRes{y} ( \pIn y(x) ; \alTrans(M)y \| \pOut* y[x] ; ( \alTrans(N)x \| \pFwd [z<>y] ) )
                \\
                &\redd \pRes{y} ( \pRes{x} ( \alTrans(N)x \| \alTrans(M)y ) \| \pFwd [z<>y] )
                \\
                &\redd \pRes{x} ( \alTrans(N)x \| \alTrans(M)z )
                \subLift M \{ N/x \}.
            \end{align*}

        \item
            Rule~\ruleLabel{red-app-A}.
            Analogous to Rule~\ruleLabel{red-app-M}.

        \item
            Rule~\ruleLabel{red-proj-pair}.
            We have $\pi_i(M_1,M_2) \aredd M_i$ for $i \in \{1,2\}$.
            Let $i' \in \{1,2\} \setminus \{i\}$.
            \begin{align*}
                \alTrans({\pi_i(M_1,M_2)})z
                &= \pRes{x_1} ( \pOut* {x_1}[x_2] ; ( \alTrans(M_2){x_2} \| \alTrans(M_1){x_1} ) \| \pIn x_1(x_2) ; \pSpw [x_{i'}->\emptyset] ; \pFwd [z<>x_i] )
                \\
                &\redd \pRes{x_1} ( \alTrans(M_1){x_1} \| \pRes{x_2} ( \alTrans(M_2){x_2} \| \pSpw [x_{i'}->\emptyset] ; \pFwd [z<>x_i] ) )
                \\
                &\redd \pSpw [z->\emptyset | z \in \fv(M_{i'})] ; \pRes{x_i} ( \alTrans(M_i){x_i} \| \pFwd [z<>x_i] )
                \\
                &\redd \pSpw [z->\emptyset | z \in \fv(M_{i'})] ; \alTrans(M_i)z
                \\
                &\subLift M_i
            \end{align*}

        \item
            Rule~\ruleLabel{red-let-unit-M}.
            We have $\tLet \mUnit = \mUnit \tIn M \aredd M$.
            \begin{align*}
                \alTrans(\tLet \mUnit = \mUnit \tIn M)z
                &= \pRes{x} ( \pClose x[] \| \pWait x() ; \alTrans(M)z )
                \\
                &\redd \alTrans(M)z
                \\
                &\subLift M
            \end{align*}

        \item
            Rule~\ruleLabel{red-let-pair}.
            We have $\tLet \<x,y\> = \<M_1, M_2\> \tIn N \aredd N \{ M_1/x,M_2/y \}$.
            \begin{align*}
                \alTrans({\tLet \<x,y\> = \<M_1, M_2\> \tIn N})z
                &= \pRes{x} ( \pOut* x[y] ; ( \alTrans(M_2)y \| \alTrans(M_1)x ) \| \pIn x(y) ; \alTrans(N)z )
                \\
                &\redd \pRes{x} ( \alTrans(M_1)x \| \pRes{y} ( \alTrans(M_2)y \| \alTrans(N)z ) )
                \\
                &\equiv \pRes{y} ( \alTrans(M_2)y \| \pRes{x} ( \alTrans(M_1)x \| \alTrans(N)z ) )
                \\
                &\subLift N \{ M_1/x,M_2/y \}
            \end{align*}

        \item
            Rule~\ruleLabel{red-case-sel}.
            We have, for ${i \in \{1,2\}}$, that
            \[
                \tCase \tSel_i(M) \tOf \{ 1(x_1) : N_1 , 2(x_2) : N_2 \} \aredd N_i \{ M/x_i \}.
            \]
            Expanding the translation:
            \begin{align*}
                & \alTrans({\tCase \tSel_i(M) \tOf \{ 1(x_1) : N_1 , 2(x_2) : N_2 \}})z
                \\
                &= \pRes{x_1} ( \alTrans({\tSel_i(M)}){x_1} \| \pBraLR x_1 > {\alTrans(N_1)z}{\pRes{x_2} ( \pFwd [x_2<>x_1] \| \alTrans(N_2)z )} )
            \end{align*}
            There are two cases for $i \in \{1,2\}$.
            \begin{itemize}

                \item
                    Case $i=1$.
                    \begin{align*}
                        & \pRes{x_1} ( \alTrans({\tSel_1(M)}){x_1} \| \pBraLR x_1 > {\alTrans(N_1)z}{\pRes{x_2} ( \pFwd [x_2<>x_1] \| \alTrans(N_2)z )} )
                        \\
                        &= \pRes{x_1} ( \pSelL {x_1} ; \alTrans(M){x_1} \| \pBraLR x_1 > {\alTrans(N_1)z}{\pRes{x_2} ( \pFwd [x_2<>x_1] \| \alTrans(N_2)z )} )
                        \\
                        &\redd \pRes{x_1} ( \alTrans(M){x_1} \| \alTrans(N_1)z )
                        \\
                        &\subLift N_1 \{ M/x_1 \}
                    \end{align*}

                \item
                    Case $i=2$.
                    \begin{align*}
                        & \pRes{x_1} ( \alTrans({\tSel_2(M)}){x_1} \| \pBraLR x_1 > {\alTrans(N_1)z}{\pRes{x_2} ( \pFwd [x_2<>x_1] \| \alTrans(N_2)z )} )
                        \\
                        &= \pRes{x_1} ( \pSelR {x_1} ; \alTrans(M){x_1} \| \pBraLR x_1 > {\alTrans(N_1)z}{\pRes{x_2} (\pFwd [x_2<>x_1] \| \alTrans(N_2)z )} )
                        \\
                        &\redd \pRes{x_1} ( \alTrans(M){x_1} \| \pRes{x_2} ( \pFwd [x_2<>x_1] \| \alTrans(N_2)z ) )
                        \\
                        &\redd \pRes{x_1} ( \alTrans(M){x_1} \| \alTrans(N_2)z \{ x_1/x_2 \} )
                        \\
                        &\equiv \pRes{x_2} ( \alTrans(M){x_2} \| \alTrans(N_2)z )
                        \\
                        &\subLift N_2 \{ M/x_2 \}
                    \end{align*}

        \end{itemize}

    \end{itemize}

    The inductive cases all concern the lifted reductions.
    Each case is analogous, so we only detail the arbitrarily chosen case of reduction lifting under $\lambda$-application.
    Assume $M \aredd M'$.
    We have $M\ N \aredd M'\ N$.
    By the IH, $\alTrans(M)y \redd* P \subLift M'$.
    Hence, assuming \mbox{$M' = M'' \{ N_1/x_1,\ldots,N_n/x_n \}$}, we have $P \congr \pRes{x_n} ( \alTrans(N_n){x_n} \| \ldots \pRes{x_1} ( \alTrans(N_1){x_1} \| \alTrans(M'')y ) \ldots )$.
    Moreover,
    \[
        M'\ N = (M'' \{ N_1/x_1,\ldots,N_n/x_n \})\ N = (M''\ N) \{ N_1/x_1,\ldots,N_n/x_n \}.
    \]
    We have the following:
    \begin{align*}
        \alTrans(M\ N)z
        &= \pRes{y} ( \alTrans(M)y \| \pIn y(w) ; \alTrans(N)z )
        \\
        &\redd* \pRes{y} ( \pRes{x_n} ( \alTrans(N_n){x_n} \| \ldots \pRes{x_1} ( \alTrans(N_1){x_1} \| \alTrans(M'')y ) \ldots ) \| \pIn y(w) ; \alTrans(N)z )
        \\
        &\equiv \pRes{x_n} ( \alTrans(N_n){x_n} \| \ldots \pRes{x_1} ( \alTrans(N_1){x_1} \| \pRes{y} ( \alTrans(M'')y \| \pIn y(w) ; \alTrans(N)z ) ) \ldots )
        \\
        &\subLift M'\ N
        \tag*{\qedhere}
    \end{align*}
\end{proof}

The statement of \Cref{l:alphalambda:basicCompleteness} cannot be chained to form a simulation diagram, since the premise does not start with the substitution relation as in the result.
The full version of completeness starts with a term and a process that are related via substitution lifting:

\tAlphalambdaCompleteness*

\begin{proof}
    Since $P \subLift M$, we can write the latter as $M' \{ N_1/x_1,\ldots,N_n/x_n \}$.
    We then consider two cases, depending on whether the reduction $M \aredd N$ already happens in $M'$, or whether this reduction is triggered by one of the substitutions.

    In the former case we already have a reduction $M' \aredd N'$ that is ``lifted'' to the reduction $M' \{ N_1/x_1,\ldots,N_n/x_n \} \aredd N' \{ N_1/x_1,\ldots,N_n/x_n \}$.
    We can then appeal directly to \Cref{l:alphalambda:basicCompleteness} to obtain a process $Q$ such that $\alTrans(M')z \redd* Q \subLift N'$.
    Then,
    \begin{align*}
        & \pRes{x_1} ( \alTrans(N_1)x_1 \| \ldots \pRes{x_n} ( \alTrans(N_n){x_n} \| \alTrans(M')z ) \dots )
        \\
        &\redd* \pRes{x_1} ( \alTrans(N_1)x_1 \| \ldots \pRes{x_n} ( \alTrans(N_n){x_n} \| Q ) \ldots ) \subLift N' \{ N_1/x_1,\ldots,N_n/x_n \}.
    \end{align*}

    In the second case, the reduction in the term is only enabled after some substitution $\{ N_i/x_i \}$ is performed.
    The idea is to reduce this to the first case, by explicitly performing the substitution $\{ N_i/x_i \}$ in the corresponding processes.

    If $\{ N_i/x_i \}$ is the substitution that enables the reduction $M' \{ N_1/x_1,\ldots,N_n/x_n \} \aredd N$, then the variable $x_i$ is located at a head position in the term $M'$.
    This means that in the translation, the corresponding process $\alTrans(x_i)c$ will not occur under an input/output prefix, which will allow us to eagerly perform the substitution by using the forwarder reduction, combined with the structural congruences and \ruleLabel{red-spawn-R}.

    Let us demonstrate what we mean by an example.
    Suppose that \mbox{$M = (x_1\ M'') \{ N_1/x_1,N_2/x_2 \}$} and $N_1 = \lam a . T$.
    Clearly, in this case the beta reduction is enabled only after the substitution.
    The corresponding substitution-lifted process can reduce as follows:
    \begin{align*}
        & \pRes{x_2} ( \alTrans(N_2){x_2} \| \pRes{x_1} ( \alTrans(N_1){x_1} \| \alTrans(x_1\ M'')z ) )
        \\
        &= \pRes{x_2} ( \alTrans(N_2){x_2} \| \pRes{x_1} ( \alTrans(N_1){x_1} \| \pRes{c} ( \alTrans(x_1)c \| \pOut* c[b] ; ( \alTrans(M'')b \| \pFwd [z<>c] ) ) ) )
        \\
        &= \pRes{x_2} ( \alTrans(N_2){x_2} \| \pRes{x_1} ( \alTrans(N_1){x_1} \| \pRes{c} ( \pFwd [c <> x_1] \| \pOut* c[b] ; ( \alTrans(M'')b \| \pFwd [z<>c] ) ) ) )
        \\
        &\redd \pRes{x_2} ( \alTrans(N_2){x_2} \| \pRes{x_1} ( \alTrans(N_1){x_1} \| \pOut* {x_1}[b] ; ( \alTrans(M'')b \| \pFwd [z<>x_1] ) ) )
        \\
        &= \pRes{x_2} ( \alTrans(N_2){x_2} \| \alTrans(N_1\ M'')z ) \subLift (N_1\ M'') \{ N_2/x_2 \}.
    \end{align*}
    The forwarder reduction in that sequence corresponds to explicitly performing the substitution $\{ N_1/x_1 \}$.
    After that we get a term $(N_1\ M'') \{ N_2/x_2 \}$ in which the reduction is enabled prior to the substitution, thus leaving us with the scenario from the case of this theorem.
\end{proof}
%</alphalambda:oc:completeness>

%<*alphalambda:oc:soundness>
\tAlphalambdaSoundness*

\begin{proof}
    By definition, $P \equiv \pSpw [\spvar_s] ; \ldots \pSpw [\spvar_1] ; \pRes{x_n} ( \alTrans(M_n){x_n} \| \ldots \pRes{x_1} ( \alTrans(M_1){x_1} \| \alTrans(M')z ) \ldots )$ where $M = M' \{ M_1/x_1,\ldots,M_n/x_n \} \{ \tilde{\spvar_1},\ldots,\tilde{\spvar_s} \}$.
    Let us consider possible reductions of $P$.
    First, each parallel subprocess of $P$ may reduce internally.
    Second, one of the subprocesses may be a forwarder, in which case a forwarder reduction is applicable.
    Third, one of the subprocesses may start with a spawn prefix, which can interact with the cuts.
    Note that no message-passing communication between the subprocesses of $P$ is possible, as follows from the definition of the translation.
    We discuss each possible case:
    \begin{itemize}

        \item
            $\alTrans(M_i){x_i}$ for $i \in [1,n]$ reduces internally, i.e., $\alTrans(M_i){x_i} \redd Q_i$.
            We apply induction on the derivation of $\Delta \vdash M : A$.
            Clearly, $\alTrans(M_i){x_i} \subLift M_i$.
            Since the typing derivation of $M_i$ is a sub-derivation of the typing derivation of $M$, the IH applies: there exist $N_i$ and $R_i$ such that $M_i \aredd^* N_i$ and $Q_i \redd* R_i \subLift N_i$.

            Let
            \[
                Q' \deq \pSpw [\spvar_s] ; \ldots \pSpw [\spvar_1] ; \pRes{x_n} ( \alTrans(M_n){x_n} \| \ldots \pRes{x_i} ( Q_i \| \ldots \pRes{x_1} ( \alTrans(M_1){x_1} \| \alTrans(M')z) \ldots ) \ldots );
            \]
            we have $P \redd Q'$.
            From $Q'$, all the reductions that were possible from $P$ are still possible.
            However, these reductions are all independent, so we postpone all but further reductions of $Q'$.
            Let
            \[
                R \deq \pSpw [\spvar_s] ; \ldots\pSpw [\spvar_1] ; \pRes{x_n} ( \alTrans(M_n){x_n} \| \ldots \pRes{x_i} ( R_i \| \ldots \pRes{x_1} ( \alTrans(M_1){x_1} \| \alTrans(M')z ) \ldots ) \ldots );
            \]
            we have $Q' \redd* R$.

            By definition,
            \[
                R_i \equiv \pSpw [\spvar'_t] ; \ldots \pSpw [\spvar'_1] ; \pRes{y_m} ( \alTrans(L_n){y_m} \| \ldots \pRes{y_1} ( \alTrans(L_1){y_1} \| \alTrans(N'_i){x_i} ) \ldots ),
            \]
            where $N_i = N'_i \{ L_1/y_1,\ldots,L_m/y_m \} \{ \tilde{\spvar'_1},\ldots,\tilde{\spvar'_t} \}$.
            Let
            \[
                M_0 = M' \{ M_1/x_1,\ldots,N_i/x_i,\ldots,M_n/x_n \};
            \]
            we have $M \aredd^* M_0$.
            Due to the shape of $R_i$, which includes substitutions, weakenings, and contractions in $N_i$, $R$ is not yet of a shape that we can relate to $M_0$.

            First, we have to move the spawn prefixes in $R_i$ to the sequence of spawn prefixes at the beginning of $R$.
            The procedure depends on whether there are $x_{i+1},\ldots,x_n$ that are weakened or contracted by the spawn prefixes in $R_i$.
            This is largely analogous to the latter cases of spawn prefixes commuting and interacting, so here we assume that no weakening or contraction takes place.
            By typability, none of the substitutions in $N_i$ touch the variable $x_i$, so we can commute the cuts in $R_i$ past the cut on $x_i$ in $R$.
            Let
            \begin{align*}
                R' &\deq
                \pSpw [\spvar_s] ; \ldots \pSpw [\spvar_1] ; \pSpw [\spvar'_t] ; \ldots \pSpw [\spvar'_1] ;
                \\
                &\hphantom{\deq} \quad \pRes{x_n} ( \alTrans(M_n){x_n} \| \ldots \pRes{y_m} ( \alTrans(L_m){y_m} \| \ldots \pRes{y_1} ( \alTrans(L_1){y_1} \| \pRes{x_i} ( \alTrans(N'_i){x_i}
                \\
                &\hphantom{\deq} \qquad {} \| \ldots \pRes{x_1} ( \alTrans(M_1){x_1} \| \alTrans(M')z ) \ldots ) ) \ldots ) \ldots )
            \end{align*}
            We have $R \redd* R'$.
            Moreover,
            \[
                M_0 = M' \{ M_1/x_1,\ldots,N'_i/x_i,L_1/y_1,\ldots,L_m/y_m,\ldots,M_n/x_n \} \{ \tilde{\spvar_1},\ldots,\tilde{\spvar_s},\tilde{\spvar'_1},\ldots,\tilde{\spvar'_t} \},
            \]
            and thus $R' \subLift M_0$.
            This proves the thesis.

        \item
            $\alTrans(M')z$ reduces internally.
            We apply induction on the derivation of $\Delta \vdash M : A$ (\ih1); there is a case per typing rule, although not all cases may yield a reduction in $P$.
            In each case, we additionally apply induction on the number $k$ of reductions from $P$ to~$Q$~(\ih2), i.e., $P \redd^k Q$.
            Depending on the shape of $P$, and relying on the independence of reductions, we then isolate $k'$ reductions $P \redd^{k'} Q'$ such that $Q' \subLift N'$ and $M \aredd N'$ (where $k'$ may be different in each case).
            We then have $Q' \redd^{k-k'} Q$, so it follows from~\ih2 that $N' \aredd^* N$ and $Q' \redd* R$ such that $R \subLift N$.

            Note that applications of \ih1 yield processes with spawn prefixes that need to be commuted past cuts to bring them to the front of the process, while some of them apply weakening or contraction when meeting certain cuts.
            We explain such procedures in the latter cases of this proof, so here we assume that \ih1 yields processes without spawn prefixes.

            \begin{itemize}

                \item
                    Rule~\ruleLabel{typ-id}.
                    We have $M' = y$ and $\alTrans(M')z = \pFwd [z<>y]$; no reductions are possible.

                \item
                    Rule~\ruleLabel{typ-cong}.
                    The thesis follows from \ih1 directly.

                \item
                    Rule~\ruleLabel{typ-weaken}.
                    We have $\alTrans(M')z = \pSpw [x->\emptyset | x \in \fv(\Delta')] ; \alTrans(M')z$.
                    There is only one possibility of reduction:
                    \[
                        \pSpw [x->\emptyset | x \in \fv(\Delta')] ; \alTrans(M')z \redd \pSpw [x->\emptyset | x \in \fv(\Delta')] ; Q'.
                    \]

                    By \ih1, there exist $L$ and $R'$ such that $M' \aredd^* L$ and $Q' \redd* R' \subLift L$.
                    Then
                    \[
                        R' \equiv \pRes{y_m} ( \alTrans(L_m){y_m} \| \ldots \pRes{y_1} ( \alTrans(L_1){y_1} \| \alTrans(L')z ) \ldots )
                    \]
                    and $L' = L' \{ L_1/y_1,\ldots,L_m/y_m \}$.

                    Let $R_0 \deq \pRes{x_n} ( \alTrans(M_n){x_n} \| \ldots \pRes{x_1} ( \alTrans(M_1){x_1} \| \pSpw [x->\emptyset | x \in \fv(\Delta')] ; R' ) )$; we have \mbox{$P \redd* R_0$}.
                    Also, let $M_0 \deq L' \{ L_1/y_1,\ldots,L_m/y_m,M_1/x_1,\ldots,M_n/x_n \}$; we have \mbox{$M \aredd^* M_0$}.

                    At this point, $R_0$ is not of appropriate shape to relate it to $M_0$ through substitution lifting, because the weakening spawn prefix is in the middle of the substitutions.
                    There are two possibilities for reduction here: the spawn interacts with one of the cuts on $x_i$, or the spawn commutes past them all.
                    The former is analogous to the case of a spawn prefix in $\alTrans(M')z$ interacting with a cut, which follows the current case.
                    In the latter case, let
                    \[
                        R \deq \pSpw [x->\emptyset | x \in \fv(\Delta')] ; \pRes{x_n} ( \alTrans(M_n){x_n} \| \ldots \pRes{x_1} ( \alTrans(M_1){x_1} \| R' ) ).
                    \]
                    Now, $R_0 \redd* R$ and $R \subLift M_0$, proving the thesis.

                \item
                    Rule~\ruleLabel{typ-contract}.
                    Analogous to Rule~\ruleLabel{typ-weaken}.

                \item
                    Rule~\ruleLabel{typ-wand-I}.
                    We have $M' = \lam x . M''$ and $\alTrans(M')z = \pIn z(x) ; \alTrans(M'')z$; no reductions are possible.

                \item
                    Rule~\ruleLabel{typ-impl-I}.
                    Analogous to Rule~\ruleLabel{typ-wand-I}.

                \item
                    Rule~\ruleLabel{typ-wand-E}.
                    We have $M' = L_1\ L_2$ and
                    \[
                        \alTrans(M')z = \pRes{x} ( \alTrans(L_1)x \| \pOut* x[y] ; ( \alTrans(L_2)y \| \pFwd [z<>x] ) ).
                    \]
                    There are three possible reductions: $\alTrans(L_1)x$ reduces internally, $\alTrans(L_1)x$ is prefixed by a spawn which commutes past the restriction on $x$, or the output on $x$ synchronizes with an input on $x$ in $\alTrans(L_1)x$.
                    \begin{itemize}

                        \item
                            $\alTrans(L_1)x$ reduces internally, i.e., $\alTrans(L_1)x \redd Q'$.
                            By \ih1, there exist $N$ and $R'$ such that $L_1 \aredd^* N$ and $Q' \redd* R' \subLift N$.
                            Then
                            \[
                                R' \equiv \pRes{y_m} ( \alTrans(N_m){y_m} \| \ldots \pRes{y_1} ( \alTrans(N_1){y_1} \| \alTrans(N')x ) \ldots )
                            \]
                            and $N = N' \{ N_1/y_1,\ldots,N_m/y_m \}$.
                            Let
                            \begin{align*}
                                R_0 &\deq
                                \pRes{x_n} ( \alTrans(M_n){x_n} \| \ldots \pRes{x_1} ( \alTrans(M_1){x_1} \| \pRes{x} ( R' \| \pOut* x[y] ; ( \alTrans(L_2)y \| \pFwd [z<>x] ) ) ) \ldots );
                            \end{align*}
                            we have $P \redd* R_0$.
                            Also, let
                            \begin{align*}
                                M_0 &\deq (N' \{ N_1/y_1,\ldots,N_m/y_m \}\ L_2) \{ M_1/x_1,\ldots,M_n/x_n \}
                                \\
                                &= (N'\ L_2) \{ N_1/y_1,\ldots,N_m/y_m,M_1/x_1,\ldots,M_n/x_n \}
                            \end{align*}
                            we have $M \aredd^* M_0$.
                            We have
                            \begin{align*}
                                R_0 &\equiv \pRes{x_n} ( \alTrans(M_n){x_n} \| \ldots \pRes{x_1} ( \alTrans(M_1){x_1} \| \pRes{y_m} ( \alTrans(N_m){y_m}
                                \\
                                &\hphantom{\equiv} \quad {} \| \ldots \pRes{y_1} ( \alTrans(N_1){y_1} \| \pRes{x} ( \alTrans(N')x \| \pOut* x[y] ; ( \alTrans(L_2)y \| \pFwd [z<>x] ) ) ) \ldots)
                                ) \ldots ),
                            \end{align*}
                            so $R_0 \subLift M_0$.
                            This proves the thesis.

                        \item
                            $\alTrans(L_1)x$ is prefixed by a spawn which commutes past the restriction on $x$.
                            This case is analogous to the case of a spawn prefix in $\alTrans(M')x$ commuting past cuts, which follows the current case.

                        \item
                            The output on $x$ synchronizes with an input on $x$ in $\alTrans(L_1)x$.
                            By typability, then $L_1 = \lam y . L'_1$ and $\alTrans(L_1)x = \pIn x(y) ; \alTrans(L'_1)x$.
                            Let
                            \[
                                Q'_0 \deq \pRes{x} ( \pRes{y} ( \alTrans(L_2)y \| \alTrans(L'_1)x ) \| \pFwd [z<>x] ).
                            \]
                            Then $\alTrans(M')x \redd Q'_0$.

                            From $Q'_0$, there may be similar reductions as from $\alTrans(M')x$, with an additional forwarder reduction possible.
                            All of these reductions are independent, so we postpone all but the forwarder reduction.
                            Let $Q'_1 \deq \pRes{y} ( \alTrans(L_2)y \| \alTrans(L'_1)z )$.
                            Then $Q'_0 \redd Q'_1$.

                            Let $Q' \deq \pRes{x_n} ( \alTrans(M_n){x_n} \| \ldots \pRes{x_1} ( \alTrans(M_1){x_1} \| Q'_1 ) )$; we have $P \redd^2 Q'$.
                            Also, let $M_0 \deq M'_1 \{ L_2/y,M_1/x_1,\ldots,M_n/x_n \}$; we have $M \aredd M_0$.
                            Since $Q' \redd^{k-2} Q$, the thesis then follows from \ih2.

                    \end{itemize}

                \item
                    Rule~\ruleLabel{typ-impl-E}.
                    Analogous to Rule~\ruleLabel{typ-wand-E}.

                \item
                    Rule~\ruleLabel{typ-emp-I}.
                    We have $M' = \mUnit$ and $\alTrans(M')z = \pClose z[]$; no reductions are possible.

                \item
                    Rule~\ruleLabel{typ-true-I}.
                    Analogous to Rule~\ruleLabel{typ-emp-I}.

                \item
                    Rule~\ruleLabel{typ-emp-E}.
                    We have $M' = \tLet \mUnit = L_1 \tIn L_2$ and
                    \[
                        \alTrans(M')z = \pRes{x} ( \alTrans(L_1)x \| \pWait x() ; \alTrans(L_2)z ).
                    \]
                    There are three possible reductions: $\alTrans(L_1)x$ reduces internally, $\alTrans(L_2)x$ is prefixed by a spawn which commutes past the restriction on $x$, or the empty input on $x$ synchronizes with an empty output on $x$ in $\alTrans(L_1)x$.
                    The former two sub-cases are analogous to the similar sub-cases in Rule~\ruleLabel{typ-wand-E}.
                    In the latter case, by typability, we have $L_1 = \mUnit$ and $\alTrans(L_1)x = \pClose x[]$.

                    Let $Q_0 \deq \alTrans(L_2)z$; we have $\alTrans(M')z \redd Q_0$.
                    Let
                    \[
                        Q' \deq \pRes{x_n} ( \alTrans(M_n){x_n} \| \ldots \pRes{x_1} ( \alTrans(M_1){x_1} \| Q_0 ) \ldots );
                    \]
                    we have $P \redd Q'$.

                    Let $M_0 \deq L_2 \{ M_1/x_1,\ldots,M_n/x_n \}$; we have $M \aredd M_0$ and $Q' \subLift M_0$.
                    Since $Q' \redd^{k-1} Q$, the thesis follows from \ih2.

                \item
                    Rule~\ruleLabel{typ-true-E}.
                    Analogous to Rule~\ruleLabel{typ-emp-E}.

                \item
                    Rule~\ruleLabel{typ-sep-I}.
                    We have $M' = \<L_1,L_2\>$ and $\alTrans(M')z = \pOut* z[y] ; ( \alTrans(L_1)y \| \alTrans(L_2)z )$; no reductions are possible.

                \item
                    Rule~\ruleLabel{typ-conj-I}.
                    Analogous to Rule~\ruleLabel{typ-sep-I}.

                \item
                    Rule~\ruleLabel{typ-sep-E}.
                    We have $M' = \tLet \<x,y\> = L_1 \tIn L_2$ and
                    \[
                        \alTrans(M')z = \pRes{y} ( \alTrans(L_1)y \| \pIn y(x) ; \alTrans(L_2)z ).
                    \]
                    There are three possible reductions: $\alTrans(L_1)y$ reduces internally, $\alTrans(L_1)y$ is prefixed by a spawn which commutes past the restriction on $y$, or the input on $y$ synchronizes with an output on $y$ in $\alTrans(L_1)y$.
                    The former two sub-cases are analogous to the similar sub-cases in Rule~\ruleLabel{typ-wand-E}.
                    In the latter case, by typability, we have $L_1 = \<K_1,K_2\>$ and $\alTrans(L_1)y = \pOut* y[x] ; ( \alTrans(K_1)x \| \alTrans(K_2)y )$.

                    Let $Q_0 \deq \pRes{y} ( \alTrans(K_2)y \| \pRes{x} ( \alTrans(K_1)x \| \alTrans(L_2)z ) )$; we have $\alTrans(M')z \redd Q_0$.
                    Let
                    \[
                        Q' \deq \pRes{x_n} ( \alTrans(M_n){x_n} \| \ldots \pRes{x_1} ( \alTrans(M_1){x_1} \| Q_0 ) \ldots );
                    \]
                    we have $P \redd Q'$.

                    Let $M_0 \deq L_2 \{ K_1/x,K_2/y,M_1/x_1,\ldots,M_n/x_n \}$; we have $M \aredd M_0$ and $Q' \subLift M_0$.
                    Since $Q' \redd^{k-1} Q$, the thesis follows from \ih2.

                \item
                    Rule~\ruleLabel{typ-conj-E}.
                    We have $M' = \pi_i L$ and
                    \[
                        \alTrans(M')z = \pRes{x_2} ( \alTrans(L){x_2} \| \pIn x_2(x_1) ; \pSpw [x_{i'}->\emptyset] ; \pFwd [z<>x_i] )
                    \]
                    for $i \in \{1,2\}$ and $i' \in \{1,2\} \setminus \{i\}$.
                    W.l.o.g., let $i = 1$ and $i' = 2$.
                    There are three possible reductions: $\alTrans(L){x_2}$ reduces internally, $\alTrans(L){x_2}$ is prefixed by a spawn which commutes past the restriction on $x_2$, or the input on $x_2$ synchronizes with an output on $x_2$ in $\alTrans(L){x_2}$.
                    The former two sub-cases are analogous to the similar sub-cases in Rule~\ruleLabel{typ-wand-E}.

                    In the latter case, by typability, we have $L = (L_1,L_2)$ and
                    \[
                        \alTrans(L){x_2} = \pOut* {x_2}[x_1] ; ( \alTrans(L_1){x_1} \| \alTrans(L_2){x_2} ).
                    \]
                    Let $Q_0 = \pRes{x_2} ( \alTrans(L_2){x_2} \| \pRes{x_1} ( \alTrans(L_1){x_1} \| \pSpw [x_2->\emptyset] ; \pFwd [z<>x_1] ) )$; we have $\alTrans(M')z \redd Q_0$.

                    From $Q_0$, there may be internal reductions of $\alTrans(L_2){x_2}$ or $\alTrans(L_1){x_1}$, a spawn prefix in $\alTrans(L_2){x_2}$ may commute past the restriction on $x_2$, a spawn prefix in $\alTrans(L_1){x_1}$ may commute past the restrictions on $x_1$ and $x_2$, and the spawn prefix $\pSpw [x_2->\emptyset]$ may commute past the restriction on $x_1$.
                    All these reductions are independent, so we postpone all but the commute of the spawn prefix $\pSpw [x_2->\emptyset]$.
                    Let
                    \[
                        Q_1 \deq \pRes{x_2} ( \alTrans(L_2){x_2} \| \pSpw [x_2->\emptyset] ; \pRes{x_1} ( \alTrans(L_1){x_1} \| \pFwd [z<>x_1] ) );
                    \]
                    we have $Q_0 \redd Q_1$.

                    From $Q_1$ we have the same possible reductions as from $Q_0$, except that there may also be weakening of $x_2$ due to the spawn prefix $\pSpw [x_2->\emptyset]$ interacting with the restriction on $x_2$.
                    Again, we postpone all but the latter reduction.
                    Let
                    \[
                        Q_2 \deq \pSpw [y->\emptyset | y \in \fv(L_2)] ; \pRes{x_1} ( \alTrans(L_1){x_1} \| \pFwd [z<>x_1] );
                    \]
                    we have $Q_1 \redd Q_2$.

                    From $Q_2$, we again have the reductions that were available from $Q_1$, but also the reduction of the forwarder $\pFwd [z<>x_1]$.
                    We postpone all but the latter.
                    Let
                    \[
                        Q_3 \deq \pSpw [y->\emptyset | y \in \fv(L_2)] ; \alTrans(L_1)z;
                    \]
                    we have $Q_2 \redd Q_3$.

                    Let $Q'_0 \deq \pRes{x_n} ( \alTrans(M_n){x_n} \| \ldots \pRes{x_1} ( \alTrans(M_1){x_1} \| Q_3 ) \ldots )$; we have $P \redd^4 Q'_0$.
                    Also, let $M_0 \deq L_1 \{ M_1/x_1,\ldots,M_n/x_n \}$, where the resources used by $L_2$ have been weakened.
                    At this point, $Q'_0$ is not of appropriate shape to relate it to $M_0$ through substitution lifting, because of the spawn prefix in $Q_3$.
                    There are two possibilities for reduction here: the spawn interacts with one of the cuts on $x_i$, or the spawn commutes past them all.
                    The former is analogous to the case of a spawn prefix in $\alTrans(M')z$ interacting with a cut, which follows the current case.
                    In the latter case, let
                    \[
                        Q' \deq \pSpw [y->\emptyset | y \in \fv(L_2)] ; \pRes{x_n} ( \alTrans(M_n){x_n} \| \ldots \pRes{x_1} ( \alTrans(M_1){x_1} \| \alTrans(L_1)z ) \ldots ).
                    \]
                    Now $Q'_0 \redd^n Q'$ and $Q' \subLift M_0$.

                    Since $Q' \redd^{k-4-n} Q$, the thesis follows from \ih2.

                \item
                    Rule~\ruleLabel{typ-disj-I}.
                    We have $M' = \tSel_i(N)$ for $i \in \{1,2\}$.
                    Depending on the value of $i$, $\alTrans(M')z$ is either $\pSelL {z} ; \alTrans(N)z$ or $\pSelR {z} ; \alTrans(N)z$.
                    Either way, no reductions are possible.

                \item
                    Rule~\ruleLabel{typ-disj-E}.
                    We have
                    \begin{align*}
                        M' &= \tCase N \tOf \{ 1(y_1) : L_1 , 2(y_2) : L_2 \}
                        \\
                        \alTrans(M')z &=
                        \pRes{y_1} ( \alTrans(N){y_1} \| \pBraLR y_1 > {\alTrans(L_1)z}{\pRes{y_2} ( \pFwd [y_2<>y_1] \| \alTrans(L_2)z )} ).
                    \end{align*}
                    There are three possible reductions: $\alTrans(N){y_1}$ reduces, $\alTrans(N){y_1}$ is prefixed by a spawn which commutes past the restriction on $y_1$, or the case on $y_1$ synchronizes with a select on $y_1$ in $\alTrans(N){y_1}$.
                    The former two sub-cases are analogous to the similar sub-cases in Rule~\ruleLabel{typ-wand-E}.

                    In the latter case, by typability, we have $N = \tSel_i(N')$ for $i \in \{1,2\}$.
                    The rest of the analysis depends on the value of $i$:
                    \begin{itemize}
                        \item
                            Case $i=1$.
                            We have $\alTrans(N){y_1} = \pSelL {y_1} ; \alTrans(N'){y_1}$.
                            Let $Q_0 \deq \pRes{y_1} ( \alTrans(N'){y_1} \| \alTrans(L_1)z )$; we have $\alTrans(M')z \redd Q_0$.
                            Let $Q' \deq \pRes{x_n} ( \alTrans(M_n){x_n} \| \ldots \pRes{x_1} ( \alTrans(M_1){x_1} \| Q_0 ) )$; we have $P \redd Q'$.
                            Also, let $M_0 \deq L_1 \{ N'/y_1,M_1/x_1,\ldots,M_n/x_n \}$; we have $M \aredd M_0$.
                            Moreover, $Q' \subLift M_0$.
                            Since $Q' \redd^{k-1} Q$, the thesis follows from \ih2.

                        \item
                            Case $i=2$.
                            We have $\alTrans(N){y_1} = \pSelR {y_1} ; \alTrans(N'){y_1}$.
                            Let
                            \[
                                Q_0 \deq \pRes{y_1} ( \alTrans(N'){y_1} \| \pRes{y_2} ( \pFwd [y_2<>y_1] \| \alTrans(L_2)z ) )
                            \]
                            for which we have $\alTrans(M')z \redd Q_0$.

                            From $Q_0$ several reductions are possible: $\alTrans(N'){y_1}$ or $\alTrans(L_2)z$ reduce internally, a spawn prefix in $\alTrans(N'){y_1}$ commutes past the restriction on $y_1$, a spawn prefix in $\alTrans(L_2)z$ commutes past or interacts with the restriction on $y_2$, or the forwarder $\pFwd [y_2<>y_1]$ interacts with the restriction on $y_1$.
                            These reductions are independent, so we postpone all but the forwarder reduction.
                            Let
                            \[
                                Q_1 \deq \pRes{y_2} ( \alTrans(N'){y_2} \| \alTrans(L_2)z );
                            \]
                            we have $Q_0 \redd Q_1$.

                            Let $Q' \deq \pRes{x_n} ( \alTrans(M_n){x_n} \| \ldots \pRes{x_1} ( \alTrans(M_1){x_1} \| Q_1 ) \ldots )$; we have $P \redd^2 Q'$.
                            Also, let $M_0 \deq L_2 \{ N'/y_2,M_1/x_1,\ldots,M_n/x_n \}$; we have $M \aredd M_0$.
                            Moreover, $Q' \subLift M_0$.
                            Since $Q' \redd^{k-2} Q$, the thesis follows from \ih2.
                    \end{itemize}

            \end{itemize}

        \item
            A forwarder in $\alTrans(M_i){x_i}$ for $i \in [1,n]$ interacts with a cut.
            We apply induction on the number $k$ of reductions from $P$ to $Q$, i.e., $P \redd^k Q$.

            We have $\alTrans(M_i){x_i} = \pFwd [x_i<>y]$ for some $y$.
            Hence, $M_i = y$.
            Let
            \[
                Q' \deq \pRes{x_n} ( \alTrans(M_n){x_n} \| \ldots \pRes{x_1} ( \alTrans(M_1){x_1} \| \alTrans(M' \{y/x_i \})z ) \ldots )
            \]
            without the cut on $x_i$.
            Since $\alTrans(M')z \{y/x_i \} = \alTrans(M' \{y/x_i \})z$, we have $P \redd Q'$.
            By typability, none of the $M_1,\ldots,M_{i-1}$ can contain the variable $y$, so we have
            \[
                M' \{ M_1/x_1,\ldots,y/x_i,\ldots,M_n/x_n \} = (M' \{ y/x_i \}) \{ M_1/x_1,\ldots,M_n/x_n \}
            \]
            where the latter substitutions do not contain the substitution on $x_i$.
            Hence, $Q' \subLift M$.
            Since $Q' \redd^{k-1} Q$, by the IH, there exist $N$ and $R$ such that $M \aredd^* N$ and $Q' \redd* R \subLift N$.
            This proves the thesis.

        \item
            A forwarder in $\alTrans(M')z$ interacts with a cut.
            We apply induction on the number $k$ of reductions from $P$ to $Q$, i.e., $P \redd^k Q$.

            We have $\alTrans(M')z = \pFwd [z<>y]$ for some $y$ and there exist $i \in [1,n]$ such that $x_i = y$.
            Hence, ${M' = y}$ and $M = y \{ M_1/x_1,\ldots,M_i/y,\ldots,M_n/x_n \}$.
            Let \[
                Q' \deq \pRes{x_n} ( \alTrans(M_n){x_n} \| \ldots \pRes{x_1} ( \alTrans(M_1){x_1} \| \alTrans(M_i)z ) \ldots ).
            \]
            Since $\alTrans(M_i){y} \{ z/y \} = \alTrans(M_i)z$, we have $P \redd Q'$.
            By typability, none of the $M_1,\ldots,M_{i-1}$ can contain the variable $y$, so we have
            \[
                y \{ M_1/x_1,\ldots,M_i/y,\ldots,M_n/x_n \} = M_i \{ M_1/x_1,\ldots,M_n/x_n \}
            \]
            where the latter substitutions do not contain the substitution on $x_i$.
            Hence, $Q' \subLift M$.
            Since $Q' \redd^{k-1} Q$, by the IH, there exist $N$ and $R$ such that $M \aredd^* N$ and $Q' \redd* R \subLift N$.
            This proves the thesis.

        \item
            A spawn prefix in $\alTrans(M')z$ commutes past or interacts with a cut.
            We apply induction on the number $k$ of reductions from $P$ to $Q$, i.e., $P \redd^k Q$.
            The last applied rule in the typing derivation of $\alTrans(M')z$ is Rule~\ruleLabel{typ-weaken} or Rule~\ruleLabel{typ-contract}; the rest of the analysis depends on which:
            \begin{itemize}
                \item
                    Rule~\ruleLabel{typ-weaken}.
                    The rule weakens the variables $y_1,\ldots,y_m$.
                    This case follows by commuting the spawn prefix past cuts on $x_i \notin \{y_1,\ldots,y_m\}$ and performing the weakening when the spawn prefix meets cuts on $x_i \in \{y_1,\ldots,y_m\}$.
                    Other reductions that were possible from $P$ remain possible throughout this process, but they are independent of these reductions, so we can postpone them.
                    After $k'$ steps of reduction, we reach from $P$ a process $Q'$ with the spawn commuted to the top of the process, and some cuts removed.
                    The cuts that were removed concern substitutions of weakened variables, so removing these substitutions from $M$ makes no difference.
                    Similarly, the cuts that were commuted past concern substitutions that are independent of the weakening.
                    Hence, $Q' \subLift M$.
                    Since \mbox{$M \aredd^* M$} and $Q' \redd^{k-k'} Q$, the thesis follows from the IH.

                \item
                    Rule~\ruleLabel{typ-contract}.
                    This case is largely analogous to the case of Rule~\ruleLabel{typ-weaken}, except that interactions of the spawn with cuts duplicates the cuts, and commuting past cuts moves the substitutions related to the contraction towards the end of the list of substitutions applied in $M$.
            \end{itemize}

        \item
            A spawn prefix in $\alTrans(M_i){x_i}$ for $i \in [1,n]$ commutes past a cut.
            This case is largely analogous to the previous case: first, the spawn can always commute past the cut on $x_i$, after which it may commute further or interact with cuts.
            \qedhere

    \end{itemize}
\end{proof}
%</alphalambda:oc:soundness>

%%% Local Variables:
%%% mode: latex
%%% TeX-master: "../main"
%%% End:
