# Supplementary material for: Correctly Communicating Software: Distributed, Asynchronous, and Beyond (extended version)
Source: arXiv:2402.09595 source file (2024-03-01)
Supplement: Supplementary file 4 [file pi-comparison.tex]

\section{Proof of Separation of Lazy and Eager Semantics}
\label{a:piBisim}

%<*clpi:bisim>
\begin{itemize}

    \item
        \Cref{d:clpi:readyPrefixDual} defines when prefixes are duals.

    \item
        \Cref{l:clpi:readyPrefixDual} states that when a process typed under empty context has a ready prefix (\Cref{d:clpi:readyPrefix}), the process can reduce to a state where the prefix's dual is ready too.

\end{itemize}

\begin{definition}[Dual Prefix]
    \label{d:clpi:readyPrefixDual}
    Given prefixes $\alpha$ and $\beta$ (\Cref{d:clpi:prefix}), we say $\alpha$ and $\beta$ are duals, denoted $\alpha \dualPrefix \beta$, if and only if
    $\subjs(\alpha) \cap \subjs(\beta) \neq \emptyset$.
\end{definition}

\begin{lemma}
    \label{l:clpi:readyPrefixDual}
    Given $\vdash P \typInf \emptyset$, if $P \readyPrefix{\alpha}$, then there exist $P',\beta$ such that $P \reddEager^\ast P' \readyPrefix{\beta}$ and $\alpha \dualPrefix \beta$.
\end{lemma}

\begin{proof}
    By well-typedness, there appears $\beta$ in $P$ with $\alpha \dualPrefix \beta$.
    However, we may have $P \nreadyPrefix{\beta}$, because $\beta$ is blocked by other prefixes.
    Hence, we need to find reductions from $P$ such that we unblock $\beta$.
    However, the prefixes blocking $\beta$ are connected to dual prefixes, that may be blocked themselves.
    The crux of this proof is thus to show that we can reduce $P$, such that we eventually unblock $\beta$.

    The proof is by induction on the number of names that may block $\beta$ (\ih{1}).
    Initially, this number corresponds to the total number of names appearing in $P$.
    Suppose $\beta$ is blocked by $n$ prefixes $\gamma_i$, where $\gamma_n$ blocks $\beta$, and $\gamma_1$ is not blocked.
    We apply another layer of induction on $n$ (\ih{2}).

    In the inductive case, $n \geq 1$.
    The goal is to perform a reduction that synchronizes $\gamma_1$ with its dual, say $\ol{\gamma_1}$.
    The prefix $\ol{\gamma_1}$ may be blocked by a number of prefixes itself.
    However, the type system of \clpi is based on Rule~\ruleLabel{typ-cut}, so $\ol{\gamma_1}$ appears in parallel with the duals of $\gamma_2,\ldots,\gamma_n$ and $\alpha$.
    We then may apply \ih{1} to find $P \reddEager^\ast P_0 \readyPrefix{\ol{\gamma_1}}$.
    We can then reduce $P_0$ by synchronizing between $\gamma_1$ and $\ol{\gamma_1}$: $P \reddEager^\ast P_0 \reddEager P_1$.
    In $P_1$, $\beta$ is blocked by one less prefix.
    Hence, by \ih{2}, $P \reddEager^\ast P_0 \reddEager P_1 \reddEager^\ast P' \readyPrefix{\beta}$, proving the thesis.

    In the base case, $\beta$ is not blocked: $P \readyPrefix{\beta}$.
    Let $P' \deq P$; trivially, $P \reddEager^\ast P' \readyPrefix{\beta}$, proving the thesis.
\end{proof}

\tClpiBisim*

\begin{proof}
    For~(i), we construct a relation $\mbb{B}$ as follows:
    \begin{align*}
        \sff{Id}^\equiv
        &\deq
        \{ (T,U) \mid T \equiv U \}
        \\
        \mbb{B}'
        &\deq
        \{
            (T,U) \mid \begin{array}[t]{@{}l@{}}
                \vdash T \equiv \evalCtx{M}[\beta_1 ; (V \nd W)] \typInf \emptyset
                \text{ and}
                \\
                \vdash U \equiv \evalCtx{M}[\beta_2 ; V \nd \beta_3 ; W] \typInf \emptyset
                \text{ and}
                \\
                V \nreadyPrefixBisim{L} W
                \text{ and}
                \\
                \beta_1 \prefRel \beta_2 \prefRel \beta_3
                \text{ and}
                \\
                \text{$\beta_1,\beta_2,\beta_3$ require a continuation}
            \}
        \end{array}
        \\
        \mbb{B}
        &\deq
        \sff{Id}^\equiv \cup \mbb{B}'
    \end{align*}

    We prove that $\mbb{B}$ is a strong ready-prefix bisimulation w.r.t.\ the lazy semantics by proving the three conditions of \Cref{d:clpi:readyPrefixBisim} for each $(T,U) \in \mbb{B}$.
    We distinguish cases depending on whether $(T,U) \in \sff{Id}^\equiv$ or $(T,U) \in \mbb{B}'$.
    \begin{itemize}

        \item
            $(T,U) \in \sff{Id}^\equiv$.
            The three conditions hold trivially.

        \item
            $(T,U) \in \mbb{B}'$.
            Then $T \equiv \evalCtx{M}[\beta_1 ; (V \nd W)]$, $U \equiv \evalCtx{M}[\beta_2 ; V \nd \beta_3 ; W]$, $V \nreadyPrefixBisim{L} W$, and \mbox{$\beta_1 \prefRel \beta_2 \prefRel \beta_3$}.
            We prove each condition separately.
            \begin{enumerate}

                \item
                    Suppose $T \reddLazy T'$.
                    Note that the hole in $\evalCtx{M}$ may appear inside a non-deterministic choice.
                    We distinguish three cases: (a)~the reduction is inside $\evalCtx{M}$ and maintains the branch with the hole, (b)~the reduction is inside $\evalCtx{M}$ and discards the branch with the hole, or (c)~the reduction synchronizes on $\beta_1$.
                    \begin{enumerate}

                        \item
                            The reduction is inside $\evalCtx{M}$ and maintains the branch with the hole.
                            Then $T' \equiv \evalCtx{M'}[\beta_1 ; (V \nd W)]$ and $U \reddLazy U' \equiv \evalCtx{M'}[\beta_2 ; V \nd \beta_3 ; W]$.
                            Clearly, $(T',U') \in \mbb{B}'$, so $(T',U') \in \mbb{B}$.

                        \item
                            The reduction is inside $\evalCtx{M}$ and discards the branch with the hole.
                            Then there exists $U'$ such that $U \reddLazy U' \equiv T'$, so $(T',U') \in \sff{Id}^\equiv$, and thus $(T',U') \in \mbb{B}$.

                        \item
                            The reduction synchronizes on $\beta_1$.
                            Then $T' \equiv \evalCtx{M'}[V \nd W]$ and, since \mbox{$\beta_1 \prefRel \beta_2 \prefRel \beta_3$}, $U \reddLazy U' \equiv \evalCtx{M'}[V \nd W]$.
                            Then $T' \equiv U'$, so $(T',U') \in \sff{Id}^\equiv$ and thus $(T',U') \in \mbb{B}$.

                    \end{enumerate}

                \item
                    Suppose $U \reddLazy U'$.
                    By reasoning analogous to above, $T \reddLazy T'$ and $(T',U') \in \mbb{B}$.

                \item
                    Suppose $T \readyPrefix{\gamma}$.
                    If the prefix $\gamma$ appears in $\evalCtx{M}$, then clearly also $U \readyPrefix{\gamma}$.
                    Otherwise, $\gamma = \beta_1$.
                    We have, e.g., $\gamma \prefRel \beta_2$ and clearly $U \readyPrefix{\beta_2}$.
                    The other direction is analogous.

            \end{enumerate}

    \end{itemize}

    It remains to show that $(R,S) \in \mbb{B}$ which trivially holds.

    \medskip
    For~(ii), toward a contradiction, assume there exists a strong ready-prefix bisimulation w.r.t.\ $\reddEager$ $\mbb{B}$ where $(R,S) \in \mbb{B}$.

    By \Cref{l:clpi:readyPrefixDual}, there exist $R',\beta_1$ such that $R \reddEager^\ast R' \readyPrefix{\beta_1}$, and $\alpha_1 \dualPrefix \beta_1$.
    By the well-typedness of $R$ and $S$, $\beta_1$ must appear in $\evalCtx{N}$, and the reduction $R \reddEager^\ast R'$ takes place in $\evalCtx{N}$.
    Take $x \in \subjs(\alpha_1) \cap \subjs(\beta_1)$ (which is non-empty by \Cref{l:clpi:readyPrefixDual}).
    Then \mbox{$R' \equiv \evalCtx[\big]{N'_1}[\pRes{x} ( \evalCtx{N'_2}[\beta_1 ; R'_2] \| \evalCtx{N'_3}[\alpha_1 ; (P \nd Q)] )]$}.
    Moreover, clearly $S \reddEager^\ast S'$ following the same reductions, resulting in $S' \equiv \evalCtx[\big]{N'_1}[\pRes{x} ( \evalCtx{N'_2}[\beta_1 ; R'_2] \| \evalCtx{N'_3}[\alpha_2 ; P \nd \alpha_3 ; Q] )]$; note that, since \mbox{$\alpha_1 \prefRel \alpha_2 \prefRel \alpha_3$}, also $\alpha_2 \dualPrefix \beta_1$ and $\alpha_3 \dualPrefix \beta_1$.
    At this point, we must have $(R',S') \in \mbb{B}$.

    The synchronization between $\beta_1$ and $\alpha_1$ gives $R' \reddEager R'' \equiv \evalCtx{N''}[P \nd Q]$.
    Then by the bisimulation, there exists $S''$ such that $S' \reddEager S''$ with $(R'',S'') \in \mbb{B}$.
    By clause~3 of the bisimulation, $R''$ and $S''$ must have the same ready-prefixes, so clearly the reduction $S' \reddEager S''$ results from a synchronization between $\beta_1$ and either of $\alpha_2$ and $\alpha_3$.
    W.l.o.g., let us assume this was $\alpha_3$.
    Then $S'' \equiv \evalCtx{N''}[Q]$.
    By assumption, $P \nreadyPrefixBisim{E} Q$ and thus $P \nd Q \nreadyPrefixBisim{E} Q$, so clearly $R'' \nreadyPrefixBisim{E} S''$.
    Hence, $\mbb{B}$ cannot be a strong ready-prefix bisimulation w.r.t.\ $\reddEager$.
    In other words, $R \nreadyPrefixBisim{E} S$.
\end{proof}
%</clpi:bisim>
