# Supplementary material for: Correctly Communicating Software: Distributed, Asynchronous, and Beyond (extended version)
Source: arXiv:2402.09595 source file (2024-03-01)
Supplement: Supplementary file 5 [file pi-proofs.tex]

% !TeX root = ../../../../main.tex
\section{Proofs of Type Preservation and Deadlock-freedom for (Full) \texorpdfstring{\clpi}{Pi}}
\label{s:piProofs}

Here we prove \Cref{t:srPi,t:dfPi} (type preservation and deadlock-freedom for the lazy semantics, respectively), as well as the analogue results for the eager semantics.
In fact, deadlock-freedom for the lazy semantics follows from deadlock-freedom for the eager semantics, so we present the proofs for the eager semantics first.

\subsection{Eager Semantics}
\label{ss:proofsEager}

\subsubsection{Subject Congruence}

%<*clpi:tp:sc>
\begin{theorem}
    \label{t:clpi:sc}
    If $\vdash P \typInf \Gamma$ and $P \equiv Q$, then $\vdash Q \typInf \Gamma$.
\end{theorem}

\begin{proof}
    
    By induction on the derivation of the structural congruence.
    We first detail the base cases.
    In each case we apply inversion on the typing of $P$ and derive the typing of $Q$; this straightforwardly works in both directions.
    \begin{itemize}
        \item
            Rule~\ruleLabel{cong-alpha}:
            $P \equiv_\alpha Q \implies P \equiv Q$.
            Since alpha-renaming only affects bound names, it does not affect the names in $\Gamma$, so clearly $\vdash Q \typInf \Gamma$.

        \item
            Rule~\ruleLabel{cong-fwd-symm}:
            $\pFwd [x<>y] \equiv \pFwd [y<>x]$.
            \begin{mathpar}
                \begin{bussproof}
                    \bussAx[\ruleLabel{typ-fwd}]{
                        \vdash \pFwd [x<>y] \typInf x:A, y:\ol{A}
                    }
                \end{bussproof}
                \and
                \equiv
                \and
                \begin{bussproof}
                    \bussAx[\ruleLabel{typ-fwd}]{
                        \vdash \pFwd [y<>x] \typInf x:A, y:\ol{A}
                    }
                \end{bussproof}
            \end{mathpar}

        \item
            Rule~\ruleLabel{cong-par-unit}:
            $P \| \0 \equiv P$.
            \begin{mathpar}
                \begin{bussproof}
                    \bussAssume{
                        \vdash P \typInf \Gamma
                    }
                    \bussAx[\ruleLabel{typ-inact}]{
                        \vdash \0 \typInf \emptyset
                    }
                    \bussBin[\ruleLabel{typ-par}]{
                        \vdash P \| \0 \typInf \Gamma
                    }
                \end{bussproof}
                \and
                \equiv
                \and
                \vdash P \typInf \Gamma
            \end{mathpar}

        \item
            Rule~\ruleLabel{cong-par-assoc}:
            $(P \| Q) \| R \equiv P \| (Q \| R)$.
            \begin{mathpar}
                \begin{bussproof}
                    \bussAssume{
                        \vdash P \typInf \Gamma
                    }
                    \bussAssume{
                        \vdash Q \typInf \Delta
                    }
                    \bussBin[\ruleLabel{typ-par}]{
                        \vdash P \| Q \typInf \Gamma, \Delta
                    }
                    \bussAssume{
                        \vdash R \typInf \Lambda
                    }
                    \bussBin[\ruleLabel{typ-par}]{
                        \vdash (P \| Q) \| R \typInf \Gamma, \Delta, \Lambda
                    }
                \end{bussproof}
                \and
                \equiv
                \and
                \begin{bussproof}
                    \bussAssume{
                        \vdash P \typInf \Gamma
                    }
                    \bussAssume{
                        \vdash Q \typInf \Delta
                    }
                    \bussAssume{
                        \vdash R \typInf \Lambda
                    }
                    \bussBin[\ruleLabel{typ-par}]{
                        \vdash Q \| R \typInf \Delta, \Lambda
                    }
                    \bussBin[\ruleLabel{typ-par}]{
                        \vdash P \| (Q \| R) \typInf \Gamma, \Delta, \Lambda
                    }
                \end{bussproof}
            \end{mathpar}

        \item
            Rule~\ruleLabel{cong-par-comm}:
            $P \| Q \equiv Q \| P$.
            \begin{mathpar}
                \begin{bussproof}
                    \bussAssume{
                        \vdash P \typInf \Gamma
                    }
                    \bussAssume{
                        \vdash Q \typInf \Delta
                    }
                    \bussBin[\ruleLabel{typ-par}]{
                        \vdash P \| Q \typInf \Gamma, \Delta
                    }
                \end{bussproof}
                \and
                \equiv
                \and
                \begin{bussproof}
                    \bussAssume{
                        \vdash Q \typInf \Delta
                    }
                    \bussAssume{
                        \vdash P \typInf \Gamma
                    }
                    \bussBin[\ruleLabel{typ-par}]{
                        \vdash Q \| P \typInf \Gamma, \Delta
                    }
                \end{bussproof}
            \end{mathpar}

        \item
            Rule~\ruleLabel{cong-conn-symm}:
            $\pRes{x} ( P \| Q ) \equiv \pRes{x} ( Q \| P )$.
            \begin{mathpar}
                \begin{bussproof}
                    \bussAssume{
                        \vdash P \typInf \Gamma, x:A
                    }
                    \bussAssume{
                        \vdash Q \typInf \Delta, x:\ol{A}
                    }
                    \bussBin[\ruleLabel{typ-cut}]{
                        \vdash \pRes{x} ( P \| Q ) \typInf \Gamma, \Delta
                    }
                \end{bussproof}
                \and
                \equiv
                \and
                \begin{bussproof}
                    \bussAssume{
                        \vdash Q \typInf \Delta, x:\ol{A}
                    }
                    \bussAssume{
                        \vdash P \typInf \Gamma, x:A
                    }
                    \bussBin[\ruleLabel{typ-cut}]{
                        \vdash \pRes{x} ( Q \| P ) \typInf \Gamma, \Delta
                    }
                \end{bussproof}
            \end{mathpar}

        \item
            Rule~\ruleLabel{cong-conn-par}:
            $x \notin \fn(Q) \implies \pRes{x} ( ( P \| Q ) \| R ) \equiv \pRes{x} ( P \| R ) \| Q$.
            Assume the condition.
            \begin{mathpar}
                \begin{bussproof}
                    \bussAssume{
                        \vdash P \typInf \Gamma, x:A
                    }
                    \bussAssume{
                        \vdash Q \typInf \Delta
                    }
                    \bussBin[\ruleLabel{typ-par}]{
                        \vdash P \| Q \typInf \Gamma, \Delta, x:A
                    }
                    \bussAssume{
                        \vdash R \typInf \Lambda, x:\ol{A}
                    }
                    \bussBin[\ruleLabel{typ-cut}]{
                        \vdash \pRes{x} ( ( P \| Q ) \| R ) \typInf \Gamma, \Delta, \Lambda
                    }
                \end{bussproof}
                \and
                \equiv
                \and
                \begin{bussproof}
                    \bussAssume{
                        \vdash P \typInf \Gamma, x:A
                    }
                    \bussAssume{
                        \vdash R \typInf \Lambda, x:\ol{A}
                    }
                    \bussBin[\ruleLabel{typ-cut}]{
                        \vdash \pRes{x} ( P \| R ) \typInf \Gamma, \Lambda
                    }
                    \bussAssume{
                        \vdash Q \typInf \Delta
                    }
                    \bussBin[\ruleLabel{typ-par}]{
                        \vdash \pRes{x} ( P \| R ) \| Q \typInf \Gamma, \Delta, \Lambda
                    }
                \end{bussproof}
            \end{mathpar}

        \item
            Rule~\ruleLabel{cong-conn-conn}:
            $x \notin \fn(Q) \implies \pRes{x} (\pRes{y} (P \| Q) \| R) \equiv \pRes{y} (\pRes{x} (P \| R) \| Q)$.
            Assume the condition.
            \begin{mathpar}
                \begin{bussproof}
                    \bussAssume{
                        \vdash P \typInf \Gamma, y:A, x:B
                    }
                    \bussAssume{
                        \vdash Q \typInf \Delta, y:\ol{A}
                    }
                    \bussBin[\ruleLabel{typ-cut}]{
                        \vdash \pRes{y} ( P \| Q ) \typInf \Gamma, \Delta, x:B
                    }
                    \bussAssume{
                        \vdash R \typInf \Lambda, x:\ol{B}
                    }
                    \bussBin[\ruleLabel{typ-cut}]{
                        \vdash \pRes{x} ( \pRes{y} ( P \| Q ) \| R ) \typInf \Gamma, \Delta, \Lambda
                    }
                \end{bussproof}
                \and
                \equiv
                \and
                \begin{bussproof}
                    \bussAssume{
                        \vdash P \typInf \Gamma, y:A, x:B
                    }
                    \bussAssume{
                        \vdash R \typInf \Lambda, x:\ol{B}
                    }
                    \bussBin[\ruleLabel{typ-cut}]{
                        \vdash \pRes{x} ( P \| R ) \typInf \Gamma, \Lambda, y:A
                    }
                    \bussAssume{
                        \vdash Q \typInf \Delta, y:\ol{A}
                    }
                    \bussBin[\ruleLabel{typ-cut}]{
                        \vdash \pRes{y} ( \pRes{x} ( P \| R ) \| Q ) \typInf \Gamma, \Delta, \Lambda
                    }
                \end{bussproof}
            \end{mathpar}

        \item
            Rule~\ruleLabel{cong-nd-refl}:
            $P \nd P \equiv P$.
            \begin{mathpar}
                \begin{bussproof}
                    \bussAssume{
                        \vdash P \typInf \Gamma
                    }
                    \bussAssume{
                        \vdash P \typInf \Gamma
                    }
                    \bussBin[\ruleLabel{typ-nd}]{
                        \vdash P \nd P \typInf \Gamma
                    }
                \end{bussproof}
                \and
                \equiv
                \and
                \vdash P \typInf \Gamma
            \end{mathpar}

        \item
            Rule~\ruleLabel{cong-nd-symm}:
            $P \nd Q \equiv Q \nd P$.
            \begin{mathpar}
                \begin{bussproof}
                    \bussAssume{
                        \vdash P \typInf \Gamma
                    }
                    \bussAssume{
                        \vdash Q \typInf \Gamma
                    }
                    \bussBin[\ruleLabel{typ-nd}]{
                        \vdash P \nd Q \typInf \Gamma
                    }
                \end{bussproof}
                \and
                \equiv
                \and
                \begin{bussproof}
                    \bussAssume{
                        \vdash Q \typInf \Gamma
                    }
                    \bussAssume{
                        \vdash P \typInf \Gamma
                    }
                    \bussBin[\ruleLabel{typ-nd}]{
                        \vdash Q \nd P \typInf \Gamma
                    }
                \end{bussproof}
            \end{mathpar}

        \item
            Rule~\ruleLabel{cong-nd-assoc}:
            $( P \nd Q ) \nd R \equiv P \nd ( Q \nd R )$
            \begin{mathpar}
                \begin{bussproof}
                    \bussAssume{
                        \vdash P \typInf \Gamma
                    }
                    \bussAssume{
                        \vdash Q \typInf \Gamma
                    }
                    \bussBin[\ruleLabel{typ-nd}]{
                        \vdash P \nd Q \typInf \Gamma
                    }
                    \bussAssume{
                        \vdash R \typInf \Gamma
                    }
                    \bussBin[\ruleLabel{typ-nd}]{
                        \vdash ( P \nd Q ) \nd R \typInf \Gamma
                    }
                \end{bussproof}
                \and
                \equiv
                \and
                \begin{bussproof}
                    \bussAssume{
                        \vdash P \typInf \Gamma
                    }
                    \bussAssume{
                        \vdash Q \typInf \Gamma
                    }
                    \bussAssume{
                        \vdash R \typInf \Gamma
                    }
                    \bussBin[\ruleLabel{typ-nd}]{
                        \vdash Q \nd R \typInf \Gamma
                    }
                    \bussBin[\ruleLabel{typ-nd}]{
                        \vdash P \nd ( Q \nd R ) \typInf \Gamma
                    }
                \end{bussproof}
            \end{mathpar}

        \item
            Rule~\ruleLabel{cong-srv}:
            $x \notin \fn(Q) \implies \pRes{x} (\pSrv x(y);P \| Q) \equiv Q$.
            Assume the condition.
            \begin{mathpar}
                \begin{bussproof}
                    \bussAssume{
                        \vdash P \typInf {?}\Gamma, y{:}A
                    }
                    \bussUn[\ruleLabel{typ-srv}]{
                        \vdash \pSrv x(y) ; P \typInf {?}\Gamma, x:{!}A
                    }
                    \bussAssume{
                        \vdash Q \typInf \Delta
                    }
                    \bussUn[\ruleLabel{typ-weaken}]{
                        \vdash Q \typInf \Delta, x:{?}\ol{A}
                    }
                    \bussBin[\ruleLabel{typ-cut}]{
                        \vdash \pRes{x} ( \pSrv x(y) ; P \| Q ) \vdash {?}\Gamma, \Delta
                    }
                \end{bussproof}
                \and
                \equiv
                \and
                \begin{bussproof}
                    \bussAssume{
                        \vdash Q \typInf \Delta
                    }
                    \doubleLine
                    \bussUn[$\ruleLabel{typ-weaken}^\ast$]{
                        \vdash Q \typInf {?}\Gamma, \Delta
                    }
                \end{bussproof}
            \end{mathpar}
    \end{itemize}
    The inductive cases follow from the IH straightforwardly.
\end{proof}
%</clpi:tp:sc>

\subsubsection{Subject Reduction}

%<*clpi:tp:srEager>
\begin{lemma}
    \label{l:clpi:ctxType}
    Suppose $\vdash P \typInf \Gamma, x:A$.
    \begin{enumerate}
        \item\label{i:clpi:ctxType:close}
            If $P = \evalCtx{N}[\pClose x[]]$, then $A = \1$.

        \item\label{i:clpi:ctxType:wait}
            If $P = \evalCtx{N}[\pWait x() ; P']$, then $A = \bot$.

        \item\label{i:clpi:ctxType:send}
            If $P = \evalCtx{N}[\pOut* x[y] ; ( P' \| P'' )]$, then $A = B \tensor C$.

        \item\label{i:clpi:ctxType:recv}
            If $P = \evalCtx{N}[\pIn x(y) ; P']$, then $A = B \parr C$.

        \item\label{i:clpi:ctxType:sel}
            If $P = \evalCtx{N}[\pSel* x < j ; P']$, then $A = \oplus \{ i : B_i \}_{i \in I}$ where $j \in I$.

        \item\label{i:clpi:ctxType:bra}
            If $P = \evalCtx{N}[\pBra* x > \{ i : P'_i \}_{i \in I}]$, then $A = \& \{ i : B_i \}_{i \in I}$.

        \item\label{i:clpi:ctxType:some}
            If $P = \evalCtx{N}[\pSome x ; P']$, then $A = \& B$.

        \item\label{i:clpi:ctxType:none}
            If $P = \evalCtx{N}[\pNone x]$, then $A = \& B$.

        \item\label{i:clpi:ctxType:someIn}
            If $P = \evalCtx{N}[\pSomeIn x{w_1,\ldots,w_n} ; P']$, then $A = \oplus B$.

        \item\label{i:clpi:ctxType:cli}
            If $P = \evalCtx{N}[\pCli* x[y] ; P']$, then $A = {?}B$.

        \item\label{i:clpi:ctxType:srv}
            If $P = \evalCtx{N}[\pSrv x(y) ; P']$, then $A = {!}B$.
    \end{enumerate}
\end{lemma}

\begin{proof}
    Each item follows by induction on the structure of the ND-context.
    The base case follows by inversion of typing, and the inductive cases follow from the IH straightforwardly.
\end{proof}

\begin{lemma}
    \label{l:clpi:reddEager}
    For each of the following items, assume $\Gamma \cap \Delta = \emptyset$.
    \begin{enumerate}
        \item\label{i:clpi:reddEager:fwd}
            If $\vdash \evalCtx[\big]{N}[\pFwd [x<>y]] \typInf \Gamma, x:A$ and $\vdash Q \typInf \Delta, x:\ol{A}$, then $\vdash \evalCtx{\D{N}}[Q \{ y/x \}] \typInf \Gamma, \Delta$.

        \item\label{i:clpi:reddEager:close}
            If $\vdash \evalCtx{N}[\pClose x[]] \typInf \Gamma, x:\1$, then $\vdash \evalCtx{\D{N}}[\0] \typInf \Gamma$.

        \item\label{i:clpi:reddEager:wait}
            If $\vdash \evalCtx{N}[\pWait x() ; Q] \typInf \Gamma, x:\bot$, then $\vdash \evalCtx{\D{N}}[Q] \typInf \Gamma$.

        \item\label{i:clpi:reddEager:sendRecv}
            If $\bn(\evalCtx{N)} \cap \fn(\evalCtx{N'}) = \emptyset$ and $\vdash \evalCtx{N}[\pOut* x[y] ; ( P \| Q )] \typInf \Gamma, x:A \tensor B$ and $\vdash \evalCtx{N'}[\pIn x(z) ; R] \typInf \Delta, x:\ol{A} \parr \ol{B}$, then $\vdash \evalCtx{\D{N}}[\pRes{x} ( Q \| \pRes{y} ( P \| \evalCtx{\D{N'}}[R \{ y/z \}] ) )] \typInf \Gamma, \Delta$.

        \item\label{i:clpi:reddEager:sel}
            If $\vdash \evalCtx{N}[\pSel* x < j ; P] \typInf \Gamma, x:\oplus \{ i : A_i \}_{i \in I}$ and $j \in I$, then $\vdash \evalCtx{\D{N}}[P] \typInf \Gamma, x:A_j$.

        \item\label{i:clpi:reddEager:bra}
            If $\vdash \evalCtx{N}[\pBra* x > \{ i : P_i \}_{i \in I}] \typInf \Gamma, x:\& \{ i : A_i \}_{i \in I}$, then $\vdash \evalCtx{\D{N}}[P_i] \typInf \Gamma, x:A_i$ for every $i \in I$.

        \item\label{i:clpi:reddEager:some}
            If $\vdash \evalCtx{N}[\pSome x ; P] \typInf \Gamma, x:\& A$, then $\vdash \evalCtx*{N}[P] \typInf \Gamma, x:A$.

        \item\label{i:clpi:reddEager:none}
            If $\vdash \evalCtx{N}[\pNone x] \typInf \Gamma, x:\& A$, then $\vdash \evalCtx{\D{N}}[\0] \typInf \Gamma$.

        \item\label{i:clpi:reddEager:someIn}
            If $\vdash \evalCtx{N}[\pSomeIn x{w_1,\ldots,w_n} ; P] \typInf \Gamma, x:\oplus A$, then $\vdash \evalCtx{\D{N}}[P] \typInf \Gamma, x:A$ and \mbox{$\vdash \evalCtx{\D{N}}[\pNone w_1 \| \ldots \| \pNone w_n] \typInf \Gamma$}.

        \item\label{i:clpi:reddEager:cliSrv}
            If $\bn(\evalCtx{N'}) \cap \fn(\evalCtx{N}) = \emptyset$ and $\vdash \evalCtx{N}[\pCli* x[y] ; P] \typInf \Gamma, x:{?}A$ and $\vdash \evalCtx{N}'[\pSrv x(y) ; Q] \typInf \Delta, x:{!}\ol{A}$, then $\vdash \evalCtx[\big]{\D{N'}}[\pRes{x} ( \pRes{y} ( \evalCtx{\D{N}}[P] \| Q \{ y/z \} ) \| \pSrv x(z) ; Q )]$.
    \end{enumerate}
\end{lemma}

\begin{proof}
    For each item, we apply induction on the structure of the ND-contexts.
    In each case, we detail the base case: $\evalCtx{N} = \evalHole$.
    For simplicity, w.l.o.g., we assume no names in $\Gamma$ and $\Delta$ were derived with \ruleLabel{typ-weaken}.
    In each case, we derive the typing of the condition, and infer the typing of the conclusion.
    \begin{enumerate}
        \item
            \begin{mathpar}
                \begin{bussproof}
                    \bussAx[\ruleLabel{typ-fwd}]{
                        \vdash \pFwd [x<>y] \typInf x:A, y:\ol{A}
                    }
                \end{bussproof}
                \and
                \land
                \and
                \vdash Q \typInf \Delta, x:\ol{A}
                \and
                \implies
                \and
                \vdash Q \{ y/x \} \typInf \Delta, y:\ol{A}
            \end{mathpar}

        \item
            \begin{mathpar}
                \begin{bussproof}
                    \bussAx[\ruleLabel{typ-close}]{
                        \vdash \pClose x[] \typInf x:\1
                    }
                \end{bussproof}
                \and
                \implies
                \and
                \begin{bussproof}
                    \bussAx[\ruleLabel{typ-inact}]{
                        \vdash \0 \typInf \emptyset
                    }
                \end{bussproof}
            \end{mathpar}

        \item
            \begin{mathpar}
                \begin{bussproof}
                    \bussAssume{
                        \vdash Q \typInf \Gamma
                    }
                    \bussUn[\ruleLabel{typ-wait}]{
                        \vdash \pWait x() ; Q \typInf \Gamma, x:\bot
                    }
                \end{bussproof}
                \and
                \implies
                \and
                \vdash Q \typInf \Gamma
            \end{mathpar}

        \item
            \begin{mathpar}
                \begin{bussproof}
                    \bussAssume{
                        \vdash P \typInf \Gamma, y:A
                    }
                    \bussAssume{
                        \vdash Q \typInf \Gamma', x:B
                    }
                    \bussBin[\ruleLabel{typ-send}]{
                        \vdash \pOut* x[y] ; ( P \| Q ) \typInf \Gamma, \Gamma', x:A \tensor B
                    }
                \end{bussproof}
                \and
                \land
                \and
                \begin{bussproof}
                    \bussAssume{
                        \vdash R \typInf \Delta, z:\ol{A}, x:\ol{B}
                    }
                    \bussUn[\ruleLabel{typ-recv}]{
                        \vdash \pIn x(z) ; R \typInf \Delta, x:\ol{A} \parr \ol{B}
                    }
                \end{bussproof}
                \and
                \implies
                \and
                \begin{bussproof}
                    \bussAssume{
                        \vdash Q \typInf \Gamma', x:B
                    }
                    \bussAssume{
                        \vdash P \typInf \Gamma, y:A
                    }
                    \bussAssume{
                        \vdash R \{ y/z \} \typInf \Delta, y:\ol{A}, x:\ol{B}
                    }
                    \bussBin[\ruleLabel{typ-cut}]{
                        \vdash \pRes{y} ( P \| R \{ y/z \} ) \typInf \Gamma, \Delta, x:\ol{B}
                    }
                    \bussBin[\ruleLabel{typ-cut}]{
                        \vdash \pRes{x} ( Q \| \pRes{y} ( P \| R \{ y/z \} ) ) \typInf \Gamma, \Gamma', \Delta
                    }
                \end{bussproof}
            \end{mathpar}

        \item
            \begin{mathpar}
                \begin{bussproof}
                    \bussAssume{
                        \vdash P \typInf \Gamma, x:A_j
                    }
                    \bussAssume{
                        j \in I
                    }
                    \bussBin[\ruleLabel{typ-sel}]{
                        \vdash \pSel* x < j ; P \typInf \Gamma, x:\oplus \{ i : A_i \}_{i \in I}
                    }
                \end{bussproof}
                \and
                \implies
                \and
                \vdash P \typInf \Gamma, x:A_j
            \end{mathpar}

        \item
            \begin{mathpar}
                \begin{bussproof}
                    \bussAssume{
                        \forall i \in I.~ \vdash P_i \typInf \Gamma, x:A_i
                    }
                    \bussUn[\ruleLabel{typ-bra}]{
                        \vdash \pBra* x > \{ i : P_i \}_{i \in I} \typInf \Gamma, x:\& \{ i : A_i \}
                    }
                \end{bussproof}
                \and
                \implies
                \and
                \forall i \in I.~ \vdash P_i \typInf \Gamma, x:A_i
            \end{mathpar}

        \item
            \begin{mathpar}
                \begin{bussproof}
                    \bussAssume{
                        \vdash P \typInf \Gamma, x:A
                    }
                    \bussUn[\ruleLabel{typ-some}]{
                        \vdash \pSome x ; P \typInf \Gamma, x:\& A
                    }
                \end{bussproof}
                \and
                \implies
                \and
                \vdash P \typInf \Gamma, x:A
            \end{mathpar}

        \item
            \begin{mathpar}
                \begin{bussproof}
                    \bussAx[\ruleLabel{typ-none}]{
                        \vdash \pNone x \typInf x:\& A
                    }
                \end{bussproof}
                \and
                \implies
                \and
                \begin{bussproof}
                    \bussAx[\ruleLabel{typ-inact}]{
                        \vdash \0 \typInf \emptyset
                    }
                \end{bussproof}
            \end{mathpar}

        \item
            \begin{mathpar}
                \begin{bussproof}
                    \bussAssume{
                        \vdash P \typInf w_1:\& B_1, \ldots, w_n:\& B_n, x:A
                    }
                    \bussUn[\ruleLabel{typ-some-in}]{
                        \vdash \pSomeIn x{w_1,\ldots,w_n} ; P \typInf w_1:\& B_1, \ldots, w_n:\& B_n, x:\oplus A
                    }
                \end{bussproof}
                \and
                \implies
                \and
                \vdash P \typInf w_1:\& B_1, \ldots, w_n:\& B_n, x:A
                \and
                \land
                \and
                \begin{bussproof}
                    \bussAx[\ruleLabel{typ-none}]{
                        \vdash \pNone w_1 \typInf w_1:\& B_1
                    }
                    \bussAssume{
                        \ldots
                    }
                    \bussAx[\ruleLabel{typ-none}]{
                        \vdash \pNone w_n \typInf w_n:\& B_n
                    }
                    \bussTern{
                        \vdash \pNone w_1 \| \ldots \| \pNone w_n \typInf w_1:\& B_1, \ldots, w_n:\& B_n
                    }
                \end{bussproof}
            \end{mathpar}

        \item
            This item depends on whether $x \in \fn(P)$.
            \begin{itemize}
                \item
                    Case $x \in \fn(P)$:
                    \begin{mathpar}
                        
                        \begin{bussproof}
                            \bussAssume{
                                \vdash P \{ x'/x \} \typInf \Gamma, y:A, x':{?}A
                            }
                            \bussUn[\ruleLabel{typ-cli}]{
                                \vdash \pCli* x[y] ; P \{ x'/x \} \typInf \Gamma, x:{?}A, x':{?}A
                            }
                            \bussUn[\ruleLabel{typ-contract}]{
                                \vdash \pCli* x[y] ; P \typInf \Gamma, x:{?}A
                            }
                        \end{bussproof}
                        \and
                        \land
                        \and
                        \begin{bussproof}
                            \bussAssume{
                                \vdash Q \typInf {?}\Delta, z:\ol{A}
                            }
                            \bussUn[\ruleLabel{typ-srv}]{
                                \vdash \pSrv x(z) ; Q \typInf {?}\Delta, x:{!}\ol{A}
                            }
                        \end{bussproof}
                        \and
                        \implies
                        \and
                        \begin{bussproof}
                            \bussAssume{
                                \vdash P \typInf \Gamma, y:A, x:{?}A
                            }
                            \bussAssume{
                                \begin{array}{@{}l@{}}
                                    \vdash \begin{array}{@{}l@{}}
                                        Q \{ y/z \}
                                        \\
                                        \{ w'/w \}_{w \in \dom({?}\Delta)}
                                    \end{array}
                                    \\
                                    \typInf {?}\Delta', y:\ol{A}
                                \end{array}
                            }
                            \bussBin[\ruleLabel{typ-cut}]{
                                \begin{array}{@{}l@{}}
                                    \vdash \pRes{y} ( P \| Q \{ y/z \} \{ w'/w \}_{w \in \dom({?}\Delta)})
                                    \\
                                    \typInf \Gamma, {?}\Delta', x:{?}A
                                \end{array}
                            }
                            \bussAssume{
                                \vdash Q \typInf {?}\Delta, z:\ol{A}
                            }
                            \bussUn[\ruleLabel{typ-srv}]{
                                \begin{array}{@{}l@{}}
                                    \vdash \pSrv x(z) ; Q \\
                                    \typInf {?}\Delta, x:{!}\ol{A}
                                \end{array}
                            }
                            \bussBin[\ruleLabel{typ-cut}]{
                                \vdash \pRes{x} ( \pRes{y} ( P \| Q \{ y/z \} \{ w'/w \}_{w \in \dom({?}\Delta)} ) \| \pSrv x(z) ; Q ) \typInf \Gamma, {?}\Delta, {?}\Delta'
                            }
                            \doubleLine
                            \bussUn[$\ruleLabel{typ-contract}^\ast$]{
                                \vdash \pRes{x} ( \pRes{y} ( P \| Q \{ y/z \} ) \| \pSrv x(z) ; Q ) \typInf \Gamma, {?}\Delta
                            }
                        \end{bussproof}
                    \end{mathpar}

                \item
                    Case $x \notin \fn(P)$:
                    \begin{mathpar}
                        
                        \begin{bussproof}
                            \bussAssume{
                                \vdash P \typInf \Gamma, y:A
                            }
                            \bussUn[\ruleLabel{typ-cli}]{
                                \vdash \pCli* x[y] ; P \typInf \Gamma, x:{?}A
                            }
                        \end{bussproof}
                        \and
                        \land
                        \and
                        \begin{bussproof}
                            \bussAssume{
                                \vdash Q \typInf {?}\Delta, z{:}\ol{A}
                            }
                            \bussUn[\ruleLabel{typ-srv}]{
                                \vdash \pSrv x(z) ; Q \typInf {?}\Delta, x:{!}\ol{A}
                            }
                        \end{bussproof}
                        \and
                        \implies
                        \and
                        \begin{bussproof}
                            \bussAssume{
                                \vdash P \typInf \Gamma, y:A
                            }
                            \bussAssume{
                                \begin{array}{@{}l@{}}
                                    \vdash \begin{array}{@{}l@{}}
                                        Q \{ y/z \}
                                        \\
                                        \{ w'/w \}_{w \in \dom({?}\Delta)}
                                    \end{array}
                                    \\
                                    \typInf {?}\Delta', y:\ol{A}
                                \end{array}
                            }
                            \bussBin[\ruleLabel{typ-cut}]{
                                \begin{array}{@{}l@{}}
                                    \vdash \pRes{y} ( P \| Q \{ y/z \} \{ w'/w \}_{w \in \dom({?}\Delta)} )
                                    \\
                                    \typInf \Gamma, {?}\Delta'
                                \end{array}
                            }
                            \bussUn[\ruleLabel{typ-weaken}]{
                                \begin{array}{@{}l@{}}
                                    \vdash \pRes{y} ( P \| Q \{ y/z \} \{ w'/w \}_{w \in \dom({?}\Delta)} )
                                    \\
                                    \typInf \Gamma, {?}\Delta', x:{?}A
                                \end{array}
                            }
                            \bussAssume{
                                \vdash Q \typInf {?}\Delta , z:\ol{A}
                            }
                            \bussUn[\ruleLabel{typ-srv}]{
                                \vdash \pSrv x(z) ; Q \typInf {?}\Delta, x:{!}\ol{A}
                            }
                            \bussBin[\ruleLabel{typ-cut}]{
                                \vdash \pRes{x} ( \pRes{y} ( P \| Q \{ y/z \} \{ w'/w \}_{w \in \dom({?}\Delta)} ) \| \pSrv x(z) ; Q ) \typInf \Gamma, {?}\Delta, {?}\Delta'
                            }
                            \doubleLine
                            \bussUn[$\ruleLabel{typ-contract}^\ast$]{
                                \vdash \pRes{x} ( \pRes{y} ( P \| Q \{ y/z \} ) \| \pSrv x(z) ; Q ) \typInf \Gamma, {?}\Delta
                            }
                        \end{bussproof}
                    \end{mathpar}
            \end{itemize}
    \end{enumerate}
    The inductive cases follow straightforwardly.
    Notice that the conditions on the bound and free names of the ND-contexts in Items~\ref{i:clpi:reddEager:sendRecv} and~\ref{i:clpi:reddEager:cliSrv} make sure that no names are captured when embedding one context in the other.
\end{proof}

\begin{theorem}[SR for the Eager Semantics]
    \label{t:clpi:srEager}
    If $\vdash P \typInf \Gamma$ and $P \reddEager Q$, then $\vdash Q \typInf \Gamma$.
\end{theorem}

\begin{proof}
    By induction on the derivation of the reduction.
    In each case, we infer the typing of $P$ to derive the typing of $Q$.
    \begin{itemize}
        \item
            Rule~\ruleLabel{red-eager-fwd}.
            \begin{mathpar}
                \begin{bussproof}
                    \bussAssume{
                        \vdash \evalCtx[\big]{N}[\pFwd [x<>y]] \typInf \Gamma, x:A
                    }
                    \bussAssume{
                        \vdash Q \typInf \Delta, x:\ol{A}
                    }
                    \bussBin[\ruleLabel{typ-cut}]{
                        \vdash \pRes{x} ( \evalCtx[\big]{N}[\pFwd [x<>y]] \| Q ) \typInf \Gamma, \Delta
                    }
                \end{bussproof}
                \and
                \implies
                \and
                \begin{bussproof}
                    \bussAssume{
                        \text{(\refitem{l}{reddEager}{fwd})}
                    }
                    \noLine
                    \bussUn{
                        \vdash \evalCtx*{N}[Q \{ y/x \}] \typInf \Gamma, \Delta
                    }
                \end{bussproof}
            \end{mathpar}

        \item
            Rule~\ruleLabel{red-eager-close-wait}.
            \begin{mathpar}
                \begin{bussproof}
                    \bussAssume{
                        \text{(\refitem{l}{ctxType}{close})}
                    }
                    \noLine
                    \bussUn{
                        \vdash \evalCtx{N}[\pClose x[]] \typInf \Gamma, x:\1
                    }
                    \bussAssume{
                        \text{(\refitem{l}{ctxType}{wait})}
                    }
                    \noLine
                    \bussUn{
                        \vdash \evalCtx{N'}[\pWait x() ; Q] \typInf \Delta, x:\bot
                    }
                    \bussBin[\ruleLabel{typ-cut}]{
                        \vdash \nu{x} ( \evalCtx{N}[\pClose x[]] \| \evalCtx{N'}[\pWait x() ; Q] ) \typInf \Gamma, \Delta
                    }
                \end{bussproof}
                \and
                \implies
                \and
                \begin{bussproof}
                    \bussAssume{
                        \text{(\refitem{l}{reddEager}{close})}
                    }
                    \noLine
                    \bussUn{
                        \vdash \evalCtx{\D{N}}[\0] \typInf \Gamma
                    }
                    \bussAssume{
                        \text{(\refitem{l}{reddEager}{wait})}
                    }
                    \noLine
                    \bussUn{
                        \vdash \evalCtx{\D{N'}}[Q] \typInf \Delta
                    }
                    \bussBin[\ruleLabel{typ-par}]{
                        \vdash \evalCtx{\D{N}}[\0] \| \evalCtx{\D{N'}}[Q] \typInf \Gamma, \Delta
                    }
                \end{bussproof}
            \end{mathpar}

        \item
            Rule~\ruleLabel{red-eager-send-recv}.
            \begin{mathpar}
                \begin{bussproof}
                    \bussAssume{
                        \text{(\refitem{l}{ctxType}{send})}
                    }
                    \noLine
                    \bussUn{
                        \vdash \evalCtx{N}[\pOut* x[y] ; ( P \| Q )] \typInf \Gamma, x:A \tensor B
                    }
                    \bussAssume{
                        \text{(\refitem{l}{ctxType}{recv})}
                    }
                    \noLine
                    \bussUn{
                        \vdash \evalCtx{N'}[\pIn x(z) ; R] \vdash \Delta, x:\ol{A} \parr \ol{B}
                    }
                    \bussBin[\ruleLabel{typ-cut}]{
                        \vdash \pRes{x} ( \evalCtx{N}[\pOut* x[y] ; ( P \| Q )] \| \evalCtx{N'}[\pIn x(z) ; R] ) \typInf \Gamma, \Delta
                    }
                \end{bussproof}
                \and
                \implies
                \and
                \begin{bussproof}
                    \bussAssume{
                        \text{(\refitem{l}{reddEager}{sendRecv})}
                    }
                    \noLine
                    \bussUn{
                        \vdash \evalCtx{\D{N}}[\pRes{x} ( Q \| \nu{y} ( P \| \evalCtx{\D{N'}}[R \{ y/z \}] ) )] \typInf \Gamma, \Delta
                    }
                \end{bussproof}
            \end{mathpar}

        \item
            Rule~\ruleLabel{red-eager-sel-bra}.
            \begin{mathpar}
                \begin{bussproof}
                    \bussAssume{
                        \text{(\refitem{l}{ctxType}{sel})}
                    }
                    \bussAssume{
                        j \in I
                    }
                    \noLine
                    \bussBin{
                        \vdash \evalCtx{N}[\pSel* x < j ; P] \typInf \Gamma, x:\oplus \{ i : A_i \}_{i \in I}
                    }
                    \bussAssume{
                        \text{(\refitem{l}{ctxType}{bra})}
                    }
                    \noLine
                    \bussUn{
                        \evalCtx{N'}[\pBra* x > \{ i : Q_i \}_{i \in I}] \typInf \Delta, x:\& \{ i : \ol{A_i} \}_{i \in I}
                    }
                    \bussBin[\ruleLabel{typ-cut}]{
                        \vdash \pRes{x} ( \evalCtx{N}[\pSel* x < j ; P] \| \evalCtx{N'}[\pBra* x > \{ i : Q_i \}_{i \in I}] ) \typInf \Gamma, \Delta
                    }
                \end{bussproof}
                \and
                \implies
                \and
                \begin{bussproof}
                    \bussAssume{
                        \text{(\refitem{l}{reddEager}{sel})}
                    }
                    \noLine
                    \bussUn{
                        \vdash \evalCtx{\D{N}}[P] \typInf \Gamma, x:A_j
                    }
                    \bussAssume{
                        \text{(\refitem{l}{reddEager}{bra})}
                    }
                    \noLine
                    \bussUn{
                        \vdash \evalCtx{\D{N'}}[Q_j] \typInf \Delta, x:\ol{A_j}
                    }
                    \bussBin[\ruleLabel{typ-cut}]{
                        \vdash \pRes{x} ( \evalCtx{\D{N}}[P] \| \evalCtx{\D{N'}}[Q_j] ) \typInf \Gamma, \Delta
                    }
                \end{bussproof}
            \end{mathpar}

        \item
            Rule~\ruleLabel{red-eager-cli-srv}.
            \begin{mathpar}
                \begin{bussproof}
                    \bussAssume{
                        \text{(\refitem{l}{ctxType}{cli})}
                    }
                    \noLine
                    \bussUn{
                        \vdash \evalCtx{N}[\pCli* x[y] ; P] \typInf \Gamma, x:{?}A
                    }
                    \bussAssume{
                        \text{(\refitem{l}{ctxType}{srv})}
                    }
                    \noLine
                    \bussUn{
                        \vdash \evalCtx{N'}[\pSrv x(z) ; Q] \typInf \Delta, x:{!}\ol{A}
                    }
                    \bussBin[\ruleLabel{typ-cut}]{
                        \vdash \pRes{x} ( \evalCtx{N}[\pCli* x[y] ; P] \| \evalCtx{N'}[\pSrv x(y) ; Q]) \typInf \Gamma, \Delta
                    }
                \end{bussproof}
                \and
                \implies
                \and
                \begin{bussproof}
                    \bussAssume{
                        \text{(\refitem{l}{reddEager}{cliSrv})}
                    }
                    \noLine
                    \bussUn{
                        \vdash \evalCtx[\big]{\D{N'}}[\pRes{x} ( \pRes{y} ( \evalCtx{\D{N}}[P] \| Q \{ y/z \} ) \| \pSrv x(z) ; Q )] \typInf \Gamma, \Delta
                    }
                \end{bussproof}
            \end{mathpar}

        \item
            Rule~\ruleLabel{red-eager-some}.
            \begin{mathpar}
                \begin{bussproof}
                    \bussAssume{
                        \text{(\refitem{l}{ctxType}{some})}
                    }
                    \noLine
                    \bussUn{
                        \vdash \evalCtx{N}[\pSome x ; P] \typInf \Gamma, x:\& A
                    }
                    \bussAssume{
                        \text{(\refitem{l}{ctxType}{someIn})}
                    }
                    \noLine
                    \bussUn{
                        \vdash \evalCtx{N'}[\pSomeIn x{(w_1,\ldots,w_n)} ; Q] \typInf \Delta, x:\oplus \ol{A}
                    }
                    \bussBin[\ruleLabel{typ-cut}]{
                        \vdash \pRes{x} ( \evalCtx{N}[\pSome x ; P] \| \evalCtx{N'}[\pSomeIn x{(w_1,\ldots,w_n)} ; Q] ) \typInf \Gamma, \Delta
                    }
                \end{bussproof}
                \and
                \implies
                \and
                \begin{bussproof}
                    \bussAssume{
                        \text{(\refitem{l}{reddEager}{some})}
                    }
                    \noLine
                    \bussUn{
                        \vdash \evalCtx{\D{N}}[P] \typInf \Gamma, x:A
                    }
                    \bussAssume{
                        \text{(\refitem{l}{reddEager}{someIn})}
                    }
                    \noLine
                    \bussUn{
                        \vdash \evalCtx{\D{N'}}[Q] \typInf \Delta, x:\ol{A}
                    }
                    \bussBin[\ruleLabel{typ-cut}]{
                        \vdash \pRes{x} ( \evalCtx{\D{N}}[P] \| \evalCtx{\D{N'}}[Q] ) \typInf \Gamma, \Delta
                    }
                \end{bussproof}
            \end{mathpar}

        \item
            Rule~\ruleLabel{red-eager-none}.
            \begin{mathpar}
                \begin{bussproof}
                    \bussAssume{
                        \text{(\refitem{l}{ctxType}{none})}
                    }
                    \noLine
                    \bussUn{
                        \vdash \evalCtx{N}[\pNone x] \typInf \Gamma, x:\& A
                    }
                    \bussAssume{
                        \text{(\refitem{l}{ctxType}{someIn})}
                    }
                    \noLine
                    \bussUn{
                        \vdash \evalCtx{N'}[\pSomeIn x{(w_1,\ldots,w_n)} ; Q] \typInf \Delta, x:\oplus \ol{A}
                    }
                    \bussBin[\ruleLabel{typ-cut}]{
                        \vdash \pRes{x} ( \evalCtx{N}[\pNone x] \| \evalCtx{N'}[\pSomeIn x{(w_1,\ldots,w_n)} ; Q] ) \typInf \Gamma, \Delta
                    }
                \end{bussproof}
                \and
                \implies
                \and
                \begin{bussproof}
                    \bussAssume{
                        \text{(\refitem{l}{reddEager}{none})}
                    }
                    \noLine
                    \bussUn{
                        \vdash \evalCtx{\D{N}}[\0] \typInf \Gamma
                    }
                    \bussAssume{
                        \text{(\refitem{l}{reddEager}{someIn})}
                    }
                    \noLine
                    \bussUn{
                        \vdash \evalCtx{\D{N'}}[\pNone w_1 \| \ldots \| \pNone w_n] \typInf \Delta
                    }
                    \bussBin[\ruleLabel{typ-par}]{
                        \vdash \evalCtx{\D{N}}[\0] \| \evalCtx{\D{N'}}[\pNone w_1 \| \ldots \| \pNone w_n]) \typInf \Gamma, \Delta
                    }
                \end{bussproof}
            \end{mathpar}

        \item
            Rule~\ruleLabel{red-eager-cong}.
            Assume $P \equiv P'$ and $P' \reddEager Q'$ and $Q' \equiv Q$.
            By \Cref{t:clpi:sc}, $\vdash P' \typInf \Gamma$.
            By the IH, $\vdash Q' \typInf \Gamma$.
            By \Cref{t:clpi:sc}, $\vdash Q \typInf \Gamma$.

        \item
            Rule~\ruleLabel{red-eager-conn}.
            Assume $P \reddEager P'$.
            \begin{mathpar}
                \begin{bussproof}
                    \bussAssume{
                        \vdash P \typInf \Gamma, x:A
                    }
                    \bussAssume{
                        \vdash Q \typInf \Delta, x:\ol{A}
                    }
                    \bussBin[\ruleLabel{typ-cut}]{
                        \vdash \pRes{x} ( P \| Q ) \typInf \Gamma, \Delta
                    }
                \end{bussproof}
                \and
                \implies
                \and
                \begin{bussproof}
                    \bussAssume{
                        \text{(IH)}
                    }
                    \noLine
                    \bussUn{
                        \vdash P' \typInf \Gamma, x:A
                    }
                    \bussAssume{
                        \vdash Q \typInf \Delta, x:\ol{A}
                    }
                    \bussBin[\ruleLabel{typ-cut}]{
                        \vdash \pRes{x} ( P' \| Q ) \typInf \Gamma, \Delta
                    }
                \end{bussproof}
            \end{mathpar}

        \item
            Rule~\ruleLabel{red-eager-par}.
            Assume $P \reddEager P'$.
            \begin{mathpar}
                \begin{bussproof}
                    \bussAssume{
                        \vdash P \typInf \Gamma
                    }
                    \bussAssume{
                        \vdash Q \typInf \Delta
                    }
                    \bussBin[\ruleLabel{typ-par}]{
                        \vdash P \| Q \typInf \Gamma, \Delta
                    }
                \end{bussproof}
                \and
                \implies
                \and
                \begin{bussproof}
                    \bussAssume{
                        \text{(IH)}
                    }
                    \noLine
                    \bussUn{
                        \vdash P' \typInf \Gamma
                    }
                    \bussAssume{
                        \vdash Q \typInf \Delta
                    }
                    \bussBin[\ruleLabel{typ-par}]{
                        \vdash P' \| Q \typInf \Gamma, \Delta
                    }
                \end{bussproof}
            \end{mathpar}

        \item
            Rule~\ruleLabel{red-eager-nd}.
            Assume $P \reddEager P'$.
            \begin{mathpar}
                \begin{bussproof}
                    \bussAssume{
                        \vdash P \typInf \Gamma
                    }
                    \bussAssume{
                        \vdash Q \typInf \Gamma
                    }
                    \bussBin[\ruleLabel{typ-nd}]{
                        \vdash P \nd Q \typInf \Gamma
                    }
                \end{bussproof}
                \and
                \implies
                \and
                \begin{bussproof}
                    \bussAssume{
                        \text{(IH)}
                    }
                    \noLine
                    \bussUn{
                        \vdash P' \typInf \Gamma
                    }
                    \bussAssume{
                        \vdash Q \typInf \Gamma
                    }
                    \bussBin[\ruleLabel{typ-nd}]{
                        \vdash P' \nd Q \typInf \Gamma
                    }
                \end{bussproof}
                \and
                \qedhere
            \end{mathpar}
    \end{itemize}
\end{proof}
%</clpi:tp:srEager>

\subsubsection{Deadlock-freedom}

The proof uses several definitions and lemmas, which we summarize:
\begin{itemize}
    \item
        \Cref{d:sctx} defines single-choice multi-hole contexts, where holes may only appear on one side of non-deterministic choices.
        \Cref{d:scoll} yields deterministic multi-hole contexts from single-choice multi-hole contexts by committing non-deterministic choices to the sides of holes.
        \Cref{l:scoll} ensures typing remains consistent when committing a single-choice multi-hole context.

    \item
        \Cref{l:sctxform} states that any typable process not equivalent to $\0$ can be written as an S-context with each hole replaced by a prefixed process.
        Let us refer to this as the \emph{S-context form}.

    \item
        \Cref{l:sformfwd} states that if a process in S-context form is typable under empty context and has a forwarder as one of its prefixes, that process contains a cut on one of the forwarder's subjects.

    \item
        \Cref{l:sctxcuts} states that the number of prefixed processes of a process in S-context form is at least the number of cuts in the S-context.
        This lemma is key to the proof of Deadlock Freedom, as it is necessary to show the next lemma.

    \item
        \Cref{l:sctxsubjs} states that if a process in S-context form is typable under empty context, then there must be two of its prefixed processes that share a subject.
\end{itemize}

\begin{definition}[Single-choice Multi-hole Contexts]\label{d:sctx}
    We define \emph{single-choice multi-hole contexts} (S-contexts, for short) as follows:
    \[
        \evalCtx{S} ::= {\evalHole}_i \sepr \pRes{x} (\evalCtx{S} \| \evalCtx{S}) \sepr \evalCtx{S} \| \evalCtx{S} \sepr \evalCtx{S} \nd P
    \]
    An S-context is $n$-ary if it has $n$ holes ${\evalHole}_1, \ldots, {\evalHole}_n$.
    We write $\evalCtx{S}[P_1, \ldots, P_n]$ to denote the process obtained from the $n$-ary multi-hole context $\evalCtx{S}$ by replacing each $i$-th hole in $\evalCtx{S}$ with $P_i$.
    Given an S-context $\evalCtx{S}$ with hole indices $I$ and a sequence of processes ${(P_i)}_{i \in I}$, we write $\evalCtx{S}[P_i]_{i \in I}$ to denote the process obtained from $\evalCtx{S}$ by replacing each hole with index $i$ in $\evalCtx{S}$ with $P_i$.
    We say an S-context is a \emph{deterministic multi-hole context} (DM-context, for short) if its holes do not appear inside any non-deterministic choices.
\end{definition}

\begin{definition}[Commitment of Single-choice Multi-hole Contexts]\label{d:scoll}
    We define the \emph{commitment} of S-context $\evalCtx{S}$, by abuse of notation denoted $\D{\evalCtx{S}}$ (cf.\ \Cref{s:disc}), as follows, yielding a deterministic multi-hole context:
    \begin{align*}
        \D{{\evalHole}_i} &\deq {\evalHole}_i
        & \D{\evalCtx{S} \| \evalCtx{S}'} &\deq \D{\evalCtx{S}} \| \D{\evalCtx{S}'}
        & \D{\pRes{x} (\evalCtx{S} \| \evalCtx{S}')} &\deq \pRes{x} (\D{\evalCtx{S}} \| \D{\evalCtx{S}'})
        & \D{\evalCtx{S} \nd P} &\deq \D{\evalCtx{S}}
    \end{align*}
\end{definition}

\begin{lemma}\label{l:scoll}
    If $\evalCtx{S}[P_i]_{i \in I} \vdash \Gamma$, then $\D{\evalCtx{S}}[P_i]_{i \in I} \vdash \Gamma$.
\end{lemma}

\begin{proof}
    Straightforward, by induction on the structure of $\evalCtx{S}$.
\end{proof}

\begin{lemma}\label{l:sctxform}
    If $P \vdash \Gamma$ and $P \not\equiv \0$, then there exist S-context $\evalCtx{S}$ with indices $I$ and sequence of prefixed processes ${(\alpha_i;P_i)}_{i \in I}$ such that $P \equiv \evalCtx{S}[\alpha_i;P_i]_{i \in I}$.
\end{lemma}

\begin{proof}
    Using structural congruence, we first remove all cuts with unused servers and parallel compositions with $\0$, obtaining $P' \equiv P$.
    Since $P \not\equiv \0$, $P' \not\equiv \0$.
    Then, we construct $\evalCtx{S}$ by induction on the typing derivation of $P'$.
    Rules \ttype{empty} and \ttype{weaken} do not occur, because of how we obtained $P'$ from $P$.
    The structural rules \ttype{mix}, \ttype{cut}, and \ttype{weaken} are simply copied.
    In case of rule \ttype{$\nd$}, we arbitrarily pick a branch to continue the construction of $\evalCtx{S}$ with, while copying the entire other branch.
    The other rules, which type prefixes, add a hole to $\evalCtx{S}$; we mark the hole with index $i$ and refer to the prefixed process typed by the rule as $\alpha_i;P_i$.
    Clearly, $P \equiv P' = \evalCtx{S}[\alpha_i;P_i]_{i \in I}$.
\end{proof}

\begin{lemma}\label{l:sformfwd}
    If $P = \evalCtx{S}[\alpha_i;P_i]_{i \in I} \vdash \emptyset$ and there is $j \in I$ s.t.\ $\alpha_j = \pFwd [x<>y]$, then there are $\evalCtx{N},\evalCtx{N'},Q$ such that $P = \evalCtx[\Big]{N}[\pRes{x} (\evalCtx[\big]{N'}[\pFwd [x<>y]] \| Q)]$.
\end{lemma}

\begin{proof}
    Note that there must be a restriction on $x$ in $P$, because $x$ appears free in $\pFwd [x<>y]$ but $P \vdash \emptyset$.
    First, we obtain $\evalCtx{N}$ from $P$ by replacing the restriction on $x$ in $P$ with a hole, referring the parallel component in which $\pFwd [x<>y]$ appears as $P'$ and the other parallel component as $Q$.
    Then, we obtain $\evalCtx{N'}$ from $P'$ by replacing $\pFwd [x<>y]$ with a hole.
    Clearly, $P = \evalCtx[\Big]{N}[\pRes{x} (\evalCtx[\big]{N'}[\pFwd [x<>y]] \| Q)]$.
\end{proof}

\begin{lemma}\label{l:sctxcuts}
    If the derivation of $P = \evalCtx{S}[\alpha_i;P_i]_{i \in I} \vdash \Gamma$ and $\evalCtx{S}$ is deterministic and contains $n$ cuts, then $|I| \geq n+1$.
\end{lemma}

\begin{proof}
    We apply strong induction on the number $n$ of cuts in $\evalCtx{S}$:
    \begin{itemize}
        \item
            Case $n = 0$.
            Any S-context must have at least one hole, so $\evalCtx{S}$ has at least one hole.
            Hence, $|I| \geq 1 = n + 1$.

        \item
            Case $n = n' + 1$.
            By abuse of notation, $P = P_1 \| \ldots \| P_k$, where for each $1 \leq k' \leq k$, $P_{k'}$ is not a parallel composition.
            By assumption, $m \geq 1$ of the $P_1,\ldots,P_k$ are cuts.
            W.l.o.g., assume $P_1,\ldots,P_m$ are cuts.

            For each $1 \leq j \leq m$, by inversion of rule \ttype{mix}, $P_j \vdash \Gamma_j$, and by construction, there are $\evalCtx{S_j},I_j$ s.t.\ $P_j = \evalCtx{S_j}[\alpha_i;P_i]_{i \in I_j}$ where $\evalCtx{S_j}$ is deterministic.
            We have for each $1 \leq j \leq m$ and $1 \leq j' \leq m$ where $j \neq j'$ that $I_j \cap I_{j'} = \emptyset$, and $\bigcup_{1 \leq j \leq m} I_j \subseteq I$.
            Then, for each $1 \leq j \leq m$, let $1 \leq n_j \leq n$ be the number of cuts in $\evalCtx{S_j}$.
            Since $P_{m+1},\ldots,P_k$ are not cuts, we have $\sum_{1 \leq j \leq m} n_j = n$.

            Take any $1 \leq j \leq m$.
            We have $P_j = \pRes{x} (P'_j \| P''_j)$, and by inversion of rule \ttype{cut}, $P'_j \vdash \Gamma'_j, x{:}A$ and $P''_j \vdash \Gamma''_j, x{:}\ol{A}$ where $\Gamma_j = \Gamma'_j, \Gamma''_j$.
            By construction, there are $\evalCtx{S'_j},\evalCtx{S''_j},I'_j,I''_j$ s.t.\ $P'_j = \evalCtx{S'_j}[\alpha_i;P_i]_{i \in I'_j}$ and $P''_j = \evalCtx{S''_j}[\alpha_i;P_i]_{i \in I''_j}$ and $\evalCtx{S'_j}$ and $\evalCtx{S''_j}$ are deterministic.
            We have $I'_j \cap I''_j = \emptyset$ and $I'_j \cup I''_j = I_j$.

            Let $n'_j$ and $n''_j$ be the number of cuts in $\evalCtx{S'_j}$ and $\evalCtx{S''_j}$, respectively.
            We have that $n'_j + n''_j + 1 = n_j$.
            Since $n_j \leq n = n' + 1$, then $n'_j,n''_j \leq n'$.
            Then, by the IH, $|I'_j| \geq n'_j + 1$ and $|I''_j| \geq n''_j + 1$.
            Therefore, $|I_j| = |I'_j \cup I''_j| = |I'_j| + |I''_j| \geq n'_j + n''_j + 1 + 1 = n_j + 1$.

            In conclusion,
            \begin{align*}
                |I| \geq |\bigcup_{1 \leq j \leq m} I_j| = \sum_{1 \leq j \leq m} |I_j| \geq \sum_{1 \leq j \leq m} (n_j + 1) = \sum_{1 \leq j \leq m} n_j + m = n + m \geq n + 1.
                \tag*{\qedhere}
            \end{align*}
    \end{itemize}
\end{proof}

\begin{lemma}\label{l:sctxsubjs}
    If $P = \evalCtx{S}[\alpha_i;P_i]_{i \in I} \vdash \emptyset$ where for each $i \in I$, $\alpha_i \neq \pFwd [x<>y]$ for any $x$ and $y$, then there are $j,k \in I$ where $j \neq k$ and $x = \subj(\alpha_j) = \subj(\alpha_k)$, and there are $\evalCtx{N},\evalCtx{N_j},\evalCtx{N_k}$ such that $P = \evalCtx[\big]{N}[\pRes{x} (\evalCtx{N_j}[\alpha_j] \| \evalCtx{N_k}[\alpha_k])]$.
\end{lemma}

\begin{proof}
    Let $Q = \evalCtx*{S}[{(\alpha_i)}_{i \in I}]$.
    Then $Q$ is deterministic and, by \Cref{l:scoll}, $Q \vdash \emptyset$.
    Let $n$ be the number of cuts in $\evalCtx{S}$.
    By \Cref{l:sctxcuts}, $|I| \geq n + 1$.

    Suppose, for contradiction, that for every $j,k \in I$ where $j \neq k$, we have $\subj(\alpha_j) \neq \subj(\alpha_k)$.
    Since $Q \vdash \emptyset$, for each $j \in I$, $\subj(\alpha_j)$ must be bound by a cut, so $\evalCtx{S}$ must contain $|I|$ cuts.
    This means $|I| = n$, contradicting the fact that $|I| \geq n + 1$.
    Therefore, there must be $j,k \in I$ where $j \neq k$ such that $\subj(\alpha_j) = \subj(\alpha_k)$.

    Hence, we can take $x = \subj(\alpha_j) = \subj(\alpha_k)$.
    Since $P \vdash \emptyset$ but $x$ appears free in $\alpha_j;P_j$ and $\alpha_k;P_k$, there must be a restriction on $x$ in $\evalCtx{S}$ containing the holes ${\evalHole}_j$ and ${\evalHole}_k$.
    We now obtain $\evalCtx{N}$ from $P$ by replacing the restriction on $x$ in $P$ with a hole, referring to the parallel component in which $\alpha_j;P_j$ appears as $P_j$ and the component in which $\alpha_k;P_k$ appears as $P_k$.
    Then, we obtain $\evalCtx{N_j}$ and $\evalCtx{N_k}$ from $P_j$ and $P_k$, respectively, by replacing $\alpha_j;P_j$ and $\alpha_k;P_k$ with a hole.
    Clearly, $P = \evalCtx[\big]{N}[\pRes{x} (\evalCtx{N_j}[\alpha_j;P_j] \| \evalCtx{N_k}[\alpha_k;P_k])]$.
\end{proof}

\thmDlfreeOne*

\begin{proof}
    By \Cref{l:sctxform}, there are S-context $\evalCtx{S}$ with hole indices $I$ and sequence of prefixed processes ${(\alpha_i;P_i)}_{i \in I}$ such that $P \equiv \evalCtx{S}[\alpha_i;P_i]_{i \in I}$.
    The next step depends on whether there is a forwarder process among the $\alpha_i$.
    \begin{itemize}
        \item
            If there exists $j \in I$ s.t.\ $\alpha_j = \pFwd [x<>y]$ for some $x$ and $y$, then by \Cref{l:sformfwd} there are $\evalCtx{N},\evalCtx{N'},Q$ s.t.\ $\evalCtx{S}[\alpha_i;P_i] = \evalCtx[\Big]{N}[\pRes{x} (\evalCtx[\big]{N'}[\pFwd [x<>y]] \| Q)]$.
            \begin{align*}
                \pRes{x} (\evalCtx[\big]{N'}[\pFwd [x<>y]] \| Q) &\reddEager \evalCtx*{N'}[Q\{y/x\}] = R'
                &&\text{(by rule $\rredone{\scc{Id}}$)}
                \\
                \evalCtx{S}[\alpha_i;P_i]_{i \in I} = \evalCtx[\Big]{N}[\pRes{x} (\evalCtx[\big]{N'}[\pFwd [x<>y]] \| Q)] &\reddEager \evalCtx{N}[R'] = R
                &&\text{(by rules $\rredone{\nu},\rredone{\|},\rredone{\nd}$)}
                \\
                P &\reddEager R
                &&\text{(by rule $\rredone{\equiv}$)}
            \end{align*}

        \item
            If for each $i \in I$, $\alpha_i \neq x \fwd y$ for any $x$ and $y$, then by \Cref{l:sctxsubjs} there are $j,k \in I$ where $j \neq k$ and $x = \subj(\alpha_j) = \subj(\alpha_k)$ for some $x$, and $\evalCtx{N},\evalCtx{N_j},\evalCtx{N_k}$ such that $\evalCtx{S}[\alpha_i;P_i]_{i \in I} = \evalCtx[\big]{N}[\pRes{x} (\evalCtx{N_j}[\alpha_j;P_j] \| \evalCtx{N_k}[\alpha_k;P_k])]$.

            We now show by cases on $\alpha_j$ that there is $R'$ such that $\pRes{x} (\evalCtx{N_j}[\alpha_j;P_j] \| \evalCtx{N_k}[\alpha_k;P_k]) \reddEager R'$.
            First, note that by typability, if the type for $x$ in $\evalCtx{N_j}[\alpha_j;P_j]$ is $A$, then the type for $x$ in $\evalCtx{N_k}[\alpha_k;P_k]$ is $\ol{A}$.
            In the following cases, we determine more precisely the form of $A$ by typing inversion on $\evalCtx{N_j}[\alpha_j;P_j]$, and then determine the form of $\alpha_k$ by typing inversion using the form of $\ol{A}$.
            Note that we can exclude any cases where $\alpha_j$ or $\alpha_k$ are forwarder processes, as we assume they are not.
            \begin{itemize}
                \item
                    If $\alpha_j;P_j = \pClose x[]$, then $A = \1$ and $\ol{A} = \bot$.
                    Hence, $\alpha_k;P_k = \pWait x();P_k$.
                    By rule $\rredone{\1\bot}$, there is $R'$ such that
                    \begin{align*}
                        \pRes{x} (\evalCtx{N_j}[\pClose x[]] \| \evalCtx{N_k}[\pWait x();P_k]) \reddEager R'.
                    \end{align*}
                \item
                    If $\alpha_j;P_j = \pOut* x[y];(P'_j \| P''_j)$ for some $y$, then $A = B \tensor C$ and $\ol{A} = \ol{B} \parr \ol{C}$ for some $B$ and $C$.
                    Hence, $\alpha_k;P_k = \pIn x(z); P_k$ for some $z$.
                    By rule $\rredone{\tensor\parr}$, there is $R'$ such that
                    \begin{align*}
                        \pRes{x} (\evalCtx{N_j}[\pOut* x[y];(P'_j \| P''_j)] \| \evalCtx{N_k}[\pIn x(z);P_k]) \reddEager R'.
                    \end{align*}

                \item
                    If $\alpha_j;P_j = \pSel* x < l'; P_j$, then $A = \oplus \{l:B_l\}_{l \in L}$ and $\ol{A} = \&\{l:\ol{B_l}\}_{l \in L}$ for some ${(B_l)}_{l \in L}$ where $l' \in L$.
                    Hence, $\alpha_k;P_k = \pBra* x >\{l:P_k^l\}_{l \in L}$.
                    By rule $\rredone{\oplus\\&}$, there is $R'$ such that
                    \begin{align*}
                        \pRes{x} (\evalCtx{N_j}[\pSel* x < l'; P_j] \| \evalCtx{N_k}[\pBra* x >\{l:P_k^l\}_{l \in L}]) \reddEager R'.
                    \end{align*}

                \item
                    If $\alpha_j;P_j = \pSome x; P_j$, then $A = \oplus B$ and $\ol{A} = \&\ol{B}$ for some $B$.
                    Hence, $\alpha_k = \pSomeIn x{w_1,\ldots,w_n}; P_k$ for some $w_1,\ldots,w_n$.
                    By rule $\rredone{\some}$, there is $R'$ such that
                    \begin{align*}
                        \pRes{x} (\evalCtx{N_j}[\pSome x; P_j] \| \evalCtx{N_k}[\pSomeIn x{w_1,\ldots,w_n}; P_k]) \reddEager R'.
                    \end{align*}

                \item
                    If $\alpha_j;P_j = \pNone x$, then $A = \oplus B$ and $\ol{A} = \&\ol{B}$ for some $B$.
                    Hence, $\alpha_k = \pSomeIn x{w_1,\ldots,w_n}; P_k$ for some $w_1,\ldots,w_n$.
                    By rule $\rredone{\none}$, there is $R'$ such that
                    \begin{align*}
                        \pRes{x} (\evalCtx{N_j}[\pNone x] \| \evalCtx{N_k}[\pSomeIn x{w_1,\ldots,w_n}; P_k]) \reddEager R'.
                    \end{align*}

                \item
                    If $\alpha_j;P_j = \pCli* x[y]; P_j$ for some $y$, then $A = {?}B$ and $\ol{A} = {!}\ol{B}$ for some $B$.
                    Hence, $\alpha_k;P_k = \pSrv x(z); P_k$ for some $z$.
                    By rule $\rredone{{?}{!}}$, there is $R'$ such that
                    \begin{align*}
                        \pRes{x} (\evalCtx{N_j}[\pCli* x[y]; P_j] \| \evalCtx{N_k}[\pSrv x(z); P_k]) \reddEager R'.
                    \end{align*}

                \item
                    Otherwise, $\alpha_j$ is a receiving prefix and $\alpha_k$ is thus a sending prefix.
                    By cases on $\alpha_k$, the proof is analogous to above.
            \end{itemize}
            In conclusion,
            \begin{align*}
                \evalCtx{S}[\alpha_i;P_i]_{i \in I} = \evalCtx[\big]{N}[\pRes{x} (\evalCtx{N_j}[\alpha_j;P_j] \| \evalCtx{N_k}[\alpha_k;P_k])] &\reddEager \evalCtx{N}[R'] = R
                &&\text{(by rules $\rredone{\nu},\rredone{\|},\rredone{\nd}$)}
                \\
                P &\reddEager R.
                &&\text{(by rule $\rredone{\equiv}$)}
                \tag*{\qedhere}
            \end{align*}
    \end{itemize}
\end{proof}

\subsection{Lazy Semantics}
\label{ss:proofsLazy}

\subsubsection{Subject Reduction}
\label{ss:TPLazy}

%<*clpi:tp:srLazy>
\begin{lemma}
    \label{l:clpi:reddLazy}
    For both of the following items, assume $\Gamma \cap \Delta = \emptyset$.
    \begin{enumerate}

        \item\label{i:clpi:reddLazy:sendRecv}
            If $\forall i \in I.~ \forall j \in J.~ \bn(\evalCtx{C_i}) \cap \fn(\evalCtx{D_j}) = \emptyset$ and $\forall i \in I.~ \vdash \evalCtx{C_i}[\pOut* x[y_i] ; ( P_i \| Q_i )] \typInf \Gamma, x:A \tensor B$ and $\forall j \in J.~ \vdash \evalCtx{D_j}[\pIn x(z) ; R_j] \typInf \Delta, x:\ol{A} \parr \ol{B}$, then 
            \[
                \vdash \bignd_{i \in I} \evalCtx[\big]{C_i}[\pRes{x} \big( Q_i \| \pRes{w} (P_i \{ w/y_i \} \| \bignd_{j \in J} \evalCtx{D_j}[R_j \{ w/z \}]) \big)] \typInf \Gamma, \Delta.
            \]

        \item\label{i:clpi:reddLazy:cliSrv}
            If $\forall i \in I.~ \forall j \in J.~ \bn(\evalCtx{D_j}) \cap \fn(\evalCtx{C_i}) = \emptyset$ and $\forall i \in I.~ \vdash \evalCtx{C_i}[\pCli* x[y_i] ; P_i] \typInf \Gamma, x:{?}A$ and \mbox{$\forall j \in J.~ \vdash \evalCtx{D_j}[\pSrv x(z) ; Q_j] \typInf \Delta, x:{!}\ol{A}$}, then 
            \[
                \bignd_{j \in J} \evalCtx[\big]{D_j}[\pRes{x} \big( \pRes{w} ( \bignd_{i \in I} \evalCtx{C_i}[P_i \{ w/y_i \}] \| Q_j \{ w/z \} ) \| \pSrv x(z) ; Q_j \big)] \typInf \Gamma, \Delta.
            \]

    \end{enumerate}
\end{lemma}

\begin{proof}
    Both items follow by induction on the structures of the D-contexts.
    For each item, we detail the base case, where $\forall i \in I.~ \evalCtx{C_i} = \evalHole$ and $\forall j \in J.~ \evalCtx{D_j} = \evalHole$.
    The inductive cases follow from the IH straightforwardly.
    \begin{enumerate}

        \item
            \begin{mathpar}
                \forall i \in I.~
                \begin{bussproof}
                    \bussAssume{
                        \vdash P_i \typInf \Gamma, y_i:A
                    }
                    \bussAssume{
                        \vdash Q_i \typInf \Delta, x:B
                    }
                    \bussBin[\ruleLabel{typ-send}]{
                        \vdash \pOut* x[y_i] ; ( P_i \| Q_i ) \typInf \Gamma, \Delta, x{:}A \tensor B
                    }
                \end{bussproof}
                \and
                \land
                \and
                \forall j \in J.~
                \begin{bussproof}
                    \bussAssume{
                        \vdash R_j \typInf \Lambda, z:\ol{A}, x:\ol{B}
                    }
                    \bussUn[\ruleLabel{typ-recv}]{
                        \vdash \pIn x(z) ; R_j \typInf \Lambda, x:\ol{A} \parr \ol{B}
                    }
                \end{bussproof}
                \and
                \implies
                \and
                \begin{bussproof}
                    \bussAssume{
                        \begin{array}{@{}l@{}}
                            \forall i \in I. \\
                            \vdash Q_i \typInf \Delta, x:B
                        \end{array}
                    }
                    \bussAssume{
                        \forall i \in I.~
                        \begin{array}[t]{@{}l@{}}
                            \vdash P_i \{ w/y_i \}
                            \\
                            \typInf \Gamma, w:A
                        \end{array}
                    }
                    \bussAssume{
                        \forall j \in J.~
                        \begin{array}[t]{@{}l@{}}
                            \vdash R_j \{ w/z \}
                            \\
                            \typInf \Lambda, w:\ol{A}, x:\ol{B}
                        \end{array}
                    }
                    \doubleLine
                    \bussUn[$\ruleLabel{typ-nd}^\ast$]{
                        \begin{array}{@{}l@{}}
                            \vdash \bignd_{j \in J} R_j \{ w/z \}
                            \typInf \Lambda, w:\ol{A}, x:\ol{B}
                        \end{array}
                    }
                    \bussBin[\ruleLabel{typ-cut}]{
                        \forall i \in I.~
                        \vdash \pRes{w} ( P_i \{ w/y_i \} \| \bignd_{j \in J} R_j \{ w/z \} ) \typInf \Gamma, \Lambda, x:\ol{B}
                    }
                    \bussBin[\ruleLabel{typ-cut}]{
                        \forall i \in I.~
                        \pRes{x} \big( Q_i \| \pRes{w} ( P_i \{ w/y_i \} \| \bignd_{j \in J} R_j \{ w/z \} ) \big) \typInf \Gamma, \Delta, \Lambda
                    }
                    \doubleLine
                    \bussUn[$\ruleLabel{typ-nd}^\ast$]{
                        \vdash \bignd_{i \in I} \pRes{x} \big( Q_i \| \pRes{w} ( P_i \{ w/y_i \} \| \bignd_{j \in J} R_j \{ w/z \} ) \big) \typInf \Gamma, \Delta, \Lambda
                    }
                \end{bussproof}
            \end{mathpar}

        \item
            This item depends on whether $x \in \fn(P_i)$ or not, for each $i \in I$.
            W.l.o.g., we only consider the cases where either $\forall i \in I.~ x \in \fn(P_i)$ or $\forall i \in I.~ x \notin \fn(P_i)$.
            \begin{itemize}

                \item
                    Case $\forall i \in I.~ x \in \fn(P_i)$.
                    \begin{mathpar}
                        \forall i \in I.~
                        \begin{bussproof}
                            \bussAssume{
                                \vdash P_i \{ x'/x \} \typInf \Gamma, y_i:A, x':{?}A
                            }
                            \bussUn[\ruleLabel{typ-cli}]{
                                \vdash \pCli* x[y_i] ; P_i \{ x'/x \} \typInf \Gamma, x:{?}A, x':{?}A
                            }
                            \bussUn[\ruleLabel{typ-contract}]{
                                \vdash \pCli* x[y_i] ; P_i \typInf \Gamma, x:{?}A
                            }
                        \end{bussproof}
                        \and
                        \land
                        \and
                        \forall j \in J.~
                        \begin{bussproof}
                            \bussAssume{
                                \vdash Q_j \typInf {?}\Delta, x:\ol{A}
                            }
                            \bussUn[\ruleLabel{typ-serv}]{
                                \vdash \pSrv x(z) ; Q_j \typInf {?}\Delta, x:{!}\ol{A}
                            }
                        \end{bussproof}
                        \and
                        \implies
                        \and
                        \begin{bussproof}
                            \bussAssume{
                                \begin{array}[t]{@{}l@{}}
                                    \forall i \in I.
                                    \\
                                    \vdash P_i \{ w/y_i \}
                                    \\
                                    \typInf \Gamma, w:A, x:{?}A
                                \end{array}
                            }
                            \doubleLine
                            \bussUn[$\ruleLabel{typ-nd}^\ast$]{
                                \begin{array}{@{}l@{}}
                                    \vdash \bignd_{i \in I} P_i \{ w/y_i \}
                                    \\
                                    \typInf \Gamma, w:A, x:{?}A
                                \end{array}
                            }
                            \bussAssume{
                                \begin{array}{@{}l@{}}
                                    \forall j \in J.
                                    \\
                                    \vdash \begin{array}[t]{@{}l@{}}
                                        Q_j \{ w/z \} \\
                                        \{ v'/v \}_{v \in \dom({?}\Delta)}
                                    \end{array}
                                    \\
                                    \typInf {?}\Delta', w:\ol{A}
                                \end{array}
                            }
                            \bussBin[\ruleLabel{typ-cut}]{
                                \begin{array}{@{}l@{}}
                                    \forall j \in J.
                                    \\
                                    \vdash \pRes{w} \begin{array}[t]{@{}l@{}}
                                        ( \bignd_{i \in I} P_i \{ w/y_i \}
                                        \\
                                        {} \| Q_j \{ w/z \} \{ v'/v \}_{v \in \dom({?}\Delta)} )
                                    \end{array}
                                    \\
                                    \typInf \Gamma, {?}\Delta', x:{?}A
                                \end{array}
                            }
                            \bussAssume{
                                \begin{array}{@{}l@{}}
                                    \forall j \in J.
                                    \\
                                    \vdash Q_j \\
                                    \typInf {?}\Delta, x:\ol{A}
                                \end{array}
                            }
                            \bussUn[\ruleLabel{typ-serv}]{
                                \begin{array}{@{}l@{}}
                                    \forall j \in J.
                                    \\
                                    \vdash \pSrv x(z) ; Q_j \\
                                    \typInf {?}\Delta, x:{!}\ol{A}
                                \end{array}
                            }
                            \bussBin[\ruleLabel{typ-cut}]{
                                \begin{array}{@{}l@{}}
                                    \forall j \in J. \\
                                    \vdash \pRes{x} \big( \pRes{w} ( \bignd_{i \in I} P_i \{ w/y_i \} \| Q_j \{ w/z \} \{ v'/v \}_{v \in \dom({?}\Delta)} ) \| \pSrv x(z) ; Q_j \big) \\
                                    \typInf \Gamma, {?}\Delta, {?}\Delta'
                                \end{array}
                            }
                            \doubleLine
                            \bussUn[$\ruleLabel{typ-nd}^\ast$]{
                                \begin{array}{@{}l@{}}
                                    \vdash \bignd_{j \in J} \pRes{x} \big( \begin{array}[t]{@{}l@{}}
                                        \pRes{w} ( \bignd_{i \in I} P_i \{ w/y_i \} \| Q_j \{ w/z \} \{ v'/v \}_{v \in \dom({?}\Delta)} ) \\
                                        {} \| \pSrv x(z) ; Q_j \big)
                                    \end{array} \\
                                    \typInf \Gamma, {?}\Delta, {?}\Delta'
                                \end{array}
                            }
                            \doubleLine
                            \bussUn[$\ruleLabel{typ-contract}^\ast$]{
                                \vdash \bignd_{j \in J} \pRes{x} \big( \pRes{w} ( \bignd_{i \in I} P_i \{ w/y_i \} \| Q_j \{ w/z \} \big) \| \pSrv x(z) ; Q_j ) \typInf \Gamma, {?}\Delta
                            }
                        \end{bussproof}
                    \end{mathpar}

                \item
                    Case $\forall i \in I.~ x \notin \fn(P_i)$.
                    \begin{mathpar}
                        \forall i \in I.~
                        \begin{bussproof}
                            \bussAssume{
                                \vdash P_i \typInf \Gamma, y_i:A
                            }
                            \bussUn[\ruleLabel{typ-cli}]{
                                \vdash \pCli* x[y_i] ; P_i \vdash \Gamma, x:{?}A
                            }
                        \end{bussproof}
                        \and
                        \land
                        \and
                        \forall j \in J.~
                        \begin{bussproof}
                            \bussAssume{
                                \vdash Q_j \typInf {?}\Delta, x:\ol{A}
                            }
                            \bussUn[\ruleLabel{typ-srv}]{
                                \vdash \pSrv x(z) ; Q_j \typInf {?}\Delta, x:{!}\ol{A}
                            }
                        \end{bussproof}
                        \and
                        \implies
                        \and
                        \begin{bussproof}
                            \bussAssume{
                                \begin{array}{@{}l@{}}
                                    \forall i \in I.
                                    \\
                                    \vdash P_i \{ w/y_i \}
                                    \\
                                    \typInf \Gamma, w:A
                                \end{array}
                            }
                            \doubleLine
                            \bussUn[$\ruleLabel{typ-nd}^\ast$]{
                                \begin{array}{@{}l@{}}
                                    \vdash \bignd_{i \in I} P_i \{ w/y_i \}
                                    \\
                                    \typInf \Gamma, w:A
                                \end{array}
                            }
                            \bussAssume{
                                \begin{array}{@{}l@{}}
                                    \forall j \in J.
                                    \\
                                    \vdash \begin{array}{@{}l@{}}
                                        Q_j \{ w/z \} \\
                                        \{ v'/v \}_{v \in \dom({?}\Delta)}
                                    \end{array}
                                    \\
                                    \typInf {?}\Delta', w:\ol{A}
                                \end{array}
                            }
                            \bussBin[\ruleLabel{typ-cut}]{
                                \begin{array}{@{}l@{}}
                                    \forall j \in J.
                                    \\
                                    \vdash \pRes{w} \begin{array}[t]{@{}l@{}}
                                        ( \bignd_{i \in I} P_i \{ w/y_i \}
                                        \\
                                        {} \| Q_j \{ w/z \} \{ v'/v \}_{v \in \dom({?}\Delta)} ) \typInf \Gamma, {?}\Delta'
                                    \end{array}
                                \end{array}
                            }
                            \bussUn[\ruleLabel{typ-weaken}]{
                                \begin{array}{@{}l@{}}
                                    \forall j \in J.
                                    \\
                                    \vdash \pRes{w} \begin{array}[t]{@{}l@{}}
                                        ( \bignd_{i \in I} P_i \{ w/y_i \}
                                        \\
                                        {} \| Q_j \{ w/z \} \{ v'/v \}_{v \in \dom({?}\Delta)} ) \typInf \Gamma, {?}\Delta', x:{?}A
                                    \end{array}
                                \end{array}
                            }
                            \bussAssume{
                                \begin{array}{@{}l@{}}
                                    \forall j \in J.
                                    \\
                                    \vdash Q_j \\
                                    \typInf {?}\Delta , z:\ol{A}
                                \end{array}
                            }
                            \bussUn[\ruleLabel{typ-srv}]{
                                \begin{array}{@{}l@{}}
                                    \forall j \in J.
                                    \\
                                    \vdash \pSrv x(z) ; Q_j \\
                                    \typInf {?}\Delta, x:{!}\ol{A}
                                \end{array}
                            }
                            \bussBin[\ruleLabel{typ-cut}]{
                                \begin{array}{@{}l@{}}
                                    \forall j \in J. \\
                                    \vdash \pRes{x} \big( \pRes{w} ( \bignd_{i \in I} P_i \{ w/y_i \} \| Q_j \{ w/z \} \{ v'/v \}_{v \in \dom({?}\Delta)} ) \| \pSrv x(z) ; Q_j \big) \\
                                    \typInf \Gamma, {?}\Delta, {?}\Delta'
                                \end{array}
                            }
                            \doubleLine
                            \bussUn[$\ruleLabel{typ-nd}^\ast$]{
                                \begin{array}{@{}l@{}}
                                    \vdash \bignd_{j \in J} \pRes{x} \big( \begin{array}[t]{@{}l@{}}
                                        \pRes{w} ( \bignd_{i \in I} P_i \{ w/y_i \} \| Q_j \{ w/z \} \{ v'/v \}_{v \in \dom({?}\Delta)} )
                                        \\
                                        {} \| \pSrv x(z) ; Q_j \big)
                                    \end{array} \\
                                    \typInf \Gamma, {?}\Delta, {?}\Delta'
                                \end{array}
                            }
                            \doubleLine
                            \bussUn[$\ruleLabel{typ-contract}^\ast$]{
                                \vdash \bignd_{j \in J} \pRes{x} \big( \pRes{w} ( \bignd_{i \in I} P_i \{ w/y_i \} \| Q_j \{ w/z \} ) \| \pSrv x(z) ; Q_j \big) \typInf \Gamma, {?}\Delta
                            }
                        \end{bussproof}
                    \end{mathpar}
                    \qedhere

            \end{itemize}

    \end{enumerate}
\end{proof}

\begin{theorem}[SR for the Lazy Semantics]
    \label{t:clpi:srLazy}
    If $\vdash P \typInf \Gamma$ and $P \reddLazy_S Q$, then $\vdash Q \typInf \Gamma$.
\end{theorem}

\begin{proof}
    By induction on the derivation of the reduction.
    \begin{itemize}

        \item
            Rule~\ruleLabel{red-lazy-fwd}:
            $\pRes{x} ( \bignd_{i \in I} \evalCtx[\big]{C_i}[\pFwd [x<>y]] \| Q ) \reddLazy_{x,y} \bignd_{i \in I} \evalCtx{C_i}[Q \{ y/x \}]$.
            \begin{mathpar}
                \begin{bussproof}
                    \bussAssume{
                        \forall i \in I.~
                        \vdash \evalCtx[\big]{C_i}[\pFwd [x<>y]] \typInf \Gamma, x:A
                    }
                    \doubleLine
                    \bussUn[$\ruleLabel{typ-nd}^\ast$]{
                        \vdash \bignd_{i \in I} \evalCtx[\big]{C_i}[\pFwd [x<>y]] \typInf \Gamma, x:A
                    }
                    \bussAssume{
                        \vdash Q \typInf \Delta , x:\ol{A}
                    }
                    \bussBin[\ruleLabel{typ-cut}]{
                        \vdash \pRes{x} ( \bignd_{i \in I} \evalCtx[\big]{C_i}[\pFwd [x<>y]] \| Q ) \typInf \Gamma, \Delta
                    }
                \end{bussproof}
                \and
                \implies
                \and
                \begin{bussproof}
                    \bussAssume{
                        \forall i \in I.~
                        \vdash \evalCtx{C_i}[Q \{ y/x \}] \typInf \Gamma, \Delta
                    }
                    \doubleLine
                    \bussUn[$\ruleLabel{typ-nd}^\ast$]{
                        \vdash \bignd_{i \in I} \evalCtx{C_i}[Q \{ y/x \}] \typInf \Gamma, \Delta
                    }
                \end{bussproof}
            \end{mathpar}

        \item
            Rule~\ruleLabel{red-lazy-send-recv}:
            \begin{align*}
                & \pRes{x} ( \bignd_{i \in I} \evalCtx{C_i}[\pOut* x[y_i] ; ( P_i \| Q_i )] \| \bignd_{j \in J} \evalCtx{D_j}[\pIn x(z) ; R_j] ) \\
                & {} \reddLazy_x \bignd_{i \in I} \evalCtx*{C_i}[\pRes{x} \big( Q_i \| \pRes{w} ( P_i \{ w/y_i \} \| \bignd_{j \in J} \evalCtx{D_j}[R_j \{ w/z \}] ) \big)].
            \end{align*}
            \begin{mathpar}
                \begin{bussproof}
                    \bussAssume{
                        \text{(\refitem{l}{ctxType}{send})}
                    }
                    \noLine
                    \bussUn{
                        \begin{array}{@{}l@{}}
                            \forall i \in I. \\
                            \vdash \evalCtx{C_i}[\pOut* x[y_i] ; ( P_i \| Q_i )] \typInf \Gamma, x:A \tensor B
                        \end{array}
                    }
                    \doubleLine
                    \bussUn[$\ruleLabel{typ-nd}^\ast$]{
                        \begin{array}{@{}l@{}}
                            \vdash \bignd_{i \in I} \evalCtx{C_i}[\pOut* x[y_i] ; ( P_i \| Q_i )] \\ 
                            \typInf \Gamma, x:A \tensor B
                        \end{array}
                    }
                    \bussAssume{
                        \text{(\refitem{l}{ctxType}{recv})}
                    }
                    \noLine
                    \bussUn{
                        \begin{array}{@{}l@{}}
                            \forall j \in J. \\
                            \vdash \evalCtx{D_j}[\pIn x(z) ; R_j] \vdash \Delta, x:\ol{A} \parr \ol{B}
                        \end{array}
                    }
                    \doubleLine
                    \bussUn[$\ruleLabel{typ-nd}^\ast$]{
                        \begin{array}{@{}l@{}}
                            \vdash \bignd_{j \in J} \evalCtx{D_j}[\pIn x(z) ; R_j] \\
                            \typInf \Delta, x:\ol{A} \parr \ol{B}
                        \end{array}
                    }
                    \bussBin[\ruleLabel{typ-cut}]{
                        \vdash \pRes{x} ( \bignd_{i \in I} \evalCtx{C_i}[\pOut* x[y_i] ; ( P_i \| Q_i )] \| \bignd_{j \in J} \evalCtx{D_j}[\pIn x(z) ; R_j] ) \typInf \Gamma, \Delta
                    }
                \end{bussproof}
                \and\implies\and
                \begin{bussproof}
                    \bussAssume{
                        \text{(\refitem{l}{reddLazy}{sendRecv})}
                    }
                    \noLine
                    \bussUn{
                        \vdash \bignd_{i \in I} \evalCtx[\big]{C_i}[\pRes{x} \big( Q_i \| \pRes{w} ( P_i \{ w/y_i \} \| \bignd_{j \in J} \evalCtx{D_j}[R_j \{ w/z \}] ) \big)] \typInf \Gamma, \Delta
                    }
                \end{bussproof}
            \end{mathpar}

        \item
            Rule~\ruleLabel{red-lazy-sel-bra}:
            $k' \in K$ implies 
            \begin{align*}
                &\pRes{x} ( \bignd_{i \in I} \evalCtx{C_i}[\pSel* x < k' ; P_i] \| \bignd_{j \in J} \evalCtx{D_j}[\pBra* x > \{ k : Q_j^k \}_{k \in K}] ) \\
                &{} \reddLazy_x \pRes{x} ( \bignd_{i \in I} \evalCtx{C_i}[P_i] \| \bignd_{j \in J} \evalCtx{D_j}[Q_j^{k'}] ).
            \end{align*}
            Take any $k' \in K$.
            \begin{mathpar}
                \begin{bussproof}
                    \bussAssume{
                        \text{(\refitem{l}{ctxType}{sel})}
                    }
                    \noLine
                    \bussUn{
                        \forall i \in I.~
                        \begin{array}{@{}l@{}}
                            \vdash \evalCtx{C_i}[\pSel* x < k' ; P_i]
                            \\
                            \typInf \Gamma, x:\oplus \{ k : A_k \}_{k \in K}
                        \end{array}
                    }
                    \doubleLine
                    \bussUn[$\ruleLabel{typ-nd}^\ast$]{
                        \begin{array}{@{}l@{}}
                            \vdash \bignd_{i \in I} \evalCtx{C_i}[\pSel* x < k' ; P_i]
                            \\
                            \typInf \Gamma, x:\oplus \{ k : A_k \}_{k \in K}
                        \end{array}
                    }
                    \bussAssume{
                        \text{(\refitem{l}{ctxType}{bra})}
                    }
                    \noLine
                    \bussUn{
                        \forall j \in J.~
                        \begin{array}{@{}l@{}}
                            \vdash \evalCtx{D_j}[\pBra* x > \{ k : Q_j^k \}_{k \in K}]
                            \\
                            \typInf \Delta, x:\& \{ k : \ol{A_k} \}_{k \in K}
                        \end{array}
                    }
                    \doubleLine
                    \bussUn[$\ruleLabel{typ-nd}^\ast$]{
                        \begin{array}{@{}l@{}}
                            \vdash \bignd_{j \in J} \evalCtx{D_j}[\pBra* x > \{ k : Q_j^k \}_{k \in K}]
                            \\
                            \typInf \Delta, x:\& \{ k : \ol{A_k} \}_{k \in K}
                        \end{array}
                    }
                    \bussBin[\ruleLabel{typ-cut}]{
                        \vdash \pRes{x} ( \bignd_{i \in I} \evalCtx{C_i}[\pSel* x < k' ; P_i] \| \bignd_{j \in J} \evalCtx{D_j}[\pBra* x > \{ k : Q_j^k \}_{k \in K}] ) \typInf \Gamma, \Delta
                    }
                \end{bussproof}
                \and
                \implies
                \and
                \begin{bussproof}
                    \bussAssume{
                        \forall i \in I.~
                        \vdash \evalCtx{C_i}[P_i] \typInf \Gamma, x:A
                    }
                    \doubleLine
                    \bussUn[$\ruleLabel{typ-nd}^\ast$]{
                        \vdash \bignd_{i \in I} \evalCtx{C_i}[P_i] \typInf \Gamma, x:A
                    }
                    \bussAssume{
                        \forall j \in J.~
                        \vdash \evalCtx{D_j}[Q_j^k] \typInf \Delta, x:\ol{A}
                    }
                    \doubleLine
                    \bussUn[$\ruleLabel{typ-nd}^\ast$]{
                        \vdash \bignd_{j \in J} \evalCtx{D_j}[Q_j^k] \typInf \Delta, x:\ol{A}
                    }
                    \bussBin[\ruleLabel{typ-cut}]{
                        \vdash \pRes{x} ( \bignd_{i \in I} \evalCtx{C_i}[P_i] \| \bignd_{j \in J} \evalCtx{D_j}[Q_j^k] ) \typInf \Gamma, \Delta
                    }
                \end{bussproof}
            \end{mathpar}

        \item
            Rule~\ruleLabel{red-lazy-cli-srv}:
            \begin{align*}
                &\pRes{x} ( \bignd_{i \in I} \evalCtx{C_i}[\pCli* x[y_i] ; P_i] \| \bignd_{j \in J} \evalCtx{D_j}[\pSrv x(z) ; Q_j] ) \\
                &{} \reddLazy_x \bignd_{j \in J} \evalCtx*{D_j}[\pRes{x} ( \bignd_{i \in I} \evalCtx{C_i}[P_i \{ w/z \}] \| Q_j \{ w/z \} ) \| \pSrv x(z) ; Q_j].
            \end{align*}
            \begin{mathpar}
                \begin{bussproof}
                    \bussAssume{
                        \text{(\refitem{l}{ctxType}{cli})}
                    }
                    \noLine
                    \bussUn{
                        \forall i \in I.~
                        \vdash \evalCtx{C_i}[\pCli* x[y_i] ; P_i] \typInf \Gamma, x:{?}A
                    }
                    \doubleLine
                    \bussUn[$\ruleLabel{typ-nd}^\ast$]{
                        \vdash \bignd_{i \in I} \evalCtx{C_i}[\pCli* x[y_i] ; P_i] \typInf \Gamma, x:{?}A
                    }
                    \bussAssume{
                        \text{(\refitem{l}{ctxType}{srv})}
                    }
                    \noLine
                    \bussUn{
                        \forall j \in J.~
                        \vdash \evalCtx{D_j}[\pSrv x(z) ; Q_j] \typInf \Delta, x:{!}\ol{A}
                    }
                    \doubleLine
                    \bussUn[$\ruleLabel{typ-nd}^\ast$]{
                        \vdash \bignd_{j \in J} \evalCtx{D_j}[\pSrv x(z) ; Q_j] \typInf \Delta, x:{!}\ol{A}
                    }
                    \bussBin[\ruleLabel{typ-cut}]{
                        \vdash \pRes{x} ( \bignd_{i \in I} \evalCtx{C_i}[\pCli* x[y_i] ; P_i] \| \bignd_{j \in J} \evalCtx{D_j}[\pSrv x(z) ; Q_j] ) \typInf \Gamma, \Delta
                    }
                \end{bussproof}
                \and
                \implies
                \and
                \begin{bussproof}
                    \bussAssume{
                        \text{(\refitem{l}{reddLazy}{cliSrv})}
                    }
                    \noLine
                    \bussUn{
                        \vdash \bignd_{j \in J} \evalCtx[\big]{D_j}[\pRes{x} \big( \pRes{w} ( \bignd_{i \in I} \evalCtx{C_i}[P_i \{ w/z \}] \| Q_j \{ w/z \} ) \| \pSrv x(z) ; Q_j \big)] \typInf \Gamma, \Delta
                    }
                \end{bussproof}
            \end{mathpar}

        \item
            Rule~\ruleLabel{red-lazy-close-wait}:
            \[
                \pRes{x} ( \bignd_{i \in I} \evalCtx{C_i}[\pClose x[]] \| \bignd_{j \in J} \evalCtx{D_j}[\pWait x() ; Q_j] ) \reddLazy_x \bignd_{i \in I} \evalCtx{C_i}[\0] \| \bignd_{j \in J} \evalCtx{D_j}[Q_j].
            \]
            \begin{mathpar}
                \begin{bussproof}
                    \bussAssume{
                        \text{(\refitem{l}{ctxType}{close})}
                    }
                    \noLine
                    \bussUn{
                        \forall i \in I.~
                        \vdash \evalCtx{C_i}[\pClose x[]] \typInf \Gamma, x:\1
                    }
                    \doubleLine
                    \bussUn[$\ruleLabel{typ-nd}^\ast$]{
                        \vdash \bignd_{i \in I} \evalCtx{C_i}[\pClose x[]] \typInf \Gamma, x:\1
                    }
                    \bussAssume{
                        \text{(\refitem{l}{ctxType}{wait})}
                    }
                    \noLine
                    \bussUn{
                        \forall j \in J.~
                        \vdash \evalCtx{D_j}[\pWait x() ; Q_j] \typInf \Delta, x:\bot
                    }
                    \doubleLine
                    \bussUn[$\ruleLabel{typ-nd}^\ast$]{
                        \vdash \bignd_{j \in J} \evalCtx{D_j}[\pWait x() ; Q_j] \typInf \Delta, x:\bot
                    }
                    \bussBin[\ruleLabel{typ-cut}]{
                        \vdash \pRes{x} ( \bignd_{i \in I} \evalCtx{C_i}[\pClose x[]] \| \bignd_{j \in J} \evalCtx{D_j}[\pWait x() ; Q_j] ) \typInf \Gamma, \Delta
                    }
                \end{bussproof}
                \and
                \implies
                \and
                \begin{bussproof}
                    \bussAssume{
                        \forall i \in I.~
                        \vdash \evalCtx{C_i}[\0] \typInf \Gamma
                    }
                    \doubleLine
                    \bussUn[$\ruleLabel{typ-nd}^\ast$]{
                        \vdash \bignd_{i \in I} \evalCtx{C_i}[\0] \typInf \Gamma
                    }
                    \bussAssume{
                        \forall j \in J.~
                        \vdash \evalCtx{D_j}[Q_j] \typInf \Delta
                    }
                    \doubleLine
                    \bussUn[$\ruleLabel{typ-nd}^\ast$]{
                        \vdash \bignd_{j \in J} \evalCtx{D_j}[Q_j] \typInf \Delta
                    }
                    \bussBin[\ruleLabel{typ-par}]{
                        \vdash \bignd_{i \in I} \evalCtx{C_i}[\0] \| \bignd_{j \in J} \evalCtx{D_j}[Q_j] \typInf \Gamma, \Delta
                    }
                \end{bussproof}
            \end{mathpar}

        \item
            Rule~\ruleLabel{red-lazy-some}:
            \begin{align*}
                &\pRes{x} ( \bignd_{i \in I} \evalCtx{C_i}[\pSome x ; P_i] \| \bignd_{j \in J} \evalCtx{D_j}[\pSomeIn x{w_1,\ldots,w_n} ; Q_j] ) \\
                &{} \reddLazy_x \pRes{x} ( \bignd_{i \in I} \evalCtx{C_i}[P_i] \| \bignd_{j \in J} \evalCtx{D_j}[Q_j] ).
            \end{align*}
            \begin{mathpar}
                \begin{bussproof}
                    \bussAssume{
                        \text{(\refitem{l}{ctxType}{some})}
                    }
                    \noLine
                    \bussUn{
                        \begin{array}{@{}l@{}}
                            \forall i \in I. \\
                            \vdash \evalCtx{C_i}[\pSome x ; P_i] \\
                            \typInf \Gamma, x:\& A
                        \end{array}
                    }
                    \doubleLine
                    \bussUn[$\ruleLabel{typ-nd}^\ast$]{
                        \begin{array}{@{}l@{}}
                            \vdash \bignd_{i \in I} \evalCtx{C_i}[\pSome x ; P_i] \\
                            \typInf \Gamma, x:\& A
                        \end{array}
                    }
                    \bussAssume{
                        \text{(\refitem{l}{ctxType}{someIn})}
                    }
                    \noLine
                    \bussUn{
                        \begin{array}{@{}l@{}}
                            \forall j \in J. \\
                            \vdash \evalCtx{D_j}[\pSomeIn x{w_1,\ldots,w_n} ; Q_j] \\
                            \typInf \Delta, x:\oplus \ol{A}
                        \end{array}
                    }
                    \doubleLine
                    \bussUn[$\ruleLabel{typ-nd}^\ast$]{
                        \begin{array}{@{}l@{}}
                            \vdash \bignd_{j \in J} \evalCtx{D_j}[\pSomeIn x{w_1,\ldots,w_n} ; Q_j] 
                            \\
                            \typInf \Delta, x:\oplus \ol{A}
                        \end{array}
                    }
                    \bussBin[\ruleLabel{typ-cut}]{
                        \vdash \pRes{x} ( \bignd_{i \in I} \evalCtx{C_i}[\pSome x ; P_i] \| \bignd_{j \in J} \evalCtx{D_j}[\pSomeIn x{w_1,\ldots,w_n} ; Q_j] ) \typInf \Gamma, \Delta
                    }
                \end{bussproof}
                \and
                \implies
                \and
                \begin{bussproof}
                    \bussAssume{
                        \forall i \in I.~
                        \vdash \evalCtx{C_i}[P_i] \vdash \Gamma, x:A
                    }
                    \doubleLine
                    \bussUn[$\ruleLabel{typ-nd}^\ast$]{
                        \vdash \bignd_{i \in I} \evalCtx{C_i}[P_i] \typInf \Gamma, x:A
                    }
                    \bussAssume{
                        \forall j \in J.~
                        \vdash \evalCtx{D_j}[Q_j] \typInf \Delta, x:\ol{A}
                    }
                    \doubleLine
                    \bussUn[$\ruleLabel{typ-nd}^\ast$]{
                        \vdash \bignd_{j \in J} \evalCtx{D_j}[Q_j] \typInf \Delta, x:\ol{A}
                    }
                    \bussBin[\ruleLabel{typ-cut}]{
                        \vdash \pRes{x} ( \bignd_{i \in I} \evalCtx{C_i}[P_i] \| \bignd_{j \in J} \evalCtx{D_j}[Q_j] ) \typInf \Gamma, \Delta
                    }
                \end{bussproof}
            \end{mathpar}

        \item
            Rule~\ruleLabel{red-lazy-none}:
            \begin{align*}
                &\pRes{x} ( \bignd_{i \in I} \evalCtx{C_i}[\pNone x] \| \bignd_{j \in J} \evalCtx{D_j}[\pSomeIn x{w_1,\ldots,w_n} ; Q_j] ) \\
                &{} \reddLazy_x \pRes{x} ( \bignd_{i \in I} \evalCtx{C_i}[\0] \| \bignd_{j \in J} \evalCtx{D_j}[\pNone w_1 \| \ldots \| \pNone w_n] ).
            \end{align*}
            \begin{mathpar}
                \begin{bussproof}
                    \bussAssume{
                        \text{(\refitem{l}{ctxType}{none})}
                    }
                    \noLine
                    \bussUn{
                        \begin{array}{@{}l@{}}
                            \forall i \in I. \\
                            \vdash \evalCtx{C_i}[\pNone x] \typInf \Gamma, x:\& A
                        \end{array}
                    }
                    \doubleLine
                    \bussUn[$\ruleLabel{typ-nd}^\ast$]{
                        \begin{array}{@{}l@{}}
                            \vdash \bignd_{i \in I} \evalCtx{C_i}[\pNone x] \\
                            \typInf \Gamma, x:\& A
                        \end{array}
                    }
                    \bussAssume{
                        \text{(\refitem{l}{ctxType}{someIn})}
                    }
                    \noLine
                    \bussUn{
                        \begin{array}{@{}l@{}}
                            \forall j \in J. \\
                            \\
                            \vdash \evalCtx{D_j}[\pSomeIn x{w_1,\ldots,w_n} ; Q_j] \typInf \Delta, x:\oplus \ol{A}
                        \end{array}
                    }
                    \doubleLine
                    \bussUn[$\ruleLabel{typ-nd}^\ast$]{
                        \begin{array}{@{}l@{}}
                            \vdash \bignd_{j \in J} \evalCtx{D_j}[\pSomeIn x{w_1,\ldots,w_n} ; Q_j] 
                            \\
                            \typInf \Delta, x:\oplus \ol{A}
                        \end{array}
                    }
                    \bussBin[\ruleLabel{typ-cut}]{
                        \vdash \pRes{x} ( \bignd_{i \in I} \evalCtx{C_i}[\pNone x] \| \bignd_{j \in J} \evalCtx{D_j}[\pSomeIn x{w_1,\ldots,w_n} ; Q_j] ) \typInf \Gamma, \Delta
                    }
                \end{bussproof}
                \and
                \implies
                \and
                \begin{bussproof}
                    \bussAssume{
                        \forall i \in I.~
                        \vdash \evalCtx{C_i}[\0] \typInf \Gamma
                    }
                    \doubleLine
                    \bussUn[$\ruleLabel{typ-nd}^\ast$]{
                        \vdash \bignd_{i \in I} \evalCtx{C_i}[P_i] \typInf \Gamma
                    }
                    \bussAssume{
                        \forall j \in J.~
                        \vdash \evalCtx{D_j}[\pNone w_1 \| \ldots \| \pNone w_n] \typInf \Delta
                    }
                    \doubleLine
                    \bussUn[$\ruleLabel{typ-nd}^\ast$]{
                        \vdash \bignd_{j \in J} \evalCtx{D_j}[\pNone w_1 \| \ldots \| \pNone w_n] \typInf \Delta
                    }
                    \bussBin[\ruleLabel{typ-par}]{
                        \vdash \bignd_{i \in I} \evalCtx{C_i}[\0] \| \bignd_{j \in J} \evalCtx{D_j}[\pNone w_1 \| \ldots \| \pNone w_n] \typInf \Gamma, \Delta
                    }
                \end{bussproof}
            \end{mathpar}
            \qedhere

    \end{itemize}
\end{proof}
%</clpi:tp:srLazy>

\subsubsection{Deadlock Freedom}
\label{ss:DFLazy}

%<*clpi:dfLazy>
We require the following definitions and intermediate results:
\begin{itemize}

    \item
        \Cref{d:clpi:mCtx} defines non-deterministic reduction contexts with multiple holes.

    \item
        \Cref{l:clpi:ndCtxMultihole} states that processes in ND-context form with at least one prefix on a free name can be written as multi-hole ND-contexts.

    \item
        \Cref{l:clpi:multiNdDet} states that multi-hole ND-contexts can be split into deterministic and non-deterministic parts.

    \item
        \Cref{d:clpi:ndFlat} defines the \emph{flattening} of multi-hole ND-contexts, propagating choices to the top-level.

    \item
        \Cref{l:clpi:multiShape} states that well-typed processes in multi-hole ND-context form can be flattened to the non-deterministic composition of D-contexts.

    \item
        \Cref{l:clpi:flatRed} states that when a process reduces by synchronization between flattened multi-hole ND-contexts, then the same process with unflattened mutli-hole ND-contexts reduces to the same process.

    \item
        \Cref{t:clpi:eagerImpliesLazy} states that an eager reduction implies a lazy reduction to the same process.

    \item
        \Cref{t:clpi:dfLazy} proved deadlock-freedom for the lazy semantics.

\end{itemize}

\begin{definition}[Multi-hole Non-deterministic Reduction Contexts]
    \label{d:clpi:mCtx}
    \[
        \evalCtx{M} ::= \evalHole \sepr \pRes{x} ( P \| \evalCtx{M} ) \sepr P \| \evalCtx{M} \sepr \evalCtx{M} \nd \evalCtx{M}
    \]
\end{definition}

\begin{lemma}
    \label{l:clpi:ndCtxMultihole}
    If $\vdash \evalCtx{N}[\alpha ; P] \typInf \Gamma, x:A$ and $x \in \subjs(\alpha)$, then there are $\evalCtx{M}$ and ${(\alpha_i ; P_i)}_{i \in I}$ such that $\evalCtx{N}[\alpha ; P] = \evalCtx{M}[\alpha_i ; P_i]_{i \in I}$ where $x \notin \fn(\evalCtx{M)}$ and $x \in \bigcap_{i \in I} \fn(\alpha_i ; P_i)$ and there is $i' \in I$ such that $\alpha_{i'} ; P_{i'} = \alpha ; P$.
\end{lemma}

\begin{lemma}
    \label{l:clpi:multiNdDet}
    For every multi-hole ND-context $\evalCtx{M}$ with indices $I$:
    \begin{itemize}

        \item
            If $\evalCtx{M}$ has two or more holes, there are $\evalCtx{C}$, $\evalCtx{M_1}$ with indices $I_1$, $\evalCtx{M_2}$ with indices $I_2$ such that $\evalCtx{M} = \evalCtx{C}[\evalCtx{M_1} \nd \evalCtx{M_2}]$ where $I_1 \cap I_2 = \emptyset$ and $I = I_1 \cup I_2$.

        \item
            If $\evalCtx{M}$ has only one hole, there is $\evalCtx{C}$ such that $\evalCtx{M} = \evalCtx{C}$.

    \end{itemize}
\end{lemma}

\begin{definition}
    \label{d:clpi:ndFlat}
    \begin{align*}
        \flat(\evalCtx{C}[\evalCtx{M} \nd \evalCtx{M'}])
        &\deq \flat(\evalCtx{C}[\evalCtx{M}]) \nd \flat(\evalCtx{C}[\evalCtx{M'}])
        &
        \flat(\evalCtx{C})
        &\deq \evalCtx{C}
    \end{align*}
\end{definition}

\begin{lemma}
    \label{l:clpi:multiShape}
    If $\vdash \evalCtx{M}[P_i]_{i \in I} \typInf \Gamma$ where $x \notin \fn(\evalCtx{M})$ and $\forall i \in I.~ x \in \fn(P_i)$, then there are ${(\evalCtx{C_i})}_{i \in I}$ such that $\flat(\evalCtx{M}[P_i]_{i \in I}) = \bignd_{i \in I} \evalCtx{C_i}[P_i]$ where $\forall i \in I.~ x \notin \fn(\evalCtx{C_i})$.
\end{lemma}

\begin{lemma}
    \label{l:clpi:flatRed}
    If
    \[
        \pRes{x} ( \evalCtx[\big]{N}[\flat(\evalCtx{M}[\alpha_i;P_i]_{i \in I})] \| \evalCtx[\big]{N'}[\flat(\evalCtx{M'}[\beta_j ; Q_j]_{j \in J})] ) \reddLazy_S R,
    \]
    then
    \[
        \pRes{x} ( \evalCtx[\big]{N}[\evalCtx{M}[\alpha_i ; P_i]_{i \in I}] \| \evalCtx[\big]{N'}[\evalCtx{M'}[\beta_j ; Q_j]_{j \in J}]) \reddLazy_S R.
    \]
\end{lemma}

\begin{proof}
    By induction on the structures of $\evalCtx{M}$ and $\evalCtx{M'}$.
    By \Cref{l:clpi:multiNdDet}, we only have to consider two cases for $\evalCtx{M}$ ($\evalCtx{M} = \evalCtx{C}[\evalCtx{M_1} \nd \evalCtx{M_2}]$ and $\evalCtx{M} = \evalCtx{C}$), and similarly for $\evalCtx{M'}$.
    We only detail the base case ($\evalCtx{M} = \evalCtx{C}$ and $\evalCtx{M'} = \evalCtx{C'}$) and a representative inductive case ($\evalCtx{M} = \evalCtx{C}[\evalCtx{M_1} \nd \evalCtx{M_2}]$ and $\evalCtx{M'} = \evalCtx{C'}$).
    \begin{itemize}

        \item
            $\evalCtx{M} = \evalCtx{C}$ and $\evalCtx{M'} = \evalCtx{C'}$.
            Note that $\evalCtx{M}$ and $\evalCtx{M'}$ have only one hole; w.l.o.g., assume \mbox{$I = J = \{1\}$}.
            \begin{align*}
                \flat(\evalCtx{M}[\alpha_1 ; P_1]) &= \flat(\evalCtx{C}[\alpha_1 ; P_1]) = \evalCtx{C}[\alpha_1 ; P_1] = \evalCtx{M}[\alpha_1 ; P_1]
                \\
                \flat(\evalCtx{M'}[\beta_1 ; Q_1]) &= \flat(\evalCtx{C'}[\beta_1 ; Q_1]) = \evalCtx{C'}[\beta_1 ; Q_1] = \evalCtx{M'}[\beta_1 ; Q_1]
            \end{align*}
            The thesis follows by assumption and equality.

        \item
            $\evalCtx{M} = \evalCtx{C}[\evalCtx{M_1} \nd \evalCtx{M_2}]$ and $\evalCtx{M'} = \evalCtx{C'}$.
            Note that $\evalCtx{M'}$ has only one hole; w.l.o.g., assume $J = \{1\}$.
            \begin{align}
                & \pRes{x} ( \evalCtx[\big]{N}[\flat(\evalCtx{M}[\alpha_i ; P_i]_{i \in I})] \| \evalCtx[\big]{N'}[\flat(\evalCtx{M'}[\beta_1 ; Q_1])] )
                \nonumber
                \\
                &= \pRes{x} ( \evalCtx[\big]{N}[\flat(\evalCtx{C}[\evalCtx{M_1} \nd \evalCtx{M_2}])[\alpha_i ; P_i]_{i \in I}] \| \evalCtx[\big]{N'}[\flat(\evalCtx{C'}[\beta_1 ; Q_1])] )
                \nonumber
                \\
                &= \pRes{x} ( \evalCtx[\big]{N}[(\flat(\evalCtx{C}[\evalCtx{M_1}]) \nd \flat(\evalCtx{C}[\evalCtx{M_2}]))[\alpha_i ; P_i]_{i \in I}] \| \evalCtx[\big]{N'}[\evalCtx{C'}[\beta_1 ; Q_1]] )
                \label{eq:clpi:oneImplTwoBeforeSplit}
            \end{align}
            There are $I_1$ and $I_2$ such that $I_1 \cap I_2 = \emptyset$ and $I = I_1 \cup I_2$ and
            \begin{align}
                & \pRes{x} ( \evalCtx[\big]{N}[\flat(\evalCtx{M}[\alpha_i ; P_i]_{i \in I})] \| \evalCtx[\big]{N'}[\flat(\evalCtx{M'}[\beta_1 ; Q_1])] )
                \nonumber
                \\
                &= \pRes{x} ( \evalCtx[\big]{N}[\flat(\evalCtx{C}[\evalCtx{M_1}])[\alpha_i ; P_i]_{i \in I_1} \nd \flat(\evalCtx{C}[\evalCtx{M_2}])[\alpha_i ; P_i]_{i \in I_2}] \| \evalCtx[\big]{N'}[\evalCtx{C'}[\beta_1 ; Q_1]] ).
                \tag{by~\eqref{eq:clpi:oneImplTwoBeforeSplit}}
                \\
                \label{eq:clpi:oneImplTwoAfterSplit}
            \end{align}
            Let $\evalCtx{N_1} = \evalCtx[\big]{N}[\evalHole \nd \flat(\evalCtx{C}[\evalCtx{M_2}])[\alpha_i ; P_i]_{i \in I_2}]$.
            \begin{align}
                & \pRes{x} ( \evalCtx[\big]{N}[\flat(\evalCtx{M}[\alpha_i ; P_i]_{i \in I})] \| \evalCtx[\big]{N'}[\flat(\evalCtx{M'}[\beta_1 ; Q_1])] )
                \nonumber
                \\
                &= \pRes{x} ( \evalCtx[\big]{N_1}[\flat(\evalCtx{C}[\evalCtx{M_1}])[\alpha_i ; P_i]_{i \in I_1}] \| \evalCtx[\big]{N'}[\evalCtx{C'}[\beta_1 ; Q_1]] )
                \tag{by~\eqref{eq:clpi:oneImplTwoAfterSplit}}
                \\
                &\reddLazy_S R
                \tag{by assumption}
                \\
                \label{eq:clpi:oneImplTwoLeftRed}
                \\
                & \pRes{x} ( \evalCtx[\big]{N_1}[\evalCtx{C}[\evalCtx{M_1}][\alpha_i ; P_i]_{i \in I_1}] \| \evalCtx[\big]{N'}[\evalCtx{C'}[\beta_1 ; Q_1]] )
                \nonumber
                \\
                &= \pRes{x} ( \evalCtx[\big]{N}[\evalCtx{C}[\evalCtx{M_1}][\alpha_i ; P_i]_{i \in I_1} \nd \flat(\evalCtx{C}[\evalCtx{M_2}])[\alpha_i ; P_i]_{i \in I_2}] \| \evalCtx[\big]{N'}[\evalCtx{C'}[\beta_1 ; Q_1]] )
                \nonumber
                \\
                &\reddLazy_S R
                \tag{by IH on~\eqref{eq:clpi:oneImplTwoLeftRed}}
                \\
                \label{eq:clpi:oneImplTwoBeforeRightRed}
            \end{align}
            Let $\evalCtx{N_2} = \evalCtx[\big]{N}[\evalCtx{C}[\evalCtx{M_1}][\alpha_i ; P_i]_{i \in I_1} \nd \evalHole]$.
            \begin{align}
                & \pRes{x} ( \evalCtx[\big]{N}[\evalCtx{C}[\evalCtx{M_1}][\alpha_i ; P_i]_{i \in I_1} \nd \flat(\evalCtx{C}[\evalCtx{M_2}])[\alpha_i ; P_i]_{i \in I_2}] \| \evalCtx[\big]{N'}[\evalCtx{C'}[\beta_1 ; Q_1]] )
                \nonumber
                \\
                &= \pRes{x} ( \evalCtx[\big]{N_2}[\flat(\evalCtx{C}[\evalCtx{M_2}])[\alpha_i ; P_i]_{i \in I_2}] \| \evalCtx[\big]{N'}[\evalCtx{C'}[\beta_1 ; Q_1]] )
                \nonumber
                \\
                &\reddLazy_S R
                \tag{by~\eqref{eq:clpi:oneImplTwoBeforeRightRed}}
                \\
                \label{eq:clpi:oneImplTwoRightRed}
                \\
                & \pRes{x} ( \evalCtx[\big]{N_2}[\evalCtx{C}[\evalCtx{M_2}][\alpha_i ; P_i]_{i \in I_2}] \| \evalCtx[\big]{N'}[\evalCtx{C'}[\beta_1 ; Q_1]] )
                \nonumber
                \\
                &= \pRes{x} ( \evalCtx[\big]{N}[\evalCtx{C}[\evalCtx{M_1}][\alpha_i ; P_i]_{i \in I_1} \nd \evalCtx{C}[\evalCtx{M_2}][\alpha_i ; P_i]_{i \in I_2}] \| \evalCtx[\big]{N'}[\evalCtx{C'}[\beta_1 ; Q_1]] )
                \nonumber
                \\
                &= \pRes{x} ( \evalCtx[\Big]{N}[\evalCtx[\big]{C}[\evalCtx{M_1}[\alpha_i ; P_i]_{i \in I_1}] \nd \evalCtx[\big]{C}[\evalCtx{M_2}[\alpha_i ; P_i]_{i \in I_2}]] \| \evalCtx[\big]{N'}[\evalCtx{C'}[\beta_1 ; Q_1]] )
                \nonumber
                \\
                &\reddLazy_S R
                \tag{by IH on~\eqref{eq:clpi:oneImplTwoRightRed}}
                \\
                \label{eq:clpi:oneImplTwoIHRed}
                \\
                & \pRes{x} ( \evalCtx[\Big]{N}[\evalCtx[\big]{C}[\evalCtx{M_1}[\alpha_i ; P_i]_{i \in I_1} \nd \evalCtx{M_2}[\alpha_i ; P_i]_{i \in I_2}]] \| \evalCtx[\big]{N'}[\evalCtx{C'}[\beta_1 ; Q_1]] )
                \nonumber
                \\
                &= \pRes{x} ( \evalCtx[\Big]{N}[\evalCtx[\big]{C}[(\evalCtx{M_1} \nd \evalCtx{M_2})[\alpha_i ; P_i]_{i \in I}]] \| \evalCtx[\big]{N'}[\evalCtx{C'}[\beta_1 ; Q_1]] )
                \nonumber
                \\
                &= \pRes{x} ( \evalCtx[\big]{N}[\evalCtx{C}[\evalCtx{M_1} \nd \evalCtx{M_2}][\alpha_i ; P_i]_{i \in I}] \| \evalCtx[\big]{N'}[\evalCtx{C'}[\beta_1 ; Q_1]] )
                \nonumber
                \\
                &= \pRes{x} ( \evalCtx[\big]{N}[\evalCtx{M}[\alpha_i ; P_i]_{i \in I}] \| \evalCtx[\big]{N'}[\evalCtx{M'}[\beta_1 ; Q_1]] )
                \nonumber
                \\
                &\reddLazy_S R
                \tag{by Rule~\ruleLabel{red-lazy-scope} on~\eqref{eq:clpi:oneImplTwoIHRed}}
            \end{align}
            \qedhere

    \end{itemize}
\end{proof}

\begin{theorem}
    \label{t:clpi:eagerImpliesLazy}
    If $\vdash P \typInf \Gamma$ and $P \reddEager R$, then $P \reddLazy_S R$.
\end{theorem}

\begin{proof}
    By induction on the derivation of the reduction.
    The inductive cases of Rules~\ruleLabel{red-eager-cong}, \ruleLabel{red-eager-conn}, \ruleLabel{red-eager-par}, and~\ruleLabel{red-eager-nd} follow from the IH straightforwardly, using the corresponding closure rule for $\reddLazy$.
    As representative base case, we consider Rule~\ruleLabel{red-eager-close-wait}: $P = \pRes{x} ( \evalCtx{N}[\pClose x[]] \| \evalCtx{N'}[\pWait x() ; Q] ) \reddEager R$.

    By inversion of typing, $\vdash \evalCtx{N}[\pClose x[]] \typInf \Gamma, x:A$, so by \Cref{l:clpi:ndCtxMultihole}, there are $\evalCtx{M}$ and ${(\alpha_i ; P_i)}_{i \in I}$ such that $\evalCtx{N}[\pClose x[]] = \evalCtx{M}[\alpha_i ; P_i]_{i \in I}$ where $x \notin \fn(\evalCtx{M})$ and $x \in \bigcap_{i \in I} \fn(\alpha_i ; P_i)$ and there is $i' \in I$ such that $\alpha_{i'} ; P_{i'} = \pClose x[]$.
    Similarly, there are $\evalCtx{M'}$ and ${(\beta_j ; Q_j)}_{j \in J}$ such that $\evalCtx{N'}[\pWait x() ; Q] = \evalCtx{M'}[\beta_j ; Q_j]_{j \in J}$ where $x \notin \fn(\evalCtx{M'})$ and $x \in \bigcap_{j \in J} \fn(\beta_j ; Q_j)$ and there is $j' \in J$ such that $\beta_{j'} ; Q_{j'} = \pWait x() ; Q$.

    By \Cref{l:clpi:multiShape},
    \begin{mathpar}
        \flat(\evalCtx{M}[\alpha_i;P_i]_{i \in I}) = \bignd_{i \in I} \evalCtx{C_i}[\alpha_i ; P_i]
        \and \text{and} \and
        \flat(\evalCtx{M'}[\beta_j ; Q_j]_{j \in J}) = \bignd_{j \in J} \evalCtx{C'_j}[\beta_j ; Q_j].
    \end{mathpar}
    By typability, there is $I' \subseteq I$ such that $\forall i \in I'.~ \alpha_i \prefRel \pClose x[]$ and \mbox{$\forall i \in I \setminus I'.~ \alpha_i \nprefRel \pClose x[]$}; hence, \mbox{$i' \in I'$}.
    Similarly, there is $J' \subseteq J$ such that $\forall j \in J'.~ \beta_j \prefRel \pWait x()$ and $\forall j \in J \setminus J'.~ \beta_j \nprefRel \pWait x()$; hence, $j' \in J'$.
    Then, by \Cref{d:clpi:precongLazy}, 
    \begin{mathpar}
        \flat(\evalCtx{M}[\alpha_i ; P_i]_{i \in I}) \precongLazy{x} \bignd_{i \in I'} \evalCtx{C_i}[\pClose x[]]
        \and \text{and} \and
        \flat(\evalCtx{M'}[\beta_j ; Q_j]_{j \in J}) \precongLazy{x} \bignd_{j \in J'} \evalCtx{C_j}[\pWait x() ; Q_j].
    \end{mathpar}
    By Rule~\ruleLabel{red-lazy-close-wait},
    \[
        \pRes{x} ( \bignd_{i \in I'} \evalCtx{C_i}[\pClose x[]] \| \bignd_{j \in J'} \evalCtx{C_j}[\pWait x() ; Q_j] ) \reddLazy_x R,
    \]
    so by Rule~\ruleLabel{red-lazy-precong},
    \[
        \pRes{x} ( \flat(\evalCtx{M}[\alpha_i ; P_i]_{i \in I}) \| \flat(\evalCtx{M'}[\beta_j ; Q_j]_{j \in J}) ) \reddLazy_x R.
    \]
    Then, by \Cref{l:clpi:flatRed},
    \[
        \pRes{x} ( \evalCtx{M}[\alpha_i ; P_i]_{i \in I} \| \evalCtx{M'}[\beta_j ; Q_j]_{j \in J} ) \reddLazy_x R.
    \]

    As second base case, we consider Rule~\ruleLabel{red-eager-fwd}: \mbox{$P = \pRes{x} ( \evalCtx[\big]{N}[\pFwd [x<>y]] \| Q ) \reddEager R$}.
    By inversion of typing, $\vdash \evalCtx[\big]{N}[\pFwd [x<>y]] \typInf \Gamma, x:A, y:\ol{A}$, so by \Cref{l:clpi:ndCtxMultihole}, there are $\evalCtx{M}$ and~\mbox{${(\alpha_i ; P_i)}_{i \in I}$} such that $\evalCtx[\big]{N}[\pFwd [x<>y]] = \evalCtx{M}[\alpha_i ; P_i]_{i \in I}$ where $x \notin \fn(\evalCtx{M)}$ and $x \in \bigcap_{i \in I} \fn(\alpha_i ; P_i)$ and there is $i' \in I$ such that $\alpha_{i'} ; P_{i'} = \pFwd [x<>y]$.

    By \Cref{l:clpi:multiShape}, $\flat(\evalCtx{M}[\alpha_i ; P_i]_{i \in I}) = \bignd_{i \in I} \evalCtx{C_i}[\alpha_i ; P_i]$.
    By typability, there is $I' \subseteq I$ such that $\forall i \in I'.~ \alpha_i = \pFwd [x<>y]$ and $\forall i \in I \setminus I'.~ \alpha_i \neq \pFwd [x<>y]$; hence, $i' \in I'$.

    Then, by \Cref{d:clpi:precongLazy}, $\flat(\evalCtx{M}[\alpha_i ; P_i]_{i \in I}) \precongLazy{x,y} \bignd_{i \in I'} \evalCtx{C_i}[\pFwd [x<>y]]$.
    By Rule~\ruleLabel{red-lazy-fwd},
    \[
        \pRes{x} ( \bignd_{i \in I}\evalCtx[\big]{C_i}[\pFwd [x<>y]] \| Q ) \reddLazy_{x,y} R,
    \]
    so by Rule~\ruleLabel{red-lazy-precong},
    \[
        \pRes{x} ( \flat(\evalCtx{M}[\alpha_i ; P_i]_{i \in I}) \| Q ) \reddLazy_{x,y} R.
    \]
    Then, by \Cref{l:clpi:flatRed},
    \[
        \pRes{x} ( \evalCtx{M}[\alpha_i ; P_i]_{i \in I} \| Q ) \reddLazy_{x,y} R.
        \tag*{\qedhere}
    \]
\end{proof}

\begin{theorem}[Deadlock-freedom: Lazy Semantics]
    \label{t:clpi:dfLazy}
    If $\vdash P \typInf \emptyset$ and $P \not\equiv \0$, then $P \reddLazy_S R$ for some $S$ and $R$.
\end{theorem}

\begin{proof}
    As a corollary of \Cref{t:clpi:dfEager,t:clpi:eagerImpliesLazy}.
\end{proof}
%</clpi:dfLazy>
