# Supplementary material for: Correctly Communicating Software: Distributed, Asynchronous, and Beyond (extended version)
Source: arXiv:2402.09595 source file (2024-03-01)
Supplement: Supplementary file 6 [file pi-proofs.tex]

% !TeX root = ../../../../main.tex
\section{Proofs of Type Preservation and Deadlock-freedom for (Full) \texorpdfstring{\clpi}{Pi}}
\label{s:piProofs}

Here we prove \Cref{t:srPi,t:dfPi} (type preservation and deadlock-freedom for the lazy semantics, respectively), as well as the analogue results for the eager semantics.
In fact, deadlock-freedom for the lazy semantics follows from deadlock-freedom for the eager semantics, so we present the proofs for the eager semantics first.

\subsection{Eager Semantics}
\label{ss:proofsEager}

\subsubsection{Subject Congruence}

\begin{theorem}\label{t:subcong}
    If $P \vdash \Gamma$ and $P \equiv Q$, then $Q \vdash \Gamma$.
\end{theorem}

\begin{proof}
    By induction on the derivation of the structural congruence.
    We first detail the base cases:
    \begin{itemize}
        \item
            $P \equiv_\alpha P' \implies P \equiv P'$.
            Since alpha-renaming only affects bound names, it does not affect the names in $\Gamma$, so clearly $P' \vdash \Gamma$.

        \item
            $\pFwd [x<>y] \equiv \pFwd [y<>x]$.
            \begin{mathpar}
                \inferrule{ }{
                    \pFwd [x<>y] \vdash x{:}A, y{:}\ol{A}
                }
                \equiv
                \inferrule{ }{
                    \pFwd [y<>x] \vdash x{:}A, y{:}\ol{A}
                }
            \end{mathpar}

        \item
            $P \| Q \equiv Q \| P$.
            \begin{mathpar}
                \inferrule{
                    P \vdash \Gamma
                    \\
                    Q \vdash \Delta
                }{
                    P \| Q \vdash \Gamma, \Delta
                }
                \equiv
                \inferrule{
                    Q \vdash \Delta
                    \\
                    P \vdash \Gamma
                }{
                    Q \| P \vdash \Gamma, \Delta
                }
            \end{mathpar}

        \item
            $(P \| Q) \| R \equiv P \| (Q \| R)$.
            \begin{mathpar}
                \inferrule{
                    \inferrule*{
                        P \vdash \Gamma
                        \\
                        Q \vdash \Delta
                    }{
                        P \| Q \vdash \Gamma, \Delta
                    }
                    \\
                    R \vdash \Lambda
                }{
                    (P \| Q) \| R \vdash \Gamma, \Delta, \Lambda
                }
                \equiv
                \inferrule{
                    P \vdash \Gamma
                    \\
                    \inferrule*{
                        Q \vdash \Delta
                        \\
                        R \vdash \Lambda
                    }{
                        Q \| R \vdash \Delta, \Lambda
                    }
                }{
                    P \| (Q \| R) \vdash \Gamma, \Delta, \Lambda
                }
            \end{mathpar}

        \item
            $P \| \0 \equiv P$
            \begin{mathpar}
                \inferrule{
                    P \vdash \Gamma
                    \\
                    \inferrule*{ }{
                        \0 \vdash \emptyset
                    }
                }{
                    P \| \0 \vdash \Gamma
                }
                \equiv
                P \vdash \Gamma
            \end{mathpar}

        \item
            $\pRes{x}(P \| Q) \equiv \pRes{x}(Q \| P)$.
            \begin{mathpar}
                \inferrule{
                    P \vdash \Gamma, x{:}A
                    \\
                    Q \vdash \Delta, x{:}\ol{A}
                }{
                    \pRes{x}(P \| Q) \vdash \Gamma, \Delta
                }
                \equiv
                \inferrule{
                    Q \vdash \Delta, x{:}\ol{A}
                    \\
                    P \vdash \Gamma, x{:}A
                }{
                    \pRes{x}(Q \| P) \vdash \Gamma, \Delta
                }
            \end{mathpar}

        \item
            $x \notin \fn{Q} \implies \pRes{x}(\pRes{y}(P \| Q) \| R) \equiv \pRes{y}(\pRes{x}(P \| R) \| Q)$.
            \begin{mathpar}
                \inferrule{
                    \inferrule*{
                        P \vdash \Gamma, y{:}A, x{:}B
                        \\
                        Q \vdash \Delta, y{:}\ol{A}
                    }{
                        \pRes{y}(P \| Q) \vdash \Gamma, \Delta, x{:}B
                    }
                    \\
                    R \vdash \Lambda, x{:}\ol{B}
                }{
                    \pRes{x}(\pRes{y}(P \| Q) \| R) \vdash \Gamma, \Delta, \Lambda
                }
                \equiv
                \inferrule{
                    \inferrule*{
                        P \vdash \Gamma, y{:}A, x{:}B
                        \\
                        R \vdash \Lambda, x{:}\ol{B}
                    }{
                        \pRes{x}(P \| R) \vdash \Gamma, \Lambda, y{:}A
                    }
                    \\
                    Q \vdash \Delta, y{:}\ol{A}
                }{
                    \pRes{y}(\pRes{x}(P \| R) \| Q) \vdash \Gamma, \Delta, \Lambda
                }
            \end{mathpar}

        \item
            $x \notin \fn{Q} \implies \pRes{x}((P \| Q) \| R) \equiv \pRes{x}(P \| R) \| Q$.
            \begin{mathpar}
                \inferrule{
                    \inferrule*{
                        P \vdash \Gamma, x{:}A
                        \\
                        Q \vdash \Delta
                    }{
                        P \| Q \vdash \Gamma, \Delta, x{:}A
                    }
                    \\
                    R \vdash \Lambda, x{:}\ol{A}
                }{
                    \pRes{x}((P \| Q) \| R) \vdash \Gamma, \Delta, \Lambda
                }
                \equiv
                \inferrule{
                    \inferrule*{
                        P \vdash \Gamma, x{:}A
                        \\
                        R \vdash \Lambda, x{:}\ol{A}
                    }{
                        \pRes{x}(P \| R) \vdash \Gamma, \Lambda
                    }
                    \\
                    Q \vdash \Delta
                }{
                    \pRes{x}(P \| R) \| Q \vdash \Gamma, \Delta, \Lambda
                }
            \end{mathpar}

        \item
            $x \notin \fn{Q} \implies \pRes{x}(\pSrv x(y);P \| Q) \equiv Q$.
            \begin{mathpar}
                \inferrule{
                    \inferrule*{
                        P \vdash {?}\Gamma, y{:}A
                    }{
                        \pSrv x(y);P \vdash {?}\Gamma, x{:}{!}A
                    }
                    \\
                    \inferrule*{
                        Q \vdash \Delta
                    }{
                        Q \vdash \Delta, x{:}{?}\ol{A}
                    }
                }{
                    \pRes{x}(\pSrv x(y);P \| Q) \vdash {?}\Gamma, \Delta
                }
                \equiv
                \inferruleDbl[vcenter]{
                    Q \vdash \Delta
                }{
                    Q \vdash {?}\Gamma, \Delta
                }
            \end{mathpar}

        \item
            $P \nd Q \equiv Q \nd P$.
            \begin{mathpar}
                \inferrule{
                    P \vdash \Gamma
                    \\
                    Q \vdash \Gamma
                }{
                    P \nd Q \vdash \Gamma
                }
                \equiv
                \inferrule{
                    Q \vdash \Gamma
                    \\
                    P \vdash \Gamma
                }{
                    Q \nd P \vdash \Gamma
                }
            \end{mathpar}

        \item
            $(P \nd Q) \nd R \equiv P \nd (Q \nd R)$
            \begin{mathpar}
                \inferrule{
                    \inferrule*{
                        P \vdash \Gamma
                        \\
                        Q \vdash \Gamma
                    }{
                        P \nd Q \vdash \Gamma
                    }
                    \\
                    R \vdash \Gamma
                }{
                    (P \nd Q) \nd R \vdash \Gamma
                }
                \equiv
                \inferrule{
                    P \vdash \Gamma
                    \\
                    \inferrule*{
                        Q \vdash \Gamma
                        \\
                        R \vdash \Gamma
                    }{
                        Q \nd R \vdash \Gamma
                    }
                }{
                    P \nd (Q \nd R) \vdash \Gamma
                }
            \end{mathpar}

        \item
            $P \nd P \equiv P$.
            \begin{mathpar}
                \inferrule{
                    P \vdash \Gamma
                    \\
                    P \vdash \Gamma
                }{
                    P \nd P \vdash \Gamma
                }
                \equiv
                P \vdash \Gamma
            \end{mathpar}
    \end{itemize}
    The inductive cases follow from the IH straightforwardly.
    Note that the rules for parallel composition do not apply directly behind the output prefix and restriction.
\end{proof}

\subsubsection{Subject Reduction}

\begin{lemma}\label{l:ctxType}
    Suppose $P \vdash \Gamma, x{:}A$.
    \begin{enumerate}
        \item\label{i:ctxTypePclose}
            If $P = \evalCtx{N}[\pClose x[]]$, then $A = \1$.

        \item\label{i:ctxTypeGclose}
            If $P = \evalCtx{N}[\pWait x();P']$, then $A = \bot$.

        \item\label{i:ctxTypePname}
            If $P = \evalCtx{N}[\pOut* x[y];(P' \| P'')]$, then $A = B \tensor C$.

        \item\label{i:ctxTypeGname}
            If $P = \evalCtx{N}[\pIn x(y);P']$, then $A = B \parr C$.

        \item\label{i:ctxTypePsel}
            If $P = \evalCtx{N}[\pSel* x < j;P']$, then $A = {\oplus}\{i:B_i\}_{i \in I}$ where $j \in I$.

        \item\label{i:ctxTypeGsel}
            If $P = \evalCtx{N}[\pBra* x > \{i:P'_i\}_{i \in I}]$, then $A = {\\&}\{i:B_i\}_{i \in I}$.

        \item\label{i:ctxTypePsome}
            If $P = \evalCtx{N}[\pSome x;P']$, then $A = {\\&}B$.

        \item\label{i:ctxTypePnone}
            If $P = \evalCtx{N}[\pNone x]$, then $A = {\\&}B$.

        \item\label{i:ctxTypeGsome}
            If $P = \evalCtx{N}[\pSomeIn x{w_1,\ldots,w_n}]$, then $A = {\oplus}B$.

        \item\label{i:ctxTypePuname}
            If $P = \evalCtx{N}[\pCli* x[y];P']$, then $A = {?}B$.

        \item\label{i:ctxTypeGuname}
            If $P = \evalCtx{N}[\pSrv x(y);P']$, then $A = {!}B$.
    \end{enumerate}
\end{lemma}

\begin{proof}
    Each item follows by induction on the structure of the ND-context.
    The base case follows by inversion of typing, and the inductive cases follow from the IH straightforwardly.
\end{proof}

\begin{lemma}\label{l:ctxRedOne}
    For each of the following items, assume $\Gamma \cap \Delta = \emptyset$.
    \begin{enumerate}
        \item\label{i:ctxRedOneFwd}
            If $\evalCtx[\big]{N}[\pFwd [x<>y]] \vdash \Gamma, x{:}A$ and $Q \vdash \Delta, x{:}\ol{A}$, then $\evalCtx*{N}[Q \{y/x\}] \vdash \Gamma, \Delta$.

        \item\label{i:ctxRedOnePclose}
            If $\evalCtx{N}[\pClose x[]] \vdash \Gamma, x{:}\1$, then $\evalCtx*{N}[\0] \vdash \Gamma$.

        \item\label{i:ctxRedOneGclose}
            If $\evalCtx{N}[\pWait x();Q] \vdash \Gamma, x{:}\bot$, then $\evalCtx*{N}[Q] \vdash \Gamma$.

        \item\label{i:ctxRedOneName}
            If $\bn{\evalCtx{N}} \cap \fn{\evalCtx{N}'} = \emptyset$ and $\evalCtx{N}[\pOut* x[y];(P \| Q)] \vdash \Gamma, x{:}A \tensor B$ and $\evalCtx{N'}[\pIn x(z);R] \vdash \Delta, x{:}\ol{A} \parr \ol{B}$, then $\evalCtx*{N}[\pRes{x}(Q \| \pRes{y}(P \| \evalCtx*{N'}[R\{y/z\}]))] \vdash \Gamma, \Delta$.

        \item\label{i:ctxRedOnePsel}
            If $\evalCtx{N}[\pSel* x < j; P] \vdash \Gamma, x{:}{\oplus}\{i: A_i\}_{i \in I}$ and $j \in I$, then $\evalCtx*{N}[P] \vdash \Gamma, x{:}A_j$.

        \item\label{i:ctxRedOneGsel}
            If $\evalCtx{N}[\pBra* x > \{i: P_i\}_{i \in I}] \vdash \Gamma, x{:}\\&\{i: A_i\}_{i \in I}$, then $\evalCtx*{N}[P_i] \vdash \Gamma, x{:}A_i$ for every $i \in I$.

        \item\label{i:ctxRedOnePsome}
            If $\evalCtx{N}[\pSome x; P] \vdash \Gamma, x{:}{\\&}A$, then $\evalCtx*{N}[P] \vdash \Gamma, x{:}A$.

        \item\label{i:ctxRedOnePnone}
            If $\evalCtx{N}[\pNone x] \vdash \Gamma, x{:}{\\&}A$, then $\evalCtx*{N}[\0] \vdash \Gamma$.

        \item\label{i:ctxRedOneGsome}
            If $\evalCtx{N}[\pSomeIn x{w_1,\ldots,w_n}; P] \vdash \Gamma, x{:}{\oplus} A$, then $\evalCtx*{N}[P] \vdash \Gamma, x{:}A$ and $\evalCtx*{N}[\pNone w_1 \| \ldots \| \pNone w_n] \vdash \Gamma$.

        \item\label{i:ctxRedOneUname}
            If $\bn{\evalCtx{N'}} \cap \fn{\evalCtx{N}} = \emptyset$ and $\evalCtx{N}[\pCli* x[y]; P] \vdash \Gamma, x{:}{?}A$ and $\evalCtx{N}'[\pSrv x(y); Q] \vdash \Delta, x{:}{!}\ol{A}$, then $\evalCtx*{N'}\big[\pRes{x}(\pRes{y}(\evalCtx*{N}[P] \| Q\{y/z\}) \| \pSrv x(z);Q)\big]$.
    \end{enumerate}
\end{lemma}

\begin{proof}
    For each item, we apply induction on the structure of the ND-contexts and detail the base cases.
    For simplicity, we assume no names in $\Gamma$ and $\Delta$ were derived with \ttype{weaken}.
    \begin{enumerate}
        \item
            \begin{mathpar}
                \inferrule*{ }{
                    \pFwd [x<>y] \vdash x{:}A, y{:}\ol{A}
                }
                \and
                \inferrule{}{
                    Q \vdash \Delta, x{:}\ol{A}
                }
                \and
                \implies
                \and
                \inferrule{}{
                    Q\{y/x\} \vdash \Delta, y{:}\ol{A}
                }
            \end{mathpar}

        \item
            \begin{mathpar}
                \inferrule*{ }{
                    \pClose x[] \vdash x{:}\1
                }
                \and\implies\and
                \inferrule*{ }{
                    \0 \vdash \emptyset
                }
            \end{mathpar}

        \item
            \begin{mathpar}
                \inferrule{
                    Q \vdash \Gamma
                }{
                    \pWait x();Q \vdash \Gamma, x{:}\bot
                }
                \and\implies\and
                \inferrule{}{
                    Q \vdash \Gamma
                }
            \end{mathpar}

        \item
            \begin{mathpar}
                \inferrule{
                    P \vdash \Gamma, y{:}A
                    \\
                    Q \vdash \Gamma', x{:}B
                }{
                    \pOut* x[y];(P \| Q) \vdash \Gamma, \Gamma', x{:}A \tensor B
                }
                \and
                \inferrule{
                    R \vdash \Delta, z{:}\ol{A}, x{:}\ol{B}
                }{
                    \pIn x(z);R \vdash \Delta, x{:}\ol{A} \parr \ol{B}
                }
                \and\implies\and
                \inferrule{
                    Q \vdash \Gamma', x{:}B
                    \\
                    \inferrule*{
                        P \vdash \Gamma, y{:}A
                        \\
                        R\{y/z\} \vdash \Delta, y{:}\ol{A}, x{:}\ol{B}
                    }{
                        \pRes{y}(P \| R\{y/z\}) \vdash \Gamma, \Delta, x{:}\ol{B}
                    }
                }{
                    \pRes{x}(Q \| \pRes{y}(P \| R\{y/z\})) \vdash \Gamma, \Gamma', \Delta
                }
            \end{mathpar}

        \item
            \begin{mathpar}
                \inferrule{
                    P \vdash \Gamma, x{:}A_j
                    \\
                    j \in I
                }{
                    \pSel* x < j;P \vdash \Gamma, x{:}{\oplus}\{i:A_i\}_{i \in I}
                }
                \and\implies\and
                \inferrule{}{
                    P \vdash \Gamma, x{:}A_j
                }
            \end{mathpar}

        \item
            \begin{mathpar}
                \inferrule{
                    \forall i \in I.~ P_i \vdash \Gamma, x{:}A_i
                }{
                    \pBra* x > \{i:P_i\}_{i \in I} \vdash \Gamma, x{:}{\\&}\{i:A_i\}
                }
                \and\implies\and
                \forall i \in I.~ \inferrule*{}{
                    P_i \vdash \Gamma, x{:}A_i
                }
            \end{mathpar}

        \item
            \begin{mathpar}
                \inferrule{
                    P \vdash \Gamma, x{:}A
                }{
                    \pSome x;P \vdash \Gamma, x{:}{\\&}A
                }
                \and\implies\and
                \inferrule{}{
                    P \vdash \Gamma, x{:}A
                }
            \end{mathpar}

        \item
            \begin{mathpar}
                \inferrule*{ }{
                    \pNone x \vdash x{:}{\\&}A
                }
                \and\implies\and
                \inferrule*{ }{
                    \0 \vdash \emptyset
                }
            \end{mathpar}

        \item
            \begin{mathpar}
                \inferrule{
                    P \vdash w_1{:}{\\&}B_1, \ldots, w_n{:}{\\&}B_n, x{:}A
                }{
                    \pSomeIn x{w_1,\ldots,w_n};P \vdash w_1{:}{\\&}B_1, \ldots, w_n{:}{\\&}B_n, x{:}{\oplus}A
                }
                \and\implies\and
                \inferrule{}{
                    P \vdash w_1{:}{\\&}B_1, \ldots, w_n{:}{\\&}B_n, x{:}A
                }
                \and
                \inferruleDbl{
                    \inferrule*[fraction={---}]{ }{
                        \pNone w_1 \vdash w_1{:}{\\&}B_1
                    }
                    \\
                    \ldots
                    \\
                    \inferrule*[fraction={---}]{ }{
                        \pNone w_n \vdash w_n{:}{\\&}B_n
                    }
                }{
                    \pNone w_1 \| \ldots \| \pNone w_n \vdash w_1{:}{\\&}B_1, \ldots, w_n{:}{\\&}B_n
                }
            \end{mathpar}

        \item
            This item depends on whether $x \in \fn{P}$.
            \begin{itemize}
                \item
                    $x \in \fn{P}$:
                    \begin{mathpar}
                        \and
                        \inferrule*{
                            \inferrule*{
                                P\{x'/x\} \vdash \Gamma, y{:}A, x'{:}{?}A
                            }{
                                \pCli* x[y];(P\{x'/x\}) \vdash \Gamma, x{:}{?}A, x'{:}{?}A
                            }
                        }{
                            \pCli* x[y];P \vdash \Gamma, x{:}{?}A
                        }
                        \and
                        \inferrule*{
                            Q \vdash {?}\Delta, z{:}\ol{A}
                        }{
                            \pSrv x(z);Q \vdash {?}\Delta, x{:}{!}\ol{A}
                        }
                        \and\implies\and
                        \inferruleDbl{
                            \inferrule*[fraction={---}]{
                                \inferrule*{
                                    P \vdash \Gamma, y{:}A, x{:}{?}A
                                    \\
                                    Q\{y/z\}\{w'/w\}_{w \in {?}\Delta} \vdash {?}\Delta', y{:}\ol{A}
                                }{
                                    \pRes{y}(P \| Q\{y/z\}\{w'/w\}_{w \in {?}\Delta}) \vdash \Gamma, {?}\Delta', x{:}{?}A
                                }
                                \\
                                \pSrv x(z);Q \vdash {?}\Delta, x{:}{!}\ol{A}
                            }{
                                \pRes{x}(\pRes{y}(P \| Q\{y/z\}\{w'/w\}_{w \in {?}\Delta}) \| \pSrv x(z);Q) \vdash \Gamma, {?}\Delta, {?}\Delta'
                            }
                        }{
                            \pRes{x}(\pRes{y}(P \| Q\{y/z\}) \| \pSrv x(z);Q) \vdash \Gamma, {?}\Delta
                        }
                    \end{mathpar}

                \item
                    $x \notin \fn{P}$:
                    \begin{mathpar}
                        \inferrule*{
                            P \vdash \Gamma, y{:}A
                        }{
                            \pCli* x[y];P \vdash \Gamma, x{:}{?}A
                        }
                        \and
                        \inferrule*{
                            Q \vdash {?}\Delta, z{:}\ol{A}
                        }{
                            \pSrv x(z);Q \vdash {?}\Delta, x{:}{!}\ol{A}
                        }
                        \and\implies\and
                        \inferruleDbl{
                            \inferrule*[fraction={---}]{
                                \inferrule*{
                                    \inferrule*{
                                        P \vdash \Gamma, y{:}A
                                        \\
                                        Q\{y/z\}\{w'/w\}_{w \in {?}\Delta} \vdash {?}\Delta', y{:}\ol{A}
                                    }{
                                        \pRes{y}(P \| Q\{y/z\}\{w'/w\}_{w \in {?}\Delta}) \vdash \Gamma, {?}\Delta'
                                    }
                                }{
                                    \pRes{y}(P \| Q\{y/z\}\{w'/w\}_{w \in {?}\Delta}) \vdash \Gamma, {?}\Delta', x{:}{?}A
                                }
                                \\
                                \pSrv x(z);Q \vdash {?}\Delta, x{:}{!}\ol{A}
                            }{
                                \pRes{x}(\pRes{y}(P \| Q\{y/z\}\{w'/w\}_{w \in {?}\Delta}) \| \pSrv x(z);Q) \vdash \Gamma, {?}\Delta, {?}\Delta'
                            }
                        }{
                            \pRes{x}(\pRes{y}(P \| Q\{y/z\}) \| \pSrv x(z);Q) \vdash \Gamma, {?}\Delta
                        }
                    \end{mathpar}
            \end{itemize}
    \end{enumerate}
    The inductive cases follow straightforwardly.
    Notice that the conditions on the bound and free names of the ND-contexts in \cref{i:ctxRedOneName,i:ctxRedOneUname} make sure that no names are captured when embedding one context in the other.
\end{proof}

\begin{theorem}[SR for the Eager Semantics]\label{t:srOne}
    If $P \vdash \Gamma$ and $P \reddEager Q$, then $Q \vdash \Gamma$.
\end{theorem}

\begin{proof}
    By induction on the derivation of the reduction.
    \begin{itemize}
        \item
            Rule $\rredone{\scc{Id}}$.
            \begin{mathpar}
                \inferrule{
                    \evalCtx[\big]{N}[\pFwd [x<>y]] \vdash \Gamma, x{:}A
                    \\
                    Q \vdash \Delta, x{:}\ol{A}
                }{
                    \pRes{x}(\evalCtx[\big]{N}[\pFwd [x<>y]] \| Q) \vdash \Gamma, \Delta
                }
                \and\implies\and
                \inferrule{}{
                    \evalCtx*{N}[Q\{y/x\}] \vdash \Gamma, \Delta
                    ~~\text{(\refitem{l}{ctxRedOne}{Fwd})}
                }
            \end{mathpar}

        \item
            Rule $\rredone{\1\bot}$.
            \begin{mathpar}
                \inferrule{
                    \evalCtx{N}[\pClose x[]] \vdash \Gamma, x{:}\1
                    ~~\text{(\refitem{l}{ctxType}{Pclose})}
                    \\
                    \evalCtx{N'}[\pWait x();Q] \vdash \Delta, x{:}\bot
                    ~~\text{(\refitem{l}{ctxType}{Gclose})}
                }{
                    \nu{x}(\evalCtx{N}[\pClose x[]] \| \evalCtx{N'}[\pWait x();Q]) \vdash \Gamma, \Delta
                }
                \and\implies\and
                \inferrule{
                    \evalCtx*{N}[\0] \vdash \Gamma
                    ~~\text{(\refitem{l}{ctxRedOne}{Pclose})}
                    \\
                    \evalCtx*{N'}[Q] \vdash \Delta
                    ~~\text{(\refitem{l}{ctxRedOne}{Gclose})}
                }{
                    \evalCtx*{N}[\0] \| \evalCtx*{N'}[Q] \vdash \Gamma, \Delta
                }
            \end{mathpar}

        \item
            Rule $\rredone{\tensor\parr}$.
            \begin{mathpar}
                \inferrule{
                    \evalCtx{N}[\pOut* x[y];(P \| Q)] \vdash \Gamma, x{:}A \tensor B
                    ~~\text{(\refitem{l}{ctxType}{Pname})}
                    \\
                    \evalCtx{N'}[\pIn x(z);R] \vdash \Delta, x{:}\ol{A} \parr \ol{B}
                    ~~\text{(\refitem{l}{ctxType}{Gname})}
                }{
                    \pRes{x}(\evalCtx{N}[\pOut* x[y];(P \| Q)] \| \evalCtx{N'}[\pIn x(z);R]) \vdash \Gamma, \Delta
                }
                \and\implies\and
                \inferrule{}{
                    \evalCtx*{N}[\pRes{x}(Q \| \nu{y}(P \| \evalCtx*{N'}[R\{y/z\}]))] \vdash \Gamma, \Delta
                    ~~\text{(\refitem{l}{ctxRedOne}{Name})}
                }
            \end{mathpar}

        \item
            Rule $\rredone{{\oplus}{\\&}}$.
            \begin{mathpar}
                \inferrule{
                    \evalCtx{N}[\pSel* x < j;P] \vdash \Gamma, x{:}{\oplus}\{i:A_i\}_{i \in I}
                    ~~ j \in I
                    ~~\text{(\refitem{l}{ctxType}{Psel})}
                    \\
                    \evalCtx{N'}[\pBra* x > \{i:Q_i\}_{i \in I}] \vdash \Delta, x{:}{\\&}\{i:\ol{A_i}\}_{i \in I}
                    ~~\text{(\refitem{l}{ctxType}{Gsel})}
                }{
                    \pRes{x}(\evalCtx{N}[\pSel* x < j;P] \| \evalCtx{N'}[\pBra* x > \{i:Q_i\}_{i \in I}]) \vdash \Gamma, \Delta
                }
                \and\implies\and
                \inferrule{
                    \evalCtx*{N}[P] \vdash \Gamma, x{:}A_j
                    ~~\text{(\refitem{l}{ctxRedOne}{Psel})}
                    \\
                    \evalCtx*{N'}[Q_j] \vdash \Delta, x{:}\ol{A_j}
                    ~~\text{(\refitem{l}{ctxRedOne}{Gsel})}
                }{
                    \pRes{x}(\evalCtx*{N}[P] \| \evalCtx*{N'}[Q_j]) \vdash \Gamma, \Delta
                }
            \end{mathpar}

        \item
            Rule $\rredone{\some}$.
            \begin{mathpar}
                \inferrule{
                    \evalCtx{N}[\pSome x;P] \vdash \Gamma, x{:}{\\&}A
                    ~~\text{(\refitem{l}{ctxType}{Psome})}
                    \\
                    \evalCtx{N'}[\pWait x(){(w_1,\ldots,w_n)};Q] \vdash \Delta, x{:}{\oplus}\ol{A}
                    ~~\text{(\refitem{l}{ctxType}{Gsome})}
                }{
                    \pRes{x}(\evalCtx{N}[\pSome x;P] \| \evalCtx{N'}[\pWait x(){(w_1,\ldots,w_n)};Q]) \vdash \Gamma, \Delta
                }
                \and\implies\and
                \inferrule{
                    \evalCtx*{N}[P] \vdash \Gamma, x{:}A
                    ~~\text{(\refitem{l}{ctxRedOne}{Psome})}
                    \\
                    \evalCtx*{N'}[Q] \vdash \Delta, x{:}\ol{A}
                    ~~\text{(\refitem{l}{ctxRedOne}{Gsome})}
                }{
                    \pRes{x}(\evalCtx*{N}[P] \| \evalCtx*{N'}[Q]) \vdash \Gamma, \Delta
                }
            \end{mathpar}

        \item
            Rule $\rredone{\none}$.
            \begin{mathpar}
                \inferrule{
                    \evalCtx{N}[\pNone x] \vdash \Gamma, x{:}{\\&}A
                    ~~\text{(\refitem{l}{ctxType}{Pnone})}
                    \\
                    \evalCtx{N'}[\pWait x(){(w_1,\ldots,w_n)};Q] \vdash \Delta, x{:}{\oplus}\ol{A}
                    ~~\text{(\refitem{l}{ctxType}{Gsome})}
                }{
                    \pRes{x}(\evalCtx{N}[\pNone x] \| \evalCtx{N'}[\pWait x(){(w_1,\ldots,w_n)};Q]) \vdash \Gamma, \Delta
                }
                \and\implies\and
                \inferrule{
                    \evalCtx*{N}[\0] \vdash \Gamma
                    ~~\text{(\refitem{l}{ctxRedOne}{Pnone})}
                    \\
                    \evalCtx*{N'}[\pNone w_1 \| \ldots \| \pNone w_n] \vdash \Delta
                    ~~\text{(\refitem{l}{ctxRedOne}{Gsome})}
                }{
                    \evalCtx*{N}[\0] \| \evalCtx*{N'}[\pNone w_1 \| \ldots \| \pNone w_n]) \vdash \Gamma, \Delta
                }
            \end{mathpar}

        \item
            Rule $\rredone{{?}{!}}$.
            \begin{mathpar}
                \inferrule{
                    \evalCtx{N}[\pCli* x[y];P] \vdash \Gamma, x{:}{?}A
                    ~~\text{(\refitem{l}{ctxType}{Puname})}
                    \\
                    \evalCtx{N'}[\pSrv x(z);Q] \vdash \Delta, x{:}{!}\ol{A}
                    ~~\text{(\refitem{l}{ctxType}{Guname})}
                }{
                    \pRes{x}(\evalCtx{N}[\pCli* x[y];P] \| \evalCtx{N'}[\pSrv x(y);Q]) \vdash \Gamma, \Delta
                }
                \and\implies\and
                \inferrule{}{
                    \evalCtx*{N'}\big[\pRes{x}(\pRes{y}(\evalCtx*{N}[P] \| Q\{y/z\}) \| \pSrv x(z);Q)\big] \vdash \Gamma, \Delta
                    ~~\text{(\refitem{l}{ctxRedOne}{Uname})}
                }
            \end{mathpar}

        \item
            Rule $\rredone{\equiv}$.
            Assume $P \equiv P'$ and $P' \reddEager Q'$ and $Q' \equiv Q$.
            By \Cref{t:subcong}, $P' \vdash \Gamma$.
            By the IH, $Q' \vdash \Gamma$.
            By \Cref{t:subcong}, $Q \vdash \Gamma$.

        \item
            Rule $\rredone{\nu}$.
            Assume $P \reddEager P'$.
            \begin{mathpar}
                \inferrule{
                    P \vdash \Gamma, x{:}A
                    \\
                    Q \vdash \Delta, x{:}\ol{A}
                }{
                    \pRes{x}(P \| Q) \vdash \Gamma, \Delta
                }
                \and\implies\and
                \inferrule{
                    P' \vdash \Gamma, x{:}A
                    ~~\text{(IH)}
                    \\
                    Q \vdash \Delta, x{:}\ol{A}
                }{
                    \pRes{x}(P' \| Q) \vdash \Gamma, \Delta
                }
            \end{mathpar}

        \item
            Rule $\rredone{\|}$.
            Assume $P \reddEager P'$.
            \begin{mathpar}
                \inferrule{
                    P \vdash \Gamma
                    \\
                    Q \vdash \Delta
                }{
                    P \| Q \vdash \Gamma, \Delta
                }
                \and\implies\and
                \inferrule{
                    P' \vdash \Gamma
                    ~~\text{(IH)}
                    \\
                    Q \vdash \Delta
                }{
                    P' \| Q \vdash \Gamma, \Delta
                }
            \end{mathpar}

        \item
            Rule $\rredone{\nd}$.
            Assume $P \reddEager P'$.
            \begin{mathpar}
                \inferrule{
                    P \vdash \Gamma
                    \\
                    Q \vdash \Gamma
                }{
                    P \nd Q \vdash \Gamma
                }
                \and\implies\and
                \inferrule{
                    P' \vdash \Gamma
                    ~~\text{(IH)}
                    \\
                    Q \vdash \Gamma
                }{
                    P' \nd Q \vdash \Gamma
                }
            \end{mathpar}
            \qedhere
    \end{itemize}
\end{proof}

\subsubsection{Deadlock-freedom}

%<*clpi:dfEager>
The proof uses several definitions and lemmas, which we summarize:
\begin{itemize}
    \item
        \Cref{d:clpi:sCtx} defines single-choice multi-hole contexts, where holes may only appear on one side of non-deterministic choices.
        \Cref{d:clpi:sColl} yields deterministic multi-hole contexts from single-choice multi-hole contexts by collapsing non-deterministic choices to the sides of holes.
        \Cref{l:clpi:sColl} ensures typing remains consistent when collapsing a single-choice multi-hole context.

    \item
        \Cref{l:clpi:sCtxForm} states that any typable process not equivalent to $\0$ can be written as an S-context with each hole replaced by a prefixed process.
        Let us refer to this as the \emph{S-context form}.

    \item
        \Cref{l:clpi:sFormFwd} states that if a process in S-context form is typable under empty context and has a forwarder as one of its prefixes, that process contains a cut on one of the forwarder's subjects.

    \item
        \Cref{l:clpi:sCtxCuts} states that the number of prefixed processes of a process in S-context form is at least the number of cuts in the S-context.
        This lemma is key to the proof of deadlock-freedom, as it is necessary to show the next lemma.

    \item
        \Cref{l:clpi:sCtxSubjs} states that if a process in S-context form is typable under empty context, then there must be two of its prefixed processes that share a subject.

    \item
        \Cref{t:clpi:dfEager} proves deadlock-freedom for the eager semantics.

\end{itemize}

\begin{definition}[Single-choice Multi-hole Contexts]
    \label{d:clpi:sCtx}
    We define \emph{single-choice multi-hole contexts} (S-contexts, for short) as follows:
    \[
        \evalCtx{S} ::= {\evalHole}_i \sepr \pRes{x} ( \evalCtx{S} \| \evalCtx{S} ) \sepr \evalCtx{S} \| \evalCtx{S} \sepr \evalCtx{S} \nd P
    \]
    An S-context is $n$-ary if it has $n$ holes ${\evalHole}_1, \ldots, {\evalHole}_n$.
    We write $\evalCtx{S}[P_1, \ldots, P_n]$ to denote the process obtained from the $n$-ary multi-hole context $\evalCtx{S}$ by replacing each $i$-th hole in $\evalCtx{S}$ with $P_i$.
    Given an S-context $\evalCtx{S}$ with hole indices $I$ and a sequence of processes ${(P_i)}_{i \in I}$, we write $\evalCtx{S}[P_i]_{i \in I}$ to denote the process obtained from $\evalCtx{S}$ by replacing each hole with index $i$ in $\evalCtx{S}$ with $P_i$.
    We say an S-context is a \emph{deterministic multi-hole context} (DM-context, for short) if its holes do not appear inside any non-deterministic choices.
\end{definition}

\begin{definition}[Collapse of Single-choice Multi-hole Contexts]
    \label{d:clpi:sColl}
    We define the \emph{collapse} of S-context $\evalCtx{S}$, by abuse of notation denoted $\evalCtx{\D{S}}$, as follows, yielding a deterministic multi-hole context:
    \begin{align*}
        \D{{\evalHole}_i} &\deq {\evalHole}_i
        & \D{\evalCtx{S} \| \evalCtx{S}'} &\deq \evalCtx{\D{S}} \| \evalCtx{\D{S'}}
        & \D{\pRes{x} ( \evalCtx{S} \| \evalCtx{S}' )} &\deq \pRes{x} ( \evalCtx{\D{S}} \| \evalCtx{\D{S'}} )
        & \D{\evalCtx{S} \nd P} &\deq \evalCtx{\D{S}}
    \end{align*}
\end{definition}

\begin{lemma}
    \label{l:clpi:sColl}
    If $\vdash \evalCtx{S}[P_i]_{i \in I} \typInf \Gamma$, then $\vdash \evalCtx{\D{S}}[P_i]_{i \in I} \typInf \Gamma$.
\end{lemma}

\begin{proof}
    Straightforward, by induction on the structure of $\evalCtx{S}$.
\end{proof}

\begin{lemma}
    \label{l:clpi:sCtxForm}
    If $\vdash P \typInf \Gamma$ and $P \not\equiv \0$, then there exist S-context $\evalCtx{S}$ with indices $I$ and sequence of prefixed processes ${(\alpha_i ; P_i)}_{i \in I}$ such that $P \equiv \evalCtx{S}[\alpha_i ; P_i]_{i \in I}$.
\end{lemma}

\begin{proof}
    Using structural congruence, we first remove all cuts with unused servers and parallel compositions with $\0$, obtaining $P' \equiv P$.
    Since $P \not\equiv \0$, $P' \not\equiv \0$.
    Then, we construct $\evalCtx{S}$ by induction on the typing derivation of $P'$.
    Rules~\ruleLabel{typ-inact} and~\ruleLabel{typ-weaken} do not occur, because of how we obtained $P'$ from $P$.
    The structural rules~\ruleLabel{typ-par}, \ruleLabel{typ-cut} are simply copied.
    In case of Rule~\ruleLabel{typ-nd}, we arbitrarily pick a branch to continue the construction of $\evalCtx{S}$ with, while copying the entire other branch.
    The other rules, which type prefixes, add a hole to $\evalCtx{S}$; we mark the hole with index $i$ and refer to the prefixed process typed by the rule as $\alpha_i ; P_i$.
    Clearly, $P \equiv P' = \evalCtx{S}[\alpha_i ; P_i]_{i \in I}$.
\end{proof}

\begin{lemma}
    \label{l:clpi:sFormFwd}
    If $\vdash P = \evalCtx{S}[\alpha_i ; P_i]_{i \in I} \typInf \emptyset$ and there is $j \in I$ s.t.\ $\alpha_j = \pFwd [x<>y]$, then there are $\evalCtx{N},\evalCtx{N'},Q$ such that $P = \evalCtx[\Big]{N}[\pRes{x} ( \evalCtx[\big]{N'}[\pFwd [x<>y]] \| Q )]$.
\end{lemma}

\begin{proof}
    Note that there must be a restriction on $x$ in $P$, because $x$ appears free in $\pFwd [x<>y]$ but $\vdash P \typInf \emptyset$.
    First, we obtain $\evalCtx{N}$ from $P$ by replacing the restriction on $x$ in $P$ with a hole, referring to the parallel component in which $\pFwd [x<>y]$ appears as $P'$ and to the other parallel component as $Q$.
    Then, we obtain $\evalCtx{N'}$ from $P'$ by replacing $\pFwd [x<>y]$ with a hole.
    Clearly, $P = \evalCtx[\Big]{N}[\pRes{x} ( \evalCtx[\big]{N'}[\pFwd [x<>y]] \| Q )]$.
\end{proof}

\begin{lemma}
    \label{l:clpi:sCtxCuts}
    If the derivation of $\vdash P = \evalCtx{S}[\alpha_i ; P_i]_{i \in I} \typInf \Gamma$ and $\evalCtx{S}$ is deterministic and contains $n$ cuts, then $|I| \geq n+1$.
\end{lemma}

\begin{proof}
    We apply strong induction on the number $n$ of cuts in $\evalCtx{S}$:
    \begin{itemize}

        \item
            Case $n = 0$.
            Any S-context must have at least one hole, so $\evalCtx{S}$ has at least one hole.
            Hence, $|I| \geq 1 = n + 1$.

        \item
            Case $n = n' + 1$.
            By abuse of notation, $P = P_1 \| \ldots \| P_k$, where for each $1 \leq k' \leq k$, $P_{k'}$ is not a parallel composition.
            By assumption, $m \geq 1$ of the $P_1,\ldots,P_k$ are cuts.
            W.l.o.g., assume $P_1,\ldots,P_m$ are cuts.

            For each $1 \leq j \leq m$, by inversion of Rule~\ruleLabel{typ-par}, $\vdash P_j \typInf \Gamma_j$, and by construction, there are $\evalCtx{S_j},I_j$ s.t.\ $P_j = \evalCtx{S_j}[\alpha_i ; P_i]_{i \in I_j}$ where $\evalCtx{S_j}$ is deterministic.
            We have for each $1 \leq j \leq m$ and $1 \leq j' \leq m$ where $j \neq j'$ that $I_j \cap I_{j'} = \emptyset$, and $\bigcup_{1 \leq j \leq m} I_j \subseteq I$.
            Then, for each $1 \leq j \leq m$, let $1 \leq n_j \leq n$ be the number of cuts in $\evalCtx{S_j}$.
            Since $P_{m+1},\ldots,P_k$ are not cuts, we have $\sum_{1 \leq j \leq m} n_j = n$.

            Take any $1 \leq j \leq m$.
            We have $P_j = \pRes{x} ( P'_j \| P''_j )$, and by inversion of Rule~\ruleLabel{typ-cut}, $\vdash P'_j \typInf \Gamma'_j, x:A$ and $\vdash P''_j \typInf \Gamma''_j, x:\ol{A}$ where $\Gamma_j = \Gamma'_j, \Gamma''_j$.
            By construction, there are $\evalCtx{S'_j},\evalCtx{S''_j},I'_j,I''_j$ s.t.\ $P'_j = \evalCtx{S'_j}[\alpha_i ; P_i]_{i \in I'_j}$ and $P''_j = \evalCtx{S''_j}[\alpha_i ; P_i]_{i \in I''_j}$ and $\evalCtx{S'_j}$ and $\evalCtx{S''_j}$ are deterministic.
            We have $I'_j \cap I''_j = \emptyset$ and $I'_j \cup I''_j = I_j$.

            Let $n'_j$ and $n''_j$ be the number of cuts in $\evalCtx{S'_j}$ and $\evalCtx{S''_j}$, respectively.
            We have that \mbox{$n'_j + n''_j + 1 = n_j$}.
            Since $n_j \leq n = n' + 1$, then $n'_j,n''_j \leq n'$.
            Then, by the IH, $|I'_j| \geq n'_j + 1$ and $|I''_j| \geq n''_j + 1$.
            Therefore, $|I_j| = |I'_j \cup I''_j| = |I'_j| + |I''_j| \geq n'_j + n''_j + 1 + 1 = n_j + 1$.

            In conclusion,
            \[
                |I| \geq |\bigcup_{1 \leq j \leq m} I_j| = \sum_{1 \leq j \leq m} |I_j| \geq \sum_{1 \leq j \leq m} (n_j + 1) = \sum_{1 \leq j \leq m} n_j + m = n + m \geq n + 1.
                \tag*{\qedhere}
            \]

    \end{itemize}
\end{proof}

\begin{lemma}
    \label{l:clpi:sCtxSubjs}
    If $\vdash P = \evalCtx{S}[\alpha_i ; P_i]_{i \in I} \typInf \emptyset$ where for each $i \in I$, $\alpha_i \neq \pFwd [x<>y]$ for any $x$ and $y$, then there are $j,k \in I$ where $j \neq k$ and $x = \subjs(\alpha_j) = \subjs(\alpha_k)$, and there are $\evalCtx{N},\evalCtx{N_j},\evalCtx{N_k}$ such that $P = \evalCtx[\big]{N}[\pRes{x} ( \evalCtx{N_j}[\alpha_j] \| \evalCtx{N_k}[\alpha_k] )]$.
\end{lemma}

\begin{proof}
    Let $Q = \evalCtx{\D{S}}[{(\alpha_i)}_{i \in I}]$.
    Then $Q$ is deterministic and, by \Cref{l:clpi:sColl}, $\vdash Q \typInf \emptyset$.
    Let $n$ be the number of cuts in $\evalCtx{S}$.
    By \Cref{l:clpi:sCtxCuts}, $|I| \geq n + 1$.

    Suppose, for contradiction, that for every $j,k \in I$ where $j \neq k$, we have $\subjs(\alpha_j) \neq \subjs(\alpha_k)$.
    Since $\vdash Q \typInf \emptyset$, for each $j \in I$, $\subjs(\alpha_j)$ must be bound by a cut, so $\evalCtx{S}$ must contain $|I|$ cuts.
    This means $|I| = n$, contradicting the fact that $|I| \geq n + 1$.
    Therefore, there must be $j,k \in I$ where $j \neq k$ such that $\subjs(\alpha_j) = \subjs(\alpha_k)$.

    Hence, we can take $x = \subjs(\alpha_j) = \subjs(\alpha_k)$.
    Since $\vdash P \typInf \emptyset$ but $x$ appears free in $\alpha_j ; P_j$ and $\alpha_k ; P_k$, there must be a restriction on $x$ in $\evalCtx{S}$ containing the holes ${\evalHole}_j$ and ${\evalHole}_k$.
    We now obtain $\evalCtx{N}$ from $P$ by replacing the restriction on $x$ in $P$ with a hole, referring to the parallel component in which $\alpha_j ; P_j$ appears as $P_j$ and the component in which $\alpha_k ; P_k$ appears as $P_k$.
    Then, we obtain $\evalCtx{N_j}$ and $\evalCtx{N_k}$ from $P_j$ and $P_k$, respectively, by replacing $\alpha_j ; P_j$ and $\alpha_k ; P_k$ with a hole.
    Clearly, $P = \evalCtx[\big]{N}[\pRes{x} ( \evalCtx{N_j}[\alpha_j ; P_j] \| \evalCtx{N_k}[\alpha_k ; P_k] )]$.
\end{proof}

\tClpiDfEager*

\begin{proof}
    By \Cref{l:clpi:sCtxForm}, there are S-context $\evalCtx{S}$ with hole indices $I$ and sequence of prefixed processes ${(\alpha_i ; P_i)}_{i \in I}$ such that $P \equiv \evalCtx{S}[\alpha_i ; P_i]_{i \in I}$.
    The next step depends on whether there is a forwarder process among the $\alpha_i$.
    \begin{itemize}

        \item
            If there exists $j \in I$ s.t.\ $\alpha_j = \pFwd [x<>y]$ for some $x$ and $y$, then by \Cref{l:clpi:sFormFwd} there are $\evalCtx{N},\evalCtx{N'},Q$ s.t.\ $\evalCtx{S}[\alpha_i ; P_i] = \evalCtx[\Big]{N}[\pRes{x} ( \evalCtx[\big]{N'}[\pFwd [x<>y]] \| Q )]$.
            \begin{align*}
                \pRes{x} ( \evalCtx[\big]{N'}[\pFwd [x<>y]] \| Q ) &\reddEager \evalCtx*{N'}[Q \{ y/x \}] \deq R'
                \\
                \evalCtx{S}[\alpha_i ; P_i]_{i \in I} = \evalCtx[\Big]{N}[\pRes{x} ( \evalCtx[\big]{N'}[\pFwd [x<>y]] \| Q )] &\reddEager \evalCtx{N}[R'] \deq R
                \\
                P &\reddEager R
            \end{align*}

        \item
            If for each $i \in I$, $\alpha_i \neq \pFwd [x<>y]$ for any $x$ and $y$, then by \Cref{l:clpi:sCtxSubjs} there are $j,k \in I$ where $j \neq k$ and $x = \subjs(\alpha_j) = \subjs(\alpha_k)$ for some $x$, and $\evalCtx{N},\evalCtx{N_j},\evalCtx{N_k}$ such that $\evalCtx{S}[\alpha_i ; P_i]_{i \in I} = \evalCtx[\big]{N}[\pRes{x} ( \evalCtx{N_j}[\alpha_j ; P_j] \| \evalCtx{N_k}[\alpha_k ; P_k] )]$.

            We now show by cases on $\alpha_j$ that there is $R'$ such that
            \[
                \pRes{x} ( \evalCtx{N_j}[\alpha_j ; P_j] \| \evalCtx{N_k}[\alpha_k ; P_k] ) \reddEager R'.
            \]
            First, note that by typability, if the type for $x$ in $\evalCtx{N_j}[\alpha_j ; P_j]$ is $A$, then the type for $x$ in $\evalCtx{N_k}[\alpha_k ; P_k]$ is $\ol{A}$.
            In the following cases, we determine more precisely the form of $A$ by typing inversion on $\evalCtx{N_j}[\alpha_j ; P_j]$, and then determine the form of $\alpha_k$ by typing inversion using the form of $\ol{A}$.
            Note that we can exclude any cases where $\alpha_j$ or $\alpha_k$ are forwarder processes, as we assume they are not.
            \begin{itemize}

                \item
                    If $\alpha_j ; P_j = \pClose x[]$, then $A = \1$ and $\ol{A} = \bot$.
                    Hence, $\alpha_k ; P_k = \pWait x() ; P_k$.
                    By Rule~\ruleLabel{red-eager-close-wait}, there is $R'$ such that
                    \begin{align*}
                        \pRes{x} ( \evalCtx{N_j}[\pClose x[]] \| \evalCtx{N_k}[\pWait x() ; P_k] ) \reddEager R'.
                    \end{align*}

                \item
                    If $\alpha_j ; P_j = \pOut* x[y] ; ( P'_j \| P''_j )$ for some $y$, then $A = B \tensor C$ and $\ol{A} = \ol{B} \parr \ol{C}$ for some $B$ and~$C$.
                    Hence, $\alpha_k ; P_k = \pIn x(z) ; P_k$ for some $z$.
                    By Rule~\ruleLabel{red-eager-send-recv}, there is~$R'$ such that
                    \begin{align*}
                        \pRes{x} ( \evalCtx{N_j}[\pOut* x[y] ; ( P'_j \| P''_j )] \| \evalCtx{N_k}[\pIn x(z) ; P_k]) \reddEager R'.
                    \end{align*}

                \item
                    If $\alpha_j ; P_j = \pSel* x < l' ; P_j$, then $A = \oplus \{ l : B_l \}_{l \in L}$ and $\ol{A} = \& \{ l : \ol{B_l} \}_{l \in L}$ for some ${(B_l)}_{l \in L}$ where $l' \in L$.
                    Hence, $\alpha_k ; P_k = \pBra* x > \{ l : P_k^l \}_{l \in L}$.
                    By Rule~\ruleLabel{red-eager-sel-bra}, there is~$R'$ such that
                    \begin{align*}
                        \pRes{x} ( \evalCtx{N_j}[\pSel* x < l' ; P_j] \| \evalCtx{N_k}[\pBra* x > \{ l : P_k^l \}_{l \in L}] ) \reddEager R'.
                    \end{align*}

                \item
                    If $\alpha_j ; P_j = \pSome x ; P_j$, then $A = \oplus B$ and $\ol{A} = \& \ol{B}$ for some $B$.
                    Hence, \mbox{$\alpha_k = \pSomeIn x{w_1,\ldots,w_n} ; P_k$} for some $w_1,\ldots,w_n$.
                    By Rule~\ruleLabel{red-eager-some}, there is $R'$ such that
                    \begin{align*}
                        \pRes{x} ( \evalCtx{N_j}[\pSome x ; P_j] \| \evalCtx{N_k}[\pSomeIn x{w_1,\ldots,w_n} ; P_k] ) \reddEager R'.
                    \end{align*}

                \item
                    If $\alpha_j ; P_j = \pNone x$, then $A = \oplus B$ and $\ol{A} = \& \ol{B}$ for some $B$.
                    Hence, \mbox{$\alpha_k = \pSomeIn x{w_1,\ldots,w_n} ; P_k$} for some $w_1,\ldots,w_n$.
                    By Rule~\ruleLabel{red-eager-none}, there is $R'$ such that
                    \begin{align*}
                        \pRes{x} ( \evalCtx{N_j}[\pNone x] \| \evalCtx{N_k}[\pSomeIn x{w_1,\ldots,w_n} ; P_k] ) \reddEager R'.
                    \end{align*}

                \item
                    If $\alpha_j ; P_j = \pCli* x[y] ; P_j$ for some $y$, then $A = {?}B$ and $\ol{A} = {!}\ol{B}$ for some $B$.
                    Hence, \mbox{$\alpha_k ; P_k = \pSrv x(z) ; P_k$} for some $z$.
                    By Rule~\ruleLabel{red-eager-cli-srv}, there is $R'$ such that
                    \begin{align*}
                        \pRes{x} ( \evalCtx{N_j}[\pCli* x[y] ; P_j] \| \evalCtx{N_k}[\pSrv x(z) ; P_k] ) \reddEager R'.
                    \end{align*}

                \item
                    Otherwise, $\alpha_j$ is a receiving prefix and $\alpha_k$ is thus a sending prefix.
                    By cases on $\alpha_k$, the proof is analogous to above.

            \end{itemize}
            In conclusion,
            \begin{align*}
                \evalCtx{S}[\alpha_i ; P_i]_{i \in I} = \evalCtx[\big]{N}[\pRes{x} ( \evalCtx{N_j}[\alpha_j ; P_j] \| \evalCtx{N_k}[\alpha_k ; P_k] )] &\reddEager \evalCtx{N}[R'] \deq R
                \\
                P &\reddEager R.
                \tag*{\qedhere}
            \end{align*}

    \end{itemize}
\end{proof}
%</clpi:dfEager>

\subsection{Lazy Semantics}
\label{ss:proofsLazy}

\subsubsection{Subject Reduction}
\label{ss:TPLazy}

\begin{lemma}\label{l:ctxRedTwo}
    For both of the following items, assume $\Gamma \cap \Delta = \emptyset$.
    \begin{enumerate}
        \item\label{i:ctxRedTwoName}
            If $\forall i \in I.~ \forall j \in J.~ \bn{\evalCtx{C_i}} \cap \fn{\evalCtx{D_j}} = \emptyset$ and $\forall i \in I.~ \evalCtx{C_i}[\pOut* x[y_i];(P_i \| Q_i)] \vdash \Gamma, x{:}A \tensor B$ and $\forall j \in J.~ \evalCtx{D_j}[\pIn x(z);R_j] \vdash \Delta, x{:}\ol{A} \parr \ol{B}$, then $\bignd_{i \in I} \evalCtx[\Big]{C_i}[\pRes{x}\Big(Q_i \| \pRes{w}\Big(P_i\{w/y_i\} \| \bignd_{j \in J} \evalCtx{D_j}[R_j\{w/z\}]\Big)\Big)] \vdash \Gamma, \Delta$.

        \item\label{i:ctxRedTwoUname}
            If $\forall i \in I.~ \forall j \in J.~ \bn{\evalCtx{D_j}} \cap \fn{\evalCtx{C_i}} = \emptyset$ and $\forall i \in I.~ \evalCtx{C_i}[\pCli* x[y_i];P_i] \vdash \Gamma, x{:}{?}A$ and $\forall j \in J.~ \evalCtx{D_j}[\pSrv x(z);Q_j] \vdash \Delta, x{:}{!}\ol{A}$, then $\bignd_{j \in J} \evalCtx[\Big]{D_j}[\pRes{x}\Big(\pRes{w}\Big(\bignd_{i \in I} \evalCtx{C_i}[P_i\{w/y_i\}] \| Q_j\{w/z\}\Big) \| \pSrv x(z);Q_j\Big)] \vdash \Gamma, \Delta$.
    \end{enumerate}
\end{lemma}

\begin{proof}
    Both items follow by induction on the structures of the D-contexts.
    For each item, we detail the base case, where $\forall i \in I.~ \evalCtx{C_i} = \hole$ and $\forall j \in J.~ \evalCtx{D_j} = \hole$.
    The inductive cases follow from the IH straightforwardly.
    \begin{enumerate}
        \item
            \begin{mathpar}
                \forall i \in I.~
                \inferrule{
                    P_i \vdash \Gamma, y_i{:}A
                    \\
                    Q_i \vdash \Delta, x{:}B
                }{
                    \pOut* x[y_i];(P_i \| Q_i) \vdash \Gamma, \Delta, x{:}A \tensor B
                }
                \and
                \forall j \in J.~
                \inferrule{
                    R_j \vdash \Lambda, z{:}\ol{A}, x{:}\ol{B}
                }{
                    \pIn x(z);R_j \vdash \Lambda, x{:}\ol{A} \parr \ol{B}
                }
                \and\implies\and
                \inferruleDbl{
                    \inferrule*[fraction={---}]{
                        \forall i \in I.~
                        Q_i \vdash \Delta, x{:}B
                        \\
                        \inferrule*{
                            \forall i \in I.~
                            P_i\{w/y_i\} \vdash \Gamma, w{:}A
                            \\
                            \inferruleDbl{
                                \forall j \in J.~ R_j\{w/z\} \vdash \Lambda, w{:}\ol{A}, x{:}\ol{B}
                            }{
                                \bignd_{j \in J} R_j\{w/z\} \vdash \Lambda, w{:}\ol{A}, x{:}\ol{B}
                            }
                        }{
                            \forall i \in I.~
                            \pRes{w}\Big(P_i\{w/y_i\} \| \bignd_{j \in J} R_j\{w/z\}\Big) \vdash \Gamma, \Lambda, x{:}\ol{B}
                        }
                    }{
                        \forall i \in I.~
                        \pRes{x}\Big(Q_i \| \pRes{w}\Big(P_i\{w/y_i\} \| \bignd_{j \in J} R_j\{w/z\}\Big)\Big) \vdash \Gamma, \Delta, \Lambda
                    }
                }{
                    \bignd_{i \in I} \pRes{x}\Big(Q_i \| \pRes{w}\Big(P_i\{w/y_i\} \| \bignd_{j \in J} R_j\{w/z\}\Big)\Big) \vdash \Gamma, \Delta, \Lambda
                }
            \end{mathpar}

        \item
            This item depends on whether $x \in \fn{P_i}$ or not, for each $i \in I$.
            For simplicity, we only consider the cases where either $\forall i \in I.~ x \in \fn{P_i}$ or $\forall i \in I.~ x \notin \fn{P_i}$.
            \begin{itemize}
                \item
                    $\forall i \in I.~ x \in \fn{P_i}$.
                    \begin{mathpar}
                        \forall i \in I.~
                        \inferrule{
                            \inferrule{
                                P_i\{x'/x\} \vdash \Gamma, y_i{:}A, x'{:}{?}A
                            }{
                                \pCli* x[y_i];(P_i\{x'/x\}) \vdash \Gamma, x{:}{?}A, x'{:}{?}A
                            }
                        }{
                            \pCli* x[y_i];P_i \vdash \Gamma, x{:}{?}A
                        }
                        \and
                        \forall j \in J.~
                        \inferrule{
                            Q_j \vdash {?}\Delta, x{:}\ol{A}
                        }{
                            \pSrv x(z);Q_j \vdash {?}\Delta, x{:}{!}\ol{A}
                        }
                        \and\implies\and
                        \inferruleDbl{
                            \inferruleDbl{
                                \inferrule*[fraction={---}]{
                                    \inferrule*{
                                        \inferruleDbl{
                                            {\begin{tarr}[b]{l}
                                                    \forall i \in I.
                                                    \\
                                                    P_i\{w/y_i\} \vdash \Gamma, w{:}A, x{:}{?}A
                                            \end{tarr}}
                                        }{
                                            \bignd_{i \in I} P_i\{w/y_i\} \vdash \Gamma, w{:}A, x{:}{?}A
                                        }
                                        \\
                                        {\begin{tarr}[b]{l}
                                                \forall j \in J.
                                                \\
                                                Q_j\{w/z\}\{v'/v\}_{v \in {?}\Delta} \vdash {?}\Delta', w{:}\ol{A}
                                        \end{tarr}}
                                    }{
                                        {\begin{tarr}[t]{l}
                                                \forall j \in J.
                                                \\
                                                \pRes{w}\Big(\bignd_{i \in I} P_i\{w/y_i\} \| Q_j\{w/z\}\{v'/v\}_{v \in {?}\Delta}\Big) \vdash \Gamma, {?}\Delta', x{:}{?}A
                                        \end{tarr}}
                                    }
                                    \\
                                    {\begin{tarr}[b]{l}
                                            \forall j \in J.
                                            \\
                                            \pSrv x(z);Q_j \vdash {?}\Delta, x{:}{!}\ol{A}
                                    \end{tarr}}
                                }{
                                    \forall j \in J.~
                                    \pRes{x}\Big(\pRes{w}\Big(\bignd_{i \in I} P_i\{w/y_i\} \| Q_j\{w/z\}\{v'/v\}_{v \in {?}\Delta}\Big) \| \pSrv x(z);Q_j\Big) \vdash \Gamma, {?}\Delta, {?}\Delta'
                                }
                            }{
                                \bignd_{j \in J} \pRes{x}\Big(\pRes{w}\Big(\bignd_{i \in I} P_i\{w/y_i\} \| Q_j\{w/z\}\{v'/v\}_{v \in {?}\Delta}\Big) \| \pSrv x(z);Q_j\Big) \vdash \Gamma, {?}\Delta, {?}\Delta'
                            }
                        }{
                            \bignd_{j \in J} \pRes{x}\Big(\pRes{w}\Big(\bignd_{i \in I} P_i\{w/y_i\} \| Q_j\{w/z\}\Big) \| \pSrv x(z);Q_j\Big) \vdash \Gamma, {?}\Delta
                        }
                    \end{mathpar}

                \item
                    $\forall i \in I.~ x \notin \fn{P_i}$.
                    \begin{mathpar}
                        \forall i \in I.~
                        \inferrule{
                            P_i \vdash \Gamma, y_i{:}A
                        }{
                            \pCli* x[y_i];P_i \vdash \Gamma, x{:}{?}A
                        }
                        \and
                        \forall j \in J.~
                        \inferrule{
                            Q_j \vdash {?}\Delta, x{:}\ol{A}
                        }{
                            \pSrv x(z);Q_j \vdash {?}\Delta, x{:}{!}\ol{A}
                        }
                        \and\implies\and
                        \inferruleDbl{
                            \inferruleDbl{
                                \inferrule*[fraction={---}]{
                                    \inferrule*{
                                        \inferrule*{
                                            \inferruleDbl{
                                                {\begin{tarr}[b]{l}
                                                        \forall i \in I.
                                                        \\
                                                        P_i\{w/y_i\} \vdash \Gamma, w{:}A
                                                \end{tarr}}
                                            }{
                                                \bignd_{i \in I} P_i\{w/y_i\} \vdash \Gamma, w{:}A
                                            }
                                            \\
                                            {\begin{tarr}[b]{l}
                                                    \forall j \in J.
                                                    \\
                                                    Q_j\{w/z\}\{v'/v\}_{v \in {?}\Delta} \vdash {?}\Delta', w{:}\ol{A}
                                            \end{tarr}}
                                        }{
                                            {\begin{tarr}[t]{l}
                                                    \forall j \in J.
                                                    \\
                                                    \pRes{w}\Big(\bignd_{i \in I} P_i\{w/y_i\} \| Q_j\{w/z\}\{v'/v\}_{v \in {?}\Delta}\Big) \vdash \Gamma, {?}\Delta'
                                            \end{tarr}}
                                        }
                                    }{
                                        {\begin{tarr}[t]{l}
                                                \forall j \in J.
                                                \\
                                                \pRes{w}\Big(\bignd_{i \in I} P_i\{w/y_i\} \| Q_j\{w/z\}\{v'/v\}_{v \in {?}\Delta}\Big) \vdash \Gamma, {?}\Delta', x{:}{?}A
                                        \end{tarr}}
                                    }
                                    \\
                                    {\begin{tarr}[b]{l}
                                            \forall j \in J.
                                            \\
                                            \pSrv x(z);Q_j \vdash {?}\Delta, x{:}{!}\ol{A}
                                    \end{tarr}}
                                }{
                                    \forall j \in J.~
                                    \pRes{x}\Big(\pRes{w}\Big(\bignd_{i \in I} P_i\{w/y_i\} \| Q_j\{w/z\}\{v'/v\}_{v \in {?}\Delta}\Big) \| \pSrv x(z);Q_j\Big) \vdash \Gamma, {?}\Delta, {?}\Delta'
                                }
                            }{
                                \bignd_{j \in J} \pRes{x}\Big(\pRes{w}\Big(\bignd_{i \in I} P_i\{w/y_i\} \| Q_j\{w/z\}\{v'/v\}_{v \in {?}\Delta}\Big) \| \pSrv x(z);Q_j\Big) \vdash \Gamma, {?}\Delta, {?}\Delta'
                            }
                        }{
                            \bignd_{j \in J} \pRes{x}\Big(\pRes{w}\Big(\bignd_{i \in I} P_i\{w/y_i\} \| Q_j\{w/z\}\Big) \| \pSrv x(z);Q_j\Big) \vdash \Gamma, {?}\Delta
                        }
                    \end{mathpar}
                    \qedhere
            \end{itemize}
    \end{enumerate}
\end{proof}

\begin{theorem}[SR for the Lazy Semantics]\label{t:srTwo}
    If $P \vdash \Gamma$ and $P \redtwo_S Q$, then $Q \vdash \Gamma$.
\end{theorem}

\begin{proof}
    By induction on the derivation of the reduction.
    \begin{itemize}
        \item
            Rule $\rredtwo{\scc{Id}}$.
            \begin{mathpar}
                \inferrule{
                    \inferruleDbl{
                        \forall i \in I.~
                        \evalCtx[\big]{C_i}[\pFwd [x<>y]] \vdash \Gamma, x{:}A
                    }{
                        \bignd_{i \in I} \evalCtx[\big]{C_i}[\pFwd [x<>y]] \vdash \Gamma, x{:}A
                    }
                    \\
                    Q \vdash \Delta, x{:}\ol{A}
                }{
                    \pRes{x}\Big(\bignd_{i \in I} \evalCtx[\big]{C_i}[\pFwd [x<>y]] \| Q\Big) \vdash \Gamma, \Delta
                }
                \and\implies\and
                \inferruleDbl{
                    \forall i \in I.~
                    \evalCtx{C_i}[Q\{y/x\}] \vdash \Gamma, \Delta
                    ~~\text{(\refitem{l}{ctxRedOne}{Fwd})}
                }{
                    \bignd_{i \in I} \evalCtx{C_i}[Q\{y/x\}] \vdash \Gamma, \Delta
                }
            \end{mathpar}

        \item
            Rule $\rredtwo{\1\bot}$.
            \begin{mathpar}
                \inferrule{
                    \inferruleDbl{
                        \forall i \in I.~
                        \evalCtx{C_i}[\pClose x[]] \vdash \Gamma, x{:}\1
                        ~~\text{(\refitem{l}{ctxType}{Pclose})}
                    }{
                        \bignd_{i \in I} \evalCtx{C_i}[\pClose x[]] \vdash \Gamma, x{:}\1
                    }
                    \\
                    \inferruleDbl{
                        \forall j \in J.~
                        \evalCtx{D_j}[\pWait x();Q_j] \vdash \Delta, x{:}\bot
                        ~~\text{(\refitem{l}{ctxType}{Gclose})}
                    }{
                        \bignd_{j \in J} \evalCtx{D_j}[\pWait x();Q_j] \vdash \Delta, x{:}\bot
                    }
                }{
                    \pRes{x}\Big(\bignd_{i \in I} \evalCtx{C_i}[\pClose x[]] \| \bignd_{j \in J} \evalCtx{D_j}[\pWait x();Q_j]\Big) \vdash \Gamma, \Delta
                }
                \and\implies\and
                \inferrule{
                    \inferruleDbl{
                        \forall i \in I.~
                        \evalCtx{C_i}[\0] \vdash \Gamma
                        ~~\text{(\refitem{l}{ctxRedOne}{Pclose})}
                    }{
                        \bignd_{i \in I} \evalCtx{C_i}[\0] \vdash \Gamma
                    }
                    \\
                    \inferruleDbl{
                        \forall j \in J.~
                        \evalCtx{D_j}[Q_j] \vdash \Delta
                        ~~\text{(\refitem{l}{ctxRedOne}{Gclose})}
                    }{
                        \bignd_{j \in J} \evalCtx{D_j}[Q_j] \vdash \Delta
                    }
                }{
                    \bignd_{i \in I} \evalCtx{C_i}[\0] \| \bignd_{j \in J} \evalCtx{D_j}[Q_j] \vdash \Gamma, \Delta
                }
            \end{mathpar}

        \item
            Rule $\rredtwo{\tensor\parr}$.
            \begin{mathpar}
                \mprset{sep=0.8em}
                \inferrule{
                    \inferruleDbl{
                        \forall i \in I.~
                        \evalCtx{C_i}[\pOut* x[y_i];(P_i \| Q_i)] \vdash \Gamma, x{:}A \tensor B
                        ~~\text{(\refitem{l}{ctxType}{Pname})}
                    }{
                        \bignd_{i \in I} \evalCtx{C_i}[\pOut* x[y_i];(P_i \| Q_i)] \vdash \Gamma, x{:}A \tensor B
                    }
                    \\
                    \inferruleDbl{
                        \forall j \in J.~
                        \evalCtx{D_j}[\pIn x(z);R_j] \vdash \Delta, x{:}\ol{A} \parr \ol{B}
                        ~~\text{(\refitem{l}{ctxType}{Gname})}
                    }{
                        \bignd_{j \in J} \evalCtx{D_j}[\pIn x(z);R_j] \vdash \Delta, x{:}\ol{A} \parr \ol{B}
                    }
                }{
                    \pRes{x}\Big(\bignd_{i \in I} \evalCtx{C_i}[\pOut* x[y_i];(P_i \| Q_i)] \| \bignd_{j \in J} \evalCtx{D_j}[\pIn x(z);R_j]\Big) \vdash \Gamma, \Delta
                }
                \and\implies\and
                \inferrule{}{
                    \bignd_{i \in I} \evalCtx[\Big]{C_i}[\pRes{x}\Big(Q_i \| \pRes{w}\Big(P_i\{w/y_i\} \| \bignd_{j \in J} \evalCtx{D_j}[R_j\{w/z\}]\Big)\Big)] \vdash \Gamma, \Delta
                    ~~\text{(\refitem{l}{ctxRedTwo}{Name})}
                }
            \end{mathpar}

        \item
            Rule $\rredtwo{{\oplus}{\\&}}$.
            Take any $k' \in K$.
            \begin{mathpar}
                \inferrule{
                    \inferruleDbl{
                        {\begin{tarr}[b]{l}
                                \forall i \in I.
                                \\
                                \evalCtx{C_i}[\pSel* x < k';P_i] \vdash \Gamma, x{:}{\oplus}\{k:A_k\}_{k \in K}
                                \\
                                \text{(\refitem{l}{ctxType}{Psel})}
                        \end{tarr}}
                    }{
                        \bignd_{i \in I} \evalCtx{C_i}[\pSel* x < k';P_i] \vdash \Gamma, x{:}{\oplus}\{k:A_k\}_{k \in K}
                    }
                    \\
                    \inferruleDbl{
                        {\begin{tarr}[b]{l}
                                \forall j \in J.
                                \\
                                \evalCtx{D_j}[\pBra* x > \{k:Q_j^k\}_{k \in K}] \vdash \Delta, x{:}{\\&}\{k:\ol{A_k}\}_{k \in K}
                                \\
                                \text{(\refitem{l}{ctxType}{Gsel})}
                        \end{tarr}}
                    }{
                        \bignd_{j \in J} \evalCtx{D_j}[\pBra* x > \{k:Q_j^k\}_{k \in K}] \vdash \Delta, x{:}{\\&}\{k:\ol{A_k}\}_{k \in K}
                    }
                }{
                    \pRes{x}\Big(\bignd_{i \in I} \evalCtx{C_i}[\pSel* x < k';P_i] \| \bignd_{j \in J} \evalCtx{D_j}[\pBra* x > \{k:Q_j^k\}_{k \in K}]\Big) \vdash \Gamma, \Delta
                }
                \and\implies\and
                \inferrule{
                    \inferruleDbl{
                        \forall i \in I.~
                        \evalCtx{C_i}[P_i] \vdash \Gamma, x{:}A
                        ~~\text{(\refitem{l}{ctxRedOne}{Psel})}
                    }{
                        \bignd_{i \in I} \evalCtx{C_i}[P_i] \vdash \Gamma, x{:}A
                    }
                    \\
                    \inferruleDbl{
                        \forall j \in J.~
                        \evalCtx{D_j}[Q_j^k] \vdash \Delta, x{:}\ol{A}
                        ~~\text{(\refitem{l}{ctxRedOne}{Gsel})}
                    }{
                        \bignd_{j \in J} \evalCtx{D_j}[Q_j^k] \vdash \Delta, x{:}\ol{A}
                    }
                }{
                    \pRes{x}\Big(\bignd_{i \in I} \evalCtx{C_i}[P_i] \| \bignd_{j \in J} \evalCtx{D_j}[Q_j^k]\Big) \vdash \Gamma, \Delta
                }
            \end{mathpar}

        \item
            Rule $\rredtwo{\some}$.
            \begin{mathpar}
                %\mprset{sep=0.5em}
                \inferrule{
                    \inferruleDbl{
                        {\begin{tarr}[b]{l}
                                \forall i \in I.
                                \\
                                \evalCtx{C_i}[\pSome x;P_i] \vdash \Gamma, x{:}{\\&}A
                                \\
                                \text{(\refitem{l}{ctxType}{Psome})}
                        \end{tarr}}
                    }{
                        \bignd_{i \in I} \evalCtx{C_i}[\pSome x;P_i] \vdash \Gamma, x{:}{\\&}A
                    }
                    \\
                    \inferruleDbl{
                        {\begin{tarr}[b]{l}
                                \forall j \in J.
                                \\
                                \evalCtx{D_j}[\pSomeIn x{w_1,\ldots,w_n};Q_j] \vdash \Delta, x{:}{\oplus}\ol{A}
                                \\
                                \text{(\refitem{l}{ctxType}{Gsome})}
                        \end{tarr}}
                    }{
                        \bignd_{j \in J} \evalCtx{D_j}[\pSomeIn x{w_1,\ldots,w_n};Q_j] \vdash \Delta, x{:}{\oplus}\ol{A}
                    }
                }{
                    \pRes{x}\Big( \bignd_{i \in I} \evalCtx{C_i}[\pSome x;P_i] \| \bignd_{j \in J} \evalCtx{D_j}[\pSomeIn x{w_1,\ldots,w_n};Q_j]\Big) \vdash \Gamma, \Delta
                }
                \and\implies\and
                \inferrule{
                    \inferruleDbl{
                        \forall i \in I.~
                        \evalCtx{C_i}[P_i] \vdash \Gamma, x{:}A
                        ~~\text{(\refitem{l}{ctxRedOne}{Psome})}
                    }{
                        \bignd_{i \in I} \evalCtx{C_i}[P_i] \vdash \Gamma, x{:}A
                    }
                    \\
                    \inferruleDbl{
                        \forall j \in J.~
                        \evalCtx{D_j}[Q_j] \vdash \Delta, x{:}\ol{A}
                        ~~\text{(\refitem{l}{ctxRedOne}{Gsome})}
                    }{
                        \bignd_{j \in J} \evalCtx{D_j}[Q_j] \vdash \Delta, x{:}\ol{A}
                    }
                }{
                    \pRes{x}\Big(\bignd_{i \in I} \evalCtx{C_i}[P_i] \| \bignd_{j \in J} \evalCtx{D_j}[Q_j]\Big) \vdash \Gamma, \Delta
                }
            \end{mathpar}

        \item
            Rule $\rredtwo{\none}$.
            \begin{mathpar}
                %\mprset{sep=0.5em}
                \inferrule{
                    \inferruleDbl{
                        {\begin{tarr}[b]{l}
                                \forall i \in I.
                                \\
                                \evalCtx{C_i}[\pNone x] \vdash \Gamma, x{:}{\\&}A
                                \\
                                \text{(\refitem{l}{ctxType}{Pnone})}
                        \end{tarr}}
                    }{
                        \bignd_{i \in I} \evalCtx{C_i}[\pNone x] \vdash \Gamma, x{:}{\\&}A
                    }
                    \\
                    \inferruleDbl{
                        {\begin{tarr}[b]{l}
                                \forall j \in J.
                                \\
                                \evalCtx{D_j}[\pSomeIn x{w_1,\ldots,w_n};Q_j] \vdash \Delta, x{:}{\oplus}\ol{A}
                                \\
                                \text{(\refitem{l}{ctxType}{Gsome})}
                        \end{tarr}}
                    }{
                        \bignd_{j \in J} \evalCtx{D_j}[\pSomeIn x{w_1,\ldots,w_n};Q_j] \vdash \Delta, x{:}{\oplus}\ol{A}
                    }
                }{
                    \pRes{x}\Big( \bignd_{i \in I} \evalCtx{C_i}[\pNone x] \| \bignd_{j \in J} \evalCtx{D_j}[\pSomeIn x{w_1,\ldots,w_n};Q_j]\Big) \vdash \Gamma, \Delta
                }
                \and\implies\and
                \inferrule{
                    \inferruleDbl{
                        \forall i \in I.~
                        \evalCtx{C_i}[\0] \vdash \Gamma
                        ~~\text{(\refitem{l}{ctxRedOne}{Pnone})}
                    }{
                        \bignd_{i \in I} \evalCtx{C_i}[P_i] \vdash \Gamma
                    }
                    \\
                    \inferruleDbl{
                        \forall j \in J.~
                        \evalCtx{D_j}[\pNone w_1 \| \ldots \| \pNone w_n] \vdash \Delta
                        ~~\text{(\refitem{l}{ctxRedOne}{Gsome})}
                    }{
                        \bignd_{j \in J} \evalCtx{D_j}[\pNone w_1 \| \ldots \| \pNone w_n] \vdash \Delta
                    }
                }{
                    \bignd_{i \in I} \evalCtx{C_i}[\0] \| \bignd_{j \in J} \evalCtx{D_j}[\pNone w_1 \| \ldots \| \pNone w_n] \vdash \Gamma, \Delta
                }
            \end{mathpar}

        \item
            Rule $\rredtwo{{?}{!}}$.
            \begin{mathpar}
                \inferrule{
                    \inferruleDbl{
                        \forall i \in I.~
                        \evalCtx{C_i}[\pCli* x[y_i];P_i] \vdash \Gamma, x{:}{?}A
                        ~~\text{(\refitem{l}{ctxType}{Puname})}
                    }{
                        \bignd_{i \in I} \evalCtx{C_i}[\pCli* x[y_i];P_i] \vdash \Gamma, x{:}{?}A
                    }
                    \\
                    \inferruleDbl{
                        \forall j \in J.~
                        \evalCtx{D_j}[\pSrv x(z);Q_j] \vdash \Delta, x{:}{!}\ol{A}
                        ~~\text{(\refitem{l}{ctxType}{Guname})}
                    }{
                        \bignd_{j \in J} \evalCtx{D_j}[\pSrv x(z);Q_j] \vdash \Delta, x{:}{!}\ol{A}
                    }
                }{
                    \pRes{x}\Big(\bignd_{i \in I} \evalCtx{C_i}[\pCli* x[y_i];P_i] \| \bignd_{j \in J} \evalCtx{D_j}[\pSrv x(z);Q_j]\Big) \vdash \Gamma, \Delta
                }
                \and\implies\and
                \inferrule{}{
                    \bignd_{j \in J} \evalCtx[\Big]{D_j}[\pRes{x}\Big(\pRes{w}\Big(\bignd_{i \in I} \evalCtx{C_i}[P_i\{w/z\}] \| Q_j\{w/z\}\Big) \| \pSrv x(z);Q_j\Big)] \vdash \Gamma, \Delta
                    ~~\text{(\refitem{l}{ctxRedTwo}{Uname})}
                }
            \end{mathpar}
            \qedhere
    \end{itemize}
\end{proof}

\subsubsection{Deadlock Freedom}
\label{ss:DFLazy}

\begin{definition}[Multi-hole Non-deterministic Reduction Contexts]
    \begin{align*}
        \evalCtx{M} ::= \hole \sepr \pRes{x}(P \| \evalCtx{M}) \sepr P \| \evalCtx{M} \sepr \evalCtx{M} \nd \evalCtx{M}
    \end{align*}
\end{definition}

\begin{lemma}\label{l:ndCtxMultihole}
    If $\evalCtx{N}[\alpha;P] \vdash \Gamma, x{:}A$ and $x = \subjs(\alpha)$, then there are $\evalCtx{M}$ and ${(\alpha_i;P_i)}_{i \in I}$ such that $\evalCtx{N}[\alpha;P] = \evalCtx{M}[\alpha_i;P_i]_{i \in I}$ where $x \notin \fn{\evalCtx{M}}$ and $x \in \bigcap_{i \in I} \fn{\alpha_i;P_i}$ and there is $i' \in I$ such that $\alpha_{i'};P_{i'} = \alpha;P$.
\end{lemma}

\begin{lemma}\label{l:multiNdDet}
    For every multi-hole ND-context $\evalCtx{M}$ with indices $I$:
    \begin{itemize}
        \item
            If $\evalCtx{M}$ has two or more holes, there are $\evalCtx{C}$, $\evalCtx{M_1}$ with indices $I_1$, $\evalCtx{M_2}$ with indices $I_2$ such that $\evalCtx{M} = \evalCtx{C}[\evalCtx{M_1} \nd \evalCtx{M_2}]$ where $I_1 \cap I_2 = \emptyset$ and $I = I_1 \cup I_2$.

        \item
            If $\evalCtx{M}$ has only one hole, there is $\evalCtx{C}$ such that $\evalCtx{M} = \evalCtx{C}$.
    \end{itemize}
\end{lemma}

\begin{definition}\label{d:ndFlat}
    \begin{align*}
        \flat{\evalCtx{C}[\evalCtx{M} \nd \evalCtx{M'}]}
        &\deq \flat{\evalCtx{C}[\evalCtx{M}]} \nd \flat{\evalCtx{C}[\evalCtx{M'}]}
        &
        \flat{\evalCtx{C}}
        &\deq \evalCtx{C}
    \end{align*}
\end{definition}

\begin{lemma}\label{l:multiShape}
    If $\evalCtx{M}[P_i]_{i \in I} \vdash \Gamma$ where $x \notin \fn{\evalCtx{M}}$ and $\forall i \in I.~ x \in \fn{P_i}$, then there are ${(\evalCtx{C_i})}_{i \in I}$ such that $\flat{\evalCtx{M}}[P_i]_{i \in I} = \bignd_{i \in I} \evalCtx{C_i}[P_i]$ where $\forall i \in I.~ x \notin \fn{\evalCtx{C_i}}$.
\end{lemma}

\begin{lemma}\label{l:flatRed}
    If
    \begin{align*}
        \pRes{x}(\evalCtx[\big]{N}[\flat{\evalCtx{M}}[\alpha_i;P_i]_{i \in I}] \| \evalCtx[\big]{N'}[\flat{\evalCtx{M'}}[\beta_j;Q_j]_{j \in J}]) \redtwo_S R,
    \end{align*}
    then
    \begin{align*}
    \pRes{x}(\evalCtx[\big]{N}[\evalCtx{M}[\alpha_i;P_i]_{i \in I}] \| \evalCtx[\big]{N'}[\evalCtx{M'}[\beta_j;Q_j]_{j \in J}]) \redtwo_S R.
    \end{align*}
\end{lemma}

\begin{proof}
    By induction on the structures of $\evalCtx{M}$ and $\evalCtx{M'}$.
    By \Cref{l:multiNdDet}, we only have to consider two cases for $\evalCtx{M}$ ($\evalCtx{M} = \evalCtx{C}[\evalCtx{M_1} \nd \evalCtx{M_2}]$ and $\evalCtx{M} = \evalCtx{C}$), and similarly for $\evalCtx{M'}$.
    We only detail the base case ($\evalCtx{M} = \evalCtx{C}$ and $\evalCtx{M'} = \evalCtx{C'}$) and a representative inductive case ($\evalCtx{M} = \evalCtx{C}[\evalCtx{M_1} \nd \evalCtx{M_2}]$ and $\evalCtx{M'} = \evalCtx{C'}$).
    \begin{itemize}
        \item
            $\evalCtx{M} = \evalCtx{C}$ and $\evalCtx{M'} = \evalCtx{C'}$.
            Note that $\evalCtx{M}$ and $\evalCtx{M'}$ have only one hole; w.l.o.g., assume $I = J = \{1\}$.
            \begin{align*}
                \flat{\evalCtx{M}}[\alpha_1;P_1] &= \flat{\evalCtx{C}}[\alpha_1;P_1] = \evalCtx{C}[\alpha_1;P_1] = \evalCtx{M}[\alpha_1;P_1]
                \\
                \flat{\evalCtx{M'}}[\beta_1;Q_1] &= \flat{\evalCtx{C'}}[\beta_1;Q_1] = \evalCtx{C'}[\beta_1;Q_1] = \evalCtx{M'}[\beta_1;Q_1]
            \end{align*}
            The thesis follows by assumption and equality.

        \item
            $\evalCtx{M} = \evalCtx{C}[\evalCtx{M_1} \nd \evalCtx{M_2}]$ and $\evalCtx{M'} = \evalCtx{C'}$.
            Note that $\evalCtx{M'}$ has only one hole; w.l.o.g., assume $J = \{1\}$.
            \begin{align}
                & \pRes{x}(\evalCtx[\big]{N}[\flat{\evalCtx{M}}[\alpha_i;P_i]_{i \in I}] \| \evalCtx[\big]{N'}[\flat{\evalCtx{M'}}[\beta_1;Q_1]])
                \nonumber
                \\
                &= \pRes{x}(\evalCtx[\big]{N}[\flat{\evalCtx{C}[\evalCtx{M_1} \nd \evalCtx{M_2}]}[\alpha_i;P_i]_{i \in I}] \| \evalCtx[\big]{N'}[\flat{\evalCtx{C'}}[\beta_1;Q_1]])
                \nonumber
                \\
                &= \pRes{x}(\evalCtx[\big]{N}[(\flat{\evalCtx{C}[\evalCtx{M_1}]} \nd \flat{\evalCtx{C}[\evalCtx{M_2}]})[\alpha_i;P_i]_{i \in I}] \| \evalCtx[\big]{N'}[\evalCtx{C'}[\beta_1;Q_1]])
                \label{eq:oneImplTwoBeforeSplit}
            \end{align}
            There are $I_1$ and $I_2$ such that $I_1 \cap I_2 = \emptyset$ and $I = I_1 \cup I_2$ and
            \begin{align}
                & \pRes{x}(\evalCtx[\big]{N}[\flat{\evalCtx{M}}[\alpha_i;P_i]_{i \in I}] \| \evalCtx[\big]{N'}[\flat{\evalCtx{M'}}[\beta_1;Q_1]])
                \nonumber
                \\
                &= \pRes{x}(\evalCtx[\big]{N}[\flat{\evalCtx{C}[\evalCtx{M_1}]}[\alpha_i;P_i]_{i \in I_1} \nd \flat{\evalCtx{C}[\evalCtx{M_2}]}[\alpha_i;P_i]_{i \in I_2}] \| \evalCtx[\big]{N'}[\evalCtx{C'}[\beta_1;Q_1]]).
                &&\text{(by~\eqref{eq:oneImplTwoBeforeSplit})}
                \label{eq:oneImplTwoAfterSplit}
            \end{align}
            Let $\evalCtx{N_1} = \evalCtx[\big]{N}[\hole \nd \flat{\evalCtx{C}[\evalCtx{M_2}]}[\alpha_i;P_i]_{i \in I_2}]$.
            \begin{align}
                & \pRes{x}(\evalCtx[\big]{N}[\flat{\evalCtx{M}}[\alpha_i;P_i]_{i \in I}] \| \evalCtx[\big]{N'}[\flat{\evalCtx{M'}}[\beta_1;Q_1]])
                \nonumber
                \\
                &= \pRes{x}(\evalCtx[\big]{N_1}[\flat{\evalCtx{C}[\evalCtx{M_1}]}[\alpha_i;P_i]_{i \in I_1}] \| \evalCtx[\big]{N'}[\evalCtx{C'}[\beta_1;Q_1]])
                &&\text{(by~\eqref{eq:oneImplTwoAfterSplit})}
                \nonumber
                \\
                &\redtwo_S R
                &&\text{(by assumption)}
                \label{eq:oneImplTwoLeftRed}
                \\
                & \pRes{x}(\evalCtx[\big]{N_1}[\evalCtx{C}[\evalCtx{M_1}][\alpha_i;P_i]_{i \in I_1}] \| \evalCtx[\big]{N'}[\evalCtx{C'}[\beta_1;Q_1]])
                \nonumber
                \\
                &= \pRes{x}(\evalCtx[\big]{N}[\evalCtx{C}[\evalCtx{M_1}][\alpha_i;P_i]_{i \in I_1} \nd \flat{\evalCtx{C}[\evalCtx{M_2}]}[\alpha_i;P_i]_{i \in I_2}] \| \evalCtx[\big]{N'}[\evalCtx{C'}[\beta_1;Q_1]])
                \nonumber
                \\
                &\redtwo_S R
                &&\text{(by IH on~\eqref{eq:oneImplTwoLeftRed})}
                \label{eq:oneImplTwoBeforeRightRed}
            \end{align}
        Let $\evalCtx{N_2} = \evalCtx[\big]{N}[\evalCtx{C}[\evalCtx{M_1}][\alpha_i;P_i]_{i \in I_1} \nd \hole]$.
            \begin{align}
                & \pRes{x}(\evalCtx[\big]{N}[\evalCtx{C}[\evalCtx{M_1}][\alpha_i;P_i]_{i \in I_1} \nd \flat{\evalCtx{C}[\evalCtx{M_2}]}[\alpha_i;P_i]_{i \in I_2}] \| \evalCtx[\big]{N'}[\evalCtx{C'}[\beta_1;Q_1]])
                \nonumber
                \\
                &= \pRes{x}(\evalCtx[\big]{N_2}[\flat{\evalCtx{C}[\evalCtx{M_2}]}[\alpha_i;P_i]_{i \in I_2}] \| \evalCtx[\big]{N'}[\evalCtx{C'}[\beta_1;Q_1]])
                \nonumber
                \\
                &\redtwo_S R
                &&\text{(by~\eqref{eq:oneImplTwoBeforeRightRed})}
                \label{eq:oneImplTwoRightRed}
                \\
                & \pRes{x}(\evalCtx[\big]{N_2}[\evalCtx{C}[\evalCtx{M_2}][\alpha_i;P_i]_{i \in I_2}] \| \evalCtx[\big]{N'}[\evalCtx{C'}[\beta_1;Q_1]])
                \nonumber
                \\
                &= \pRes{x}(\evalCtx[\big]{N}[\evalCtx{C}[\evalCtx{M_1}][\alpha_i;P_i]_{i \in I_1} \nd \evalCtx{C}[\evalCtx{M_2}][\alpha_i;P_i]_{i \in I_2}] \| \evalCtx[\big]{N'}[\evalCtx{C'}[\beta_1;Q_1]])
                \nonumber
                \\
                &= \pRes{x}(\evalCtx[\Big]{N}[\evalCtx[\big]{C}[\evalCtx{M_1}[\alpha_i;P_i]_{i \in I_1}] \nd \evalCtx[\big]{C}[\evalCtx{M_2}[\alpha_i;P_i]_{i \in I_2}]] \| \evalCtx[\big]{N'}[\evalCtx{C'}[\beta_1;Q_1]])
                \nonumber
                \\
                &\redtwo_S R
                &&\text{(by IH on~\eqref{eq:oneImplTwoRightRed})}
                \label{eq:oneImplTwoIHRed}
                \\
                & \pRes{x}(\evalCtx[\Big]{N}[\evalCtx[\big]{C}[\evalCtx{M_1}[\alpha_i;P_i]_{i \in I_1} \nd \evalCtx{M_2}[\alpha_i;P_i]_{i \in I_2}]] \| \evalCtx[\big]{N'}[\evalCtx{C'}[\beta_1;Q_1]])
                \nonumber
                \\
                &= \pRes{x}(\evalCtx[\Big]{N}[\evalCtx[\big]{C}[(\evalCtx{M_1} \nd \evalCtx{M_2})[\alpha_i;P_i]_{i \in I}]] \| \evalCtx[\big]{N'}[\evalCtx{C'}[\beta_1;Q_1]])
                \nonumber
                \\
                &= \pRes{x}(\evalCtx[\big]{N}[\evalCtx{C}[\evalCtx{M_1} \nd \evalCtx{M_2}][\alpha_i;P_i]_{i \in I}] \| \evalCtx[\big]{N'}[\evalCtx{C'}[\beta_1;Q_1]])
                \nonumber
                \\
                &= \pRes{x}(\evalCtx[\big]{N}[\evalCtx{M}[\alpha_i;P_i]_{i \in I}] \| \evalCtx[\big]{N'}[\evalCtx{M'}[\beta_1;Q_1]])
                \nonumber
                \\
                &\redtwo_S R
                &&\text{(by rule $\rredtwo{\nu\nd}$ on~\eqref{eq:oneImplTwoIHRed})}
                \nonumber
                \tag*{\qedhere}
            \end{align}
    \end{itemize}
\end{proof}

\begin{theorem}\label{t:oneImpliesTwo}
    If $P \vdash \Gamma$ and $P \reddEager R$, then $P \redtwo_S R'$.
\end{theorem}

\begin{proof}
    By induction on the derivation of the reduction.
    The inductive cases of rules $\rredone{\equiv}$, $\rredone{\nu}$, $\rredone{\|}$, and $\rredone{\nd}$ follow from the IH straightforwardly, using the corresponding closure rule for $\redtwo$.
    As representative base case, we consider rule $\rredone{\1\bot}$: $P = \pRes{x}(\evalCtx{N}[\pClose x[]] \| \evalCtx{N'}[\pWait x();Q]) \reddEager R$.

    By inversion of typing, $\evalCtx{N}[\pClose x[]] \vdash \Gamma, x{:}A$, so by \Cref{l:ndCtxMultihole}, there are $\evalCtx{M}$ and ${(\alpha_i;P_i)}_{i \in I}$ such that $\evalCtx{N}[\pClose x[]] = \evalCtx{M}[\alpha_i;P_i]_{i \in I}$ where $x \notin \fn{\evalCtx{M}}$ and $x \in \bigcap_{i \in I} \fn{\alpha_i;P_i}$ and there is $i' \in I$ such that $\alpha_{i'};P_{i'} = \pClose x[]$.
    Similarly, there are $\evalCtx{M'}$ and ${(\beta_j;Q_j)}_{j \in J}$ such that $\evalCtx{N'}[\pWait x();Q] = \evalCtx{M'}[\beta_j;Q_j]_{j \in J}$ where $x \notin \fn{\evalCtx{M'}}$ and $x \in \bigcap_{j \in J} \fn{\beta_j;Q_j}$ and there is $j' \in J$ such that $\beta_{j'};Q_{j'} = \pWait x();Q$.

    By \Cref{l:multiShape}, $\flat{\evalCtx{M}}[\alpha_i;P_i]_{i \in I} = \bignd_{i \in I} \evalCtx{C_i}[\alpha_i;P_i]$ and $\flat{\evalCtx{M'}}[\beta_j;Q_j]_{j \in J} = \bignd_{j \in J} \evalCtx{C'_j}[\beta_j;Q_j]$.
    By typability, there is $I' \subseteq I$ such that $\forall i \in I'.~ \alpha_i \relalpha \pClose x[]$ and $\forall i \in I \setminus I'.~ \alpha_i \not\relalpha \pClose x[]$; hence, $i' \in I'$.
    Similarly, there is $J' \subseteq J$ such that $\forall j \in J'.~ \beta_j \relalpha \pWait x()$ and $\forall j \in J \setminus J'.~ \beta_j \not\relalpha \pWait x()$; hence, $j' \in J'$.
    Then, by \Cref{d:rpreone}, $\flat{\evalCtx{M}}[\alpha_i;P_i]_{i \in I} \piprecong{x} \bignd_{i \in I'} \evalCtx{C_i}[\pClose x[]]$ and $\flat{\evalCtx{M'}}[\beta_j;Q_j]_{j \in J} \piprecong{x} \bignd_{j \in J'} \evalCtx{C_j}[\pWait x();Q_j]$.
    By rule $\rredtwo{\1\bot}$,
    \begin{align*}
        \pRes{x}(\bignd_{i \in I'} \evalCtx{C_i}[\pClose x[]] \| \bignd_{j \in J'} \evalCtx{C_j}[\pWait x();Q_j]) &\redtwo_x R,
    \end{align*}
    so by rule $\rredtwo{\piprecong{x}}$,
    \begin{align*}
        \pRes{x}(\flat{\evalCtx{M}}[\alpha_i;P_i]_{i \in I} \| \flat{\evalCtx{M'}}[\beta_j;Q_j]_{j \in J}) \redtwo_x R.
    \end{align*}
    Then, by \Cref{l:flatRed},
    \begin{align*}
        \pRes{x}(\evalCtx{M}[\alpha_i;P_i]_{i \in I} \| \evalCtx{M'}[\beta_j;Q_j]_{j \in J}) \redtwo_x R.
    \end{align*}

    A second base case, we consider rule $\rredone{\scc{Id}}$: $P = \pRes{x}(\evalCtx[\big]{N}[\pFwd [x<>y]] \| Q) \reddEager R$.

    By inversion of typing, $ \evalCtx[\big]{N}[\pFwd [x<>y]]  \vdash \Gamma, x{:}A, y{:}\dual{A}$, so by \Cref{l:ndCtxMultihole}, there are $\evalCtx{M}$ and ${(\alpha_i;P_i)}_{i \in I}$ such that $\evalCtx[\big]{N}[\pFwd [x<>y]]  = \evalCtx{M}[\alpha_i;P_i]_{i \in I}$ where $x \notin \fn{\evalCtx{M}}$ and $x \in \bigcap_{i \in I} \fn{\alpha_i;P_i}$ and there is $i' \in I$ such that $\alpha_{i'};P_{i'} = \pFwd [x<>y] $.

    By \Cref{l:multiShape}, $\flat{\evalCtx{M}}[\alpha_i;P_i]_{i \in I} = \bignd_{i \in I} \evalCtx{C_i}[\alpha_i;P_i]$.
    By typability, there is $I' \subseteq I$ such that $\forall i \in I'.~ \alpha_i = \pFwd [x<>y]$ and $\forall i \in I \setminus I'.~ \alpha_i \not= \pFwd [x<>y]$; hence, $i' \in I'$.

    Then, by \Cref{d:rpreone}, $\flat{\evalCtx{M}}[\alpha_i;P_i]_{i \in I} \piprecong{x,y} \bignd_{i \in I'} \evalCtx{C_i}[\pFwd [x<>y]]$.
    By rule $\rredtwo{\scc{Id}}$,
    \begin{align*}
        \pRes{x} \Big( \bignd_{i \in I}\evalCtx[\big]{C_i}[\pFwd [x<>y]] \| Q\Big)
                \redtwo_{x,y}
                 R,
    \end{align*}
    so by rule $\rredtwo{\piprecong{x,y}}$,
    \begin{align*}
        \pRes{x}(\flat{\evalCtx{M}}[\alpha_i;P_i]_{i \in I} \| Q ) \redtwo_{x,y} R.
    \end{align*}
    Then, by \Cref{l:flatRed},
    \begin{align*}
        \pRes{x}(\evalCtx{M}[\alpha_i;P_i]_{i \in I} \| Q ) \redtwo_{x,y} R.
        \tag*{\qedhere}
    \end{align*}
\end{proof}

\begin{theorem}[DF: Lazy Semantics]\label{t:dlfreeTwo}
    If $P \vdash \emptyset$ and $P \not\equiv \0$, then $P \redtwo_S R$ for some $S$ and $R$.
\end{theorem}

\begin{proof}
    As a corollary of \Cref{t:dlfreeOne,t:oneImpliesTwo}.
\end{proof}
